# Supplementary material for: Six-loop beta functions in general scalar theory
Source: arXiv:2102.12832 ancillary file (2021-04-26)
Supplement: Supplementary file 1 [file RG6_results_ctb.pdf]

The beta functions for the parameters for the Lagrangian

$$\mathcal{L} = \frac{1}{2} \partial_\mu \phi_a \partial_\mu \phi_a - \frac{m_{ab}^2}{2} \phi_a \phi_b - \frac{h_{abc}}{3!} \phi_a \phi_b \phi_c - \frac{\lambda_{abcd}}{4!} \phi_a \phi_b \phi_c \phi_d - t_a \phi_a - \Lambda \quad (1)$$

are given by

$$\begin{aligned} \beta_{\lambda_{abcd}} \equiv \beta_{abcd} &= \left[ \lambda_{abcf} \gamma_{fd}^\phi + \lambda_{abdf} \gamma_{fc}^\phi + \lambda_{acdf} \gamma_{fb}^\phi + \lambda_{bcdf} \gamma_{fa}^\phi \right] + [\lambda_{abef} \lambda_{cdgh} \bigcirc_{ef|gh} + 5 \text{ perm.}] \\ &+ [\lambda_{abef} \lambda_{cg hi} \lambda_{djkl} \triangle_{ef|ghi|jkl} + 11 \text{ perm.}] \\ &+ [\lambda_{aefg} \lambda_{bhij} \lambda_{cklm} \lambda_{dnop} \square_{efg|hij|klm|nop} + 23 \text{ perm.}] \end{aligned} \quad (2)$$

$$\begin{aligned} \beta_{h_{abc}} \equiv \beta_{abc} &= \left[ h_{abf} \gamma_{fc}^\phi + h_{acf} \gamma_{fb}^\phi + h_{bcf} \gamma_{fa}^\phi \right] + [\lambda_{abef} h_{cgh} (\bigcirc_{ef|gh} + \bigcirc_{gh|ef}) + 2 \text{ perm.}] \\ &+ [\lambda_{abef} \lambda_{cg hi} h_{jkl} (\triangle_{ef|ghi|jkl} + \triangle_{ef|jkl|ghi}) + 2 \text{ perm.}] \\ &+ [h_{aef} \lambda_{bg hi} \lambda_{cjkl} \triangle_{ef|ghi|jkl} + 5 \text{ perm.}] + [\lambda_{aefg} \lambda_{bhij} \lambda_{cklm} h_{nop} (\square_{efg|hij|klm|nop} \\ &+ \square_{nop|efg|hij|klm} + \square_{klm|nop|efg|hij} + \square_{hij|klm|nop|efg}) + 5 \text{ perm.}] \end{aligned} \quad (3)$$

$$\begin{aligned} \beta_{m_{ab}^2} \equiv \beta_{ab} &= \left[ m_{af}^2 \gamma_{fb}^\phi + m_{bf}^2 \gamma_{fa}^\phi \right] + [(\lambda_{abef} m_{gh}^2 + h_{aef} h_{bgh}) (\bigcirc_{ef|gh} + \bigcirc_{gh|ef})] \\ &+ [\lambda_{abef} h_{g hi} h_{jkl} \triangle_{ef|ghi|jkl} + m_{ef}^2 \lambda_{ag hi} \lambda_{bjkl} (\triangle_{ef|ghi|jkl} + \triangle_{ef|jkl|ghi})] \\ &+ [h_{aef} h_{g hi} \lambda_{bjkl} (\triangle_{ef|ghi|jkl} + \triangle_{ef|jkl|ghi}) + (a \leftrightarrow b)] \\ &+ [\lambda_{aefg} \lambda_{bhij} h_{klm} h_{nop} (\square_{efg|hij|klm|nop} + \square_{efg|klm|hij|nop} + \square_{efg|klm|nop|hij} \\ &+ \square_{klm|efg|hij|nop} + \square_{klm|efg|nop|hij} + \square_{klm|nop|efg|hij}) + (a \leftrightarrow b)] . \end{aligned} \quad (4)$$

$$\begin{aligned} \beta_{t_a} \equiv \beta_a &= t_f \gamma_{fb}^\phi + h_{aef} m_{gh}^2 [\bigcirc_{ef|gh} + \bigcirc_{gh|ef}] \\ &+ [h_{aef} h_{g hi} h_{jkl} \triangle_{ef|ghi|jkl} + m_{ef}^2 \lambda_{ag hi} h_{bjkl} (\triangle_{ef|ghi|jkl} + \triangle_{ef|jkl|ghi})] \\ &+ \lambda_{aefg} h_{hij} h_{klm} h_{nop} [\square_{efg|hij|klm|nop} + \square_{nop|efg|hij|klm} \\ &+ \square_{klm|nop|efg|hij} + \square_{hij|klm|nop|efg}] . \end{aligned} \quad (5)$$

$$\beta_\Lambda = m_{ef}^2 m_{gh}^2 \bigcirc_{ef|gh} + m_{ef}^2 h_{g hi} h_{jkl} \triangle_{ef|ghi|jkl} + h_{efg} h_{hij} h_{klm} h_{nop} \square_{efg|hij|klm|nop} . \quad (6)$$

In what follows we present loop expansion of the “circle”, “triangle”, and “box” structures:

$$\bigcirc_{ab|cd} = \sum_{l=1}^6 \bigcirc_{ab|cd}^{(l)} , \quad (7)$$

$$\triangle_{ab|cde|fgh} = \sum_{l=1}^6 \triangle^{(l)}_{ab|cde|fgh} , \quad (8)$$

$$\square_{abc|def|ghi|jkl} = \sum_{l=1}^6 \square^{(l)}_{abc|def|ghi|jkl} . \quad (9)$$

$$\bigcirc_{ab|cd}^{(1)} = \delta_{ac} \delta_{bd} \left( \frac{1}{2} \right) \quad (10)$$

$$\begin{aligned} \bigcirc_{ab|cd}^{(3)} &= \lambda_{c\alpha\beta a} \lambda_{d\alpha\beta b} \left( \frac{1}{4} \right) \\ &+ \delta_{bd} \lambda_{\alpha\beta\gamma a} \lambda_{\alpha\beta\gamma c} \left( -\frac{3}{16} \right) \end{aligned} \quad (11)$$

$$\begin{aligned} \bigcirc_{ab|cd}^{(4)} &= \lambda_{\alpha\beta\delta a} \lambda_{\alpha\beta\gamma c} \lambda_{d\gamma\delta b} \left( \zeta_3 - \frac{11}{6} \right) \\ &+ \lambda_{\beta\gamma\delta a} \lambda_{c\alpha\beta a} \lambda_{d\gamma\delta b} \left( \frac{1}{2} - \frac{\zeta_3}{2} \right) \\ &+ \delta_{bd} \lambda_{\alpha\beta\gamma c} \lambda_{\alpha\delta\epsilon a} \lambda_{\gamma\delta\epsilon\beta} \left( \frac{7}{24} \right) \end{aligned} \quad (12)$$

$$\begin{aligned} \bigcirc_{ab|cd}^{(5)} &= \lambda_{\alpha\beta\delta d} \lambda_{\alpha\beta\gamma c} \lambda_{\delta\epsilon\zeta b} \lambda_{\gamma\epsilon\zeta a} \left( -\frac{1}{24} \right) \\ &+ \lambda_{\alpha\beta\delta c} \lambda_{\alpha\gamma\epsilon d} \lambda_{\beta\gamma\zeta a} \lambda_{\delta\epsilon\zeta b} \left( \frac{7\zeta_3}{4} - 2\zeta_5 + \frac{\pi^4}{80} \right) \end{aligned}$$

$$\begin{aligned}
& + \lambda_{\alpha\beta\gamma c} \lambda_{\alpha\delta\epsilon d} \lambda_{\beta\gamma\zeta a} \lambda_{\delta\epsilon\zeta b} \left( -\frac{1}{3} + \frac{\pi^4}{240} \right) \\
& + \lambda_{\alpha\beta\delta c} \lambda_{\alpha\beta\gamma a} \lambda_{\delta\epsilon\zeta b} \lambda_{\gamma\epsilon\zeta d} \left( \frac{\zeta_3}{8} + \frac{\pi^4}{480} - \frac{1}{3} \right) \\
& + \lambda_{\alpha\beta\gamma a} \lambda_{\alpha\beta\gamma c} \lambda_{\delta\epsilon\zeta b} \lambda_{\delta\epsilon\zeta d} \left( -\frac{25}{13824} \right) \\
& + \lambda_{\alpha\beta\gamma c} \lambda_{\beta\gamma\delta a} \lambda_{\delta\epsilon\zeta a} \lambda_{d\epsilon\zeta b} \left( \frac{157}{768} \right) \\
& + \lambda_{\alpha\beta\epsilon c} \lambda_{\beta\gamma\delta a} \lambda_{d\epsilon\zeta b} \lambda_{\gamma\delta\zeta a} \left( -\frac{2}{3} + \frac{\pi^4}{120} \right) \\
& + \delta_{bd} \lambda_{\alpha\zeta\eta a} \lambda_{\beta\zeta\eta\alpha} \lambda_{\gamma\delta\epsilon\beta} \lambda_{\gamma\delta\epsilon c} \left( -\frac{25}{6912} \right) \\
& + \lambda_{\alpha\beta\delta c} \lambda_{\beta\gamma\epsilon a} \lambda_{d\epsilon\zeta b} \lambda_{\gamma\delta\zeta a} \left( -\frac{15\zeta_3}{2} - \frac{\pi^4}{120} + \frac{73}{6} \right) \\
& + \delta_{bd} \lambda_{\alpha\zeta\eta a} \lambda_{\beta\epsilon\eta\alpha} \lambda_{\gamma\delta\epsilon c} \lambda_{\gamma\delta\zeta\beta} \left( \frac{\zeta_3}{2} - \frac{125}{96} \right) \\
& + \lambda_{\beta\gamma\delta a} \lambda_{\beta\gamma\epsilon\alpha} \lambda_{c\delta\zeta a} \lambda_{d\epsilon\zeta b} \left( -\frac{1075}{2304} \right) \\
& + \delta_{bd} \lambda_{\alpha\epsilon\eta c} \lambda_{\alpha\zeta\eta a} \lambda_{\gamma\delta\epsilon\beta} \lambda_{\gamma\delta\zeta\beta} \left( \frac{857}{4608} \right) \\
& + \lambda_{\beta\delta\zeta a} \lambda_{\beta\gamma\epsilon\alpha} \lambda_{c\gamma\delta a} \lambda_{d\epsilon\zeta b} \left( \frac{7\zeta_3}{4} + \frac{\pi^4}{480} - \frac{101}{48} \right) \\
& + \delta_{bd} \lambda_{\alpha\delta\epsilon c} \lambda_{\alpha\zeta\eta a} \lambda_{\gamma\delta\zeta\beta} \lambda_{\gamma\epsilon\eta\beta} \left( -\frac{\zeta_3}{2} - \frac{193}{768} \right) \\
& + \lambda_{\alpha\gamma\delta c} \lambda_{\beta\gamma\delta a} \lambda_{\beta\epsilon\zeta a} \lambda_{d\epsilon\zeta b} \left( \frac{11\zeta_3}{8} - \frac{\pi^4}{480} - \frac{7}{4} \right) \\
& + \lambda_{\beta\gamma\delta a} \lambda_{\beta\epsilon\zeta a} \lambda_{c\gamma\delta a} \lambda_{d\epsilon\zeta b} \left( \frac{3\zeta_3}{16} - \frac{\pi^4}{240} + \frac{7}{32} \right) \\
& + \delta_{bd} \lambda_{\alpha\delta\epsilon c} \lambda_{\alpha\zeta\eta a} \lambda_{\gamma\delta\epsilon\beta} \lambda_{\gamma\zeta\eta\beta} \left( \frac{81}{512} - \frac{3\zeta_3}{32} \right)
\end{aligned} \tag{13}$$

$$\begin{aligned}
\bigcirc_{ab|cd}^{(6)} = & \lambda_{\alpha\beta\zeta c} \lambda_{\beta\gamma\delta a} \lambda_{\gamma\delta\epsilon a} \lambda_{\epsilon\eta\theta d} \lambda_{\zeta\eta\theta b} \left( -\frac{3\zeta_3}{20} + \frac{3\zeta_5}{10} + \frac{\pi^4}{400} - \frac{11}{40} \right) \\
& + \lambda_{\alpha\beta\epsilon c} \lambda_{\beta\gamma\delta a} \lambda_{\gamma\delta\epsilon a} \lambda_{\zeta\eta\theta b} \lambda_{\zeta\eta\theta d} \left( \frac{\zeta_3}{96} + \frac{5}{576} \right) \\
& + \lambda_{\beta\gamma\delta a} \lambda_{\beta\gamma\epsilon\alpha} \lambda_{\delta\zeta\eta c} \lambda_{d\eta\theta b} \lambda_{\epsilon\zeta\theta a} \left( -\frac{7\zeta_3}{12} + \frac{\pi^4}{1440} + \frac{30337}{11520} \right) \\
& + \lambda_{\alpha\delta\eta c} \lambda_{\beta\gamma\zeta a} \lambda_{\beta\epsilon\theta d} \lambda_{\gamma\delta\epsilon a} \lambda_{\zeta\eta\theta b} \left( \frac{21\zeta_3^2}{10} + \frac{7}{300}\pi^4\zeta_3 - \frac{7\zeta_5}{2} + \frac{13\zeta_7}{20} - \frac{\pi^6}{252} \right) \\
& + \lambda_{\alpha\delta\epsilon c} \lambda_{\beta\eta\theta d} \lambda_{\beta\gamma\zeta a} \lambda_{\gamma\delta\epsilon a} \lambda_{\zeta\eta\theta b} \left( \frac{5\zeta_3}{4} - \frac{27\zeta_5}{40} + \frac{\pi^4}{400} - \frac{23}{40} \right) \\
& + \lambda_{\alpha\beta\delta c} \lambda_{\beta\gamma\zeta a} \lambda_{\gamma\delta\epsilon a} \lambda_{\epsilon\eta\theta d} \lambda_{\zeta\eta\theta b} \left( -\frac{14\zeta_3}{5} + \frac{13\zeta_5}{20} - \frac{\pi^4}{60} + \frac{17}{4} \right) \\
& + \lambda_{\beta\gamma\delta a} \lambda_{\beta\gamma\eta\alpha} \lambda_{\delta\epsilon\zeta c} \lambda_{d\eta\theta b} \lambda_{\epsilon\zeta\theta a} \left( -\frac{\zeta_3}{10} + \frac{\pi^4}{800} - \frac{457}{768} \right) \\
& + \delta_{bd} \lambda_{\alpha\theta\iota a} \lambda_{\gamma\delta\theta\beta} \lambda_{\gamma\delta\epsilon\beta} \lambda_{\epsilon\zeta\eta c} \lambda_{\zeta\eta\iota\alpha} \left( \frac{3\zeta_3}{160} + \frac{17}{240} \right) \\
& + \lambda_{\alpha\beta\gamma c} \lambda_{\beta\delta\epsilon a} \lambda_{\delta\epsilon\theta a} \lambda_{\gamma\zeta\eta d} \lambda_{\zeta\eta\theta b} \left( -\frac{7\zeta_3}{20} + \frac{3\zeta_5}{4} - \frac{\pi^4}{1200} - \frac{11}{40} \right) \\
& + \lambda_{\alpha\gamma\epsilon c} \lambda_{\beta\delta\zeta a} \lambda_{\beta\gamma\eta d} \lambda_{\delta\epsilon\theta a} \lambda_{\zeta\eta\theta b} \left( \frac{3\zeta_3^2}{5} + \frac{1}{150}\pi^4\zeta_3 - 7\zeta_5 + \frac{201\zeta_7}{20} - \frac{\pi^6}{126} \right) \\
& + \lambda_{\alpha\beta\gamma c} \lambda_{\beta\delta\zeta a} \lambda_{\delta\epsilon\theta a} \lambda_{\gamma\epsilon\eta d} \lambda_{\zeta\eta\theta b} \left( \frac{27\zeta_3^2}{10} - \frac{57\zeta_3}{10} + \frac{51\zeta_5}{10} - \frac{\pi^6}{315} - \frac{3\pi^4}{200} \right)
\end{aligned}$$

$$\begin{aligned}
& + \lambda_{\beta\delta\zeta\alpha}\lambda_{\beta\gamma\epsilon\alpha}\lambda_{d\eta\theta b}\lambda_{\gamma\delta\eta c}\lambda_{\epsilon\zeta\theta a}\left(-\frac{51\zeta_3}{10}-\frac{53\zeta_5}{20}-\frac{7\pi^4}{300}+\frac{35}{4}\right) \\
& + \lambda_{\beta\delta\eta\alpha}\lambda_{\beta\gamma\epsilon\alpha}\lambda_{d\eta\theta b}\lambda_{\gamma\delta\zeta c}\lambda_{\epsilon\zeta\theta a}\left(\frac{79\zeta_3}{5}+\frac{127\zeta_5}{10}+\frac{\pi^4}{60}-\frac{1207}{30}\right) \\
& + \lambda_{\beta\delta\theta\alpha}\lambda_{\beta\gamma\eta\alpha}\lambda_{\delta\epsilon\zeta a}\lambda_{d\eta\theta b}\lambda_{\gamma\epsilon\zeta c}\left(-\frac{109\zeta_3}{20}+\frac{31\zeta_5}{8}+\frac{3\pi^4}{400}+\frac{277}{120}\right) \\
& + \lambda_{\beta\gamma\delta\alpha}\lambda_{\beta\epsilon\zeta\alpha}\lambda_{d\eta\theta b}\lambda_{\gamma\delta\epsilon c}\lambda_{\zeta\eta\theta a}\left(-\frac{\zeta_3}{5}-\frac{\pi^4}{2400}-\frac{685}{768}\right) \\
& + \lambda_{\beta\gamma\delta\alpha}\lambda_{\beta\epsilon\zeta\alpha}\lambda_{d\eta\theta b}\lambda_{\gamma\delta\eta c}\lambda_{\epsilon\zeta\theta a}\left(-\frac{7\zeta_3}{20}+\frac{3\zeta_5}{4}-\frac{\pi^4}{1200}-\frac{11}{40}\right) \\
& + \lambda_{\beta\gamma\delta\alpha}\lambda_{\beta\epsilon\eta\alpha}\lambda_{d\eta\theta b}\lambda_{\gamma\delta\zeta c}\lambda_{\epsilon\zeta\theta a}\left(-\frac{\zeta_3}{5}+\frac{31\zeta_5}{5}-\frac{3\pi^4}{100}-\frac{91}{30}\right) \\
& + \delta_{bd}\lambda_{\alpha\theta i a}\lambda_{\delta\eta i \alpha}\lambda_{\gamma\delta\epsilon\beta}\lambda_{\gamma\zeta\theta\beta}\lambda_{\epsilon\zeta\eta c}\left(-\frac{43\zeta_3}{20}-\frac{\pi^4}{400}+\frac{8369}{1920}\right) \\
& + \lambda_{\beta\eta\theta\alpha}\lambda_{\beta\gamma\delta\alpha}\lambda_{\delta\epsilon\zeta a}\lambda_{d\eta\theta b}\lambda_{\gamma\epsilon\zeta c}\left(-\frac{33\zeta_3}{40}+\frac{6\zeta_5}{5}+\frac{\pi^4}{100}-\frac{79}{80}\right) \\
& + \lambda_{\alpha\beta\zeta c}\lambda_{\beta\eta\theta d}\lambda_{\gamma\delta\epsilon a}\lambda_{\gamma\delta\epsilon\alpha}\lambda_{\zeta\eta\theta b}\left(-\frac{\zeta_3}{4}+\frac{\pi^4}{1440}+\frac{757}{11520}\right) \\
& + \lambda_{\alpha\beta\eta c}\lambda_{\beta\epsilon\theta d}\lambda_{\gamma\delta\epsilon a}\lambda_{\gamma\delta\zeta\alpha}\lambda_{\zeta\eta\theta b}\left(-\frac{23}{5}\zeta_3^2-\frac{57\zeta_3}{5}+\frac{101\zeta_5}{5}-\frac{\pi^6}{945}-\frac{3\pi^4}{100}\right) \\
& + \lambda_{\alpha\beta\epsilon c}\lambda_{\beta\eta\theta d}\lambda_{\gamma\delta\epsilon a}\lambda_{\gamma\delta\zeta\alpha}\lambda_{\zeta\eta\theta b}\left(\frac{9\zeta_3}{5}-\frac{99\zeta_5}{20}-\frac{\pi^4}{50}+\frac{17}{4}\right) \\
& + \lambda_{\beta\delta\eta\alpha}\lambda_{\beta\gamma\zeta c}\lambda_{\delta\epsilon\zeta a}\lambda_{d\eta\theta b}\lambda_{\gamma\epsilon\theta\alpha}\left(-\frac{21}{10}\zeta_3^2-\frac{27\zeta_3}{2}+\frac{161\zeta_5}{10}+\frac{2\pi^6}{315}-\frac{7\pi^4}{120}\right) \\
& + \delta_{bd}\lambda_{\alpha\theta i a}\lambda_{\delta\zeta i \beta}\lambda_{\gamma\delta\eta\alpha}\lambda_{\gamma\epsilon\theta\beta}\lambda_{\epsilon\zeta\eta c}\left(\frac{19\zeta_3}{20}-\frac{\zeta_5}{5}+\frac{\pi^4}{75}\right) \\
& + \delta_{bd}\lambda_{\alpha\theta i a}\lambda_{\delta\eta\theta\beta}\lambda_{\gamma\delta i \alpha}\lambda_{\gamma\epsilon\zeta\beta}\lambda_{\epsilon\zeta\eta c}\left(-\frac{37\zeta_3}{20}+\frac{\pi^4}{300}+\frac{61}{24}\right) \\
& + \lambda_{\alpha\beta\gamma c}\lambda_{\beta\gamma\eta d}\lambda_{\delta\epsilon\theta a}\lambda_{\delta\epsilon\zeta\alpha}\lambda_{\zeta\eta\theta b}\left(-\frac{2\zeta_3}{5}-\frac{7\zeta_5}{20}-\frac{\pi^4}{300}+\frac{83}{60}\right) \\
& + \delta_{bd}\lambda_{\alpha\theta i a}\lambda_{\gamma\delta i \alpha}\lambda_{\gamma\delta\theta\beta}\lambda_{\epsilon\zeta\eta\beta}\lambda_{\epsilon\zeta\eta c}\left(\frac{\zeta_3}{48}+\frac{5}{288}\right) \\
& + \lambda_{\beta\gamma\eta\alpha}\lambda_{\beta\gamma\zeta c}\lambda_{\delta\epsilon\theta\alpha}\lambda_{\delta\epsilon\zeta a}\lambda_{d\eta\theta b}\left(\frac{13\zeta_3}{2}-\frac{32\zeta_5}{5}-\frac{\pi^4}{200}-\frac{91}{60}\right) \\
& + \lambda_{\beta\gamma\delta c}\lambda_{\beta\gamma\epsilon\alpha}\lambda_{\delta\zeta\eta\alpha}\lambda_{d\eta\theta b}\lambda_{\epsilon\zeta\theta a}\left(33\zeta_3+\frac{19\zeta_5}{10}+\frac{\pi^4}{100}-\frac{1207}{30}\right) \\
& + \lambda_{\beta\gamma\delta\alpha}\lambda_{\beta\gamma\delta c}\lambda_{d\eta\theta b}\lambda_{\epsilon\zeta\eta\alpha}\lambda_{\epsilon\zeta\theta a}\left(-\frac{\zeta_3}{4}+\frac{\pi^4}{1440}+\frac{757}{11520}\right) \\
& + \lambda_{\beta\gamma\delta\alpha}\lambda_{\beta\gamma\theta c}\lambda_{\delta\epsilon\zeta a}\lambda_{d\eta\theta b}\lambda_{\epsilon\zeta\eta\alpha}\left(\frac{9\zeta_3}{5}-\frac{99\zeta_5}{20}-\frac{\pi^4}{50}+\frac{17}{4}\right) \\
& + \delta_{bd}\lambda_{\alpha\theta i a}\lambda_{\gamma\delta i \alpha}\lambda_{\gamma\delta\epsilon\beta}\lambda_{\epsilon\zeta\eta c}\lambda_{\zeta\eta\theta\beta}\left(-\frac{13\zeta_3}{80}+\frac{\pi^4}{300}+\frac{27}{256}\right) \\
& + \lambda_{\beta\gamma\delta\alpha}\lambda_{\beta\gamma\zeta c}\lambda_{\delta\epsilon\zeta a}\lambda_{d\eta\theta b}\lambda_{\epsilon\eta\theta\alpha}\left(-\frac{73\zeta_3}{10}-\frac{27\zeta_5}{5}+\frac{\pi^4}{150}+\frac{779}{60}\right) \\
& + \lambda_{\beta\gamma\delta\alpha}\lambda_{\beta\epsilon\zeta\alpha}\lambda_{c\zeta\theta a}\lambda_{\delta\epsilon\eta\gamma}\lambda_{d\eta\theta b}\left(\frac{11\zeta_3}{40}+\frac{\pi^4}{2400}+\frac{7157}{3840}\right) \\
& + \delta_{bd}\lambda_{\alpha\eta i c}\lambda_{\alpha\theta i a}\lambda_{\gamma\delta\epsilon\beta}\lambda_{\gamma\zeta\eta\beta}\lambda_{\epsilon\zeta\theta\delta}\left(-\frac{\zeta_3}{40}-\frac{677}{960}\right) \\
& + \lambda_{\alpha\beta\theta d}\lambda_{\alpha\beta\epsilon c}\lambda_{\delta\zeta\eta\gamma}\lambda_{\gamma\delta\epsilon a}\lambda_{\zeta\eta\theta b}\left(\frac{\zeta_3}{40}+\frac{7\zeta_5}{20}+\frac{\pi^4}{400}-\frac{31}{48}\right) \\
& + \lambda_{\beta\delta\eta\alpha}\lambda_{\beta\gamma\epsilon\alpha}\lambda_{c\epsilon\zeta a}\lambda_{\delta\zeta\theta\gamma}\lambda_{d\eta\theta b}\left(-\frac{163\zeta_3}{20}-\frac{23\zeta_5}{5}+\frac{\pi^4}{120}+\frac{1429}{120}\right)
\end{aligned}$$

$$\begin{aligned}
& + \delta_{bd} \lambda_{\alpha\theta ia} \lambda_{\alpha\zeta\eta c} \lambda_{\gamma\delta\zeta\beta} \lambda_{\gamma\varepsilon\theta\beta} \lambda_{\varepsilon\eta i\delta} \left( \frac{33\zeta_3}{20} - \frac{\pi^4}{240} + \frac{2401}{1920} \right) \\
& + \lambda_{\beta\gamma\delta\alpha} \lambda_{\beta\varepsilon\eta\alpha} \lambda_{c\varepsilon\zeta a} \lambda_{\delta\zeta\theta\gamma} \lambda_{d\eta\theta b} \left( -2\zeta_3 - \frac{19\zeta_5}{10} + \frac{61}{15} \right) \\
& + \delta_{bd} \lambda_{\alpha\theta ia} \lambda_{\alpha\zeta\eta c} \lambda_{\gamma\delta\varepsilon\beta} \lambda_{\gamma\zeta\theta\beta} \lambda_{\varepsilon\eta i\delta} \left( \frac{7\zeta_3}{4} - \frac{\pi^4}{2400} - \frac{2293}{1280} \right) \\
& + \lambda_{\beta\delta\zeta\alpha} \lambda_{\beta\gamma\varepsilon\alpha} \lambda_{c\varepsilon\zeta a} \lambda_{\delta\eta\theta\gamma} \lambda_{d\eta\theta b} \left( \frac{9\zeta_3}{20} + \frac{53\zeta_5}{20} + \frac{\pi^4}{75} - \frac{31}{8} \right) \\
& + \delta_{bd} \lambda_{\alpha\theta ia} \lambda_{\alpha\zeta\eta c} \lambda_{\gamma\delta\zeta\beta} \lambda_{\gamma\varepsilon\eta\beta} \lambda_{\varepsilon\theta i\delta} \left( \frac{53\zeta_3}{80} - \frac{\pi^4}{480} + \frac{11}{1920} \right) \\
& + \lambda_{\beta\gamma\delta\alpha} \lambda_{\beta\varepsilon\zeta\alpha} \lambda_{c\varepsilon\zeta a} \lambda_{\delta\eta\theta\gamma} \lambda_{d\eta\theta b} \left( \frac{\zeta_3}{10} - \frac{3\zeta_5}{8} + \frac{\pi^4}{600} + \frac{1}{10} \right) \\
& + \delta_{bd} \lambda_{\alpha\theta ia} \lambda_{\alpha\zeta\eta c} \lambda_{\gamma\delta\varepsilon\beta} \lambda_{\gamma\zeta\eta\beta} \lambda_{\varepsilon\theta i\delta} \left( -\frac{3\zeta_3}{80} - \frac{\pi^4}{1200} + \frac{103}{1280} \right) \\
& + \lambda_{\alpha\beta\gamma c} \lambda_{\beta\delta\eta\alpha} \lambda_{\delta\varepsilon\zeta a} \lambda_{d\eta\theta b} \lambda_{\varepsilon\zeta\theta\gamma} \left( \frac{51\zeta_3}{20} - \frac{31\zeta_5}{20} - \frac{3\pi^4}{400} - \frac{91}{60} \right) \\
& + \lambda_{\alpha\beta\gamma c} \lambda_{\beta\delta\varepsilon\alpha} \lambda_{\delta\varepsilon\zeta a} \lambda_{d\eta\theta b} \lambda_{\zeta\eta\theta\gamma} \left( \frac{\zeta_3}{10} - \frac{23\zeta_5}{20} + \frac{\pi^4}{200} + \frac{7}{15} \right) \\
& + \lambda_{\beta\gamma\delta\alpha} \lambda_{\beta\gamma\varepsilon\alpha} \lambda_{c\varepsilon\zeta a} \lambda_{d\eta\theta b} \lambda_{\zeta\eta\theta\delta} \left( \frac{11\zeta_3}{24} - \frac{\pi^4}{1440} - \frac{9709}{11520} \right) \\
& + \delta_{bd} \lambda_{\alpha\theta ia} \lambda_{\alpha\zeta\eta c} \lambda_{\eta\theta i\varepsilon} \lambda_{\gamma\delta\varepsilon\beta} \lambda_{\gamma\delta\zeta\beta} \left( -\frac{\zeta_3}{24} - \frac{31}{160} \right) \\
& + \lambda_{\alpha\beta\gamma c} \lambda_{\beta\gamma\delta\alpha} \lambda_{\delta\varepsilon\zeta a} \lambda_{d\eta\theta b} \lambda_{\zeta\eta\theta\varepsilon} \left( \frac{11\zeta_3}{60} - \frac{7\pi^4}{7200} + \frac{201}{1280} \right)
\end{aligned} \tag{14}$$

$$\Delta_{ab|cde|fgh}^{(2)} = \delta_{af} \delta_{bc} \delta_{dg} \delta_{eh} \left( -\frac{1}{2} \right) \tag{15}$$

$$\begin{aligned}
\Delta_{ab|cde|fgh}^{(3)} &= \delta_{af} \delta_{eg} \lambda_{cdhb} (2) \\
&+ \delta_{af} \delta_{be} \lambda_{dghc} \left( -\frac{1}{4} \right)
\end{aligned} \tag{16}$$

$$\begin{aligned}
\Delta_{ab|cde|fgh}^{(4)} &= \lambda_{cfgb} \lambda_{deha} \left( \frac{5}{12} \right) \\
&+ \delta_{ef} \lambda_{cg\alpha b} \lambda_{dh\alpha a} \left( -3\zeta_3 - \frac{\pi^4}{60} \right) \\
&+ \delta_{ef} \lambda_{cd\alpha a} \lambda_{gh\alpha b} \left( \frac{5}{12} - \frac{\zeta_3}{2} \right) \\
&+ \delta_{df} \delta_{eg} \lambda_{c\alpha\beta a} \lambda_{h\alpha\beta b} \left( \frac{1}{4} \right) \\
&+ \delta_{af} \delta_{eg} \lambda_{d\alpha\beta c} \lambda_{h\alpha\beta b} \left( \frac{5}{6} - \zeta_3 \right) \\
&+ \delta_{af} \delta_{dg} \delta_{eh} \lambda_{\alpha\beta\gamma b} \lambda_{\alpha\beta\gamma c} \left( -\frac{37}{288} \right) \\
&+ \delta_{ae} \lambda_{cg\alpha b} \lambda_{fh\alpha d} (-5) \\
&+ \delta_{af} \delta_{be} \lambda_{g\alpha\beta c} \lambda_{h\alpha\beta d} \left( \frac{1}{2} - \zeta_3 \right) \\
&+ \delta_{bf} \lambda_{cd\alpha a} \lambda_{gh\alpha e} \left( \frac{2}{3} \right) \\
&+ \delta_{bg} \delta_{df} \lambda_{c\alpha\beta a} \lambda_{h\alpha\beta e} (4\zeta_3 - 5) \\
&+ \delta_{af} \delta_{be} \lambda_{d\alpha\beta c} \lambda_{h\alpha\beta g} \left( \frac{\zeta_3}{4} - \frac{1}{8} \right) \\
&+ \delta_{af} \delta_{bd} \delta_{eg} \lambda_{\alpha\beta\gamma c} \lambda_{\alpha\beta\gamma h} \left( \frac{121}{288} \right)
\end{aligned} \tag{17}$$

$$\begin{aligned}
\triangle_{ab|cde|fgh}^{(5)} = & \delta_{eg} \lambda_{\alpha\beta\gamma a} \lambda_{df\gamma c} \lambda_{h\alpha\beta b} \left( -\frac{4}{3} \right) \\
& + \lambda_{de\beta b} \lambda_{f\alpha\beta c} \lambda_{gh\alpha a} \left( \frac{1}{3} \right) \\
& + \delta_{ef} \lambda_{\alpha\beta\gamma b} \lambda_{dh\gamma a} \lambda_{g\alpha\beta c} \left( 4\zeta_3 - \frac{7\zeta_5}{2} \right) \\
& + \delta_{ef} \lambda_{d\beta\gamma a} \lambda_{g\alpha\beta b} \lambda_{h\alpha\gamma c} \left( -\zeta_3^2 + 15\zeta_5 + \frac{5\pi^6}{378} \right) \\
& + \delta_{ef} \lambda_{\alpha\beta\gamma c} \lambda_{dh\gamma a} \lambda_{g\alpha\beta b} (8\zeta_3 - 12\zeta_5) \\
& + \lambda_{c\alpha\beta a} \lambda_{eghd} \lambda_{f\alpha\beta b} \left( -\frac{3\zeta_3}{16} - \frac{\pi^4}{960} + \frac{5}{48} \right) \\
& + \lambda_{c\alpha\beta a} \lambda_{eh\beta d} \lambda_{fg\alpha b} \left( \frac{7\zeta_3}{4} - \frac{\pi^4}{240} - \frac{5}{3} \right) \\
& + \lambda_{cg\alpha a} \lambda_{eh\beta d} \lambda_{f\alpha\beta b} (8\zeta_3 + 3\zeta_5) \\
& + \lambda_{ch\beta a} \lambda_{e\alpha\beta d} \lambda_{fg\alpha b} \left( -\frac{5}{3} \right) \\
& + \lambda_{cgha} \lambda_{e\alpha\beta d} \lambda_{f\alpha\beta b} \left( -\frac{\zeta_3}{2} - \frac{\pi^4}{240} + \frac{3}{8} \right) \\
& + \delta_{ae} \lambda_{\alpha\beta\gamma b} \lambda_{fh\gamma d} \lambda_{g\alpha\beta c} \left( -\frac{3\zeta_3}{2} + \frac{\pi^4}{120} - \frac{1}{2} \right) \\
& + \delta_{ae} \lambda_{\alpha\beta\gamma c} \lambda_{fh\gamma d} \lambda_{g\alpha\beta b} \left( -\frac{9\zeta_3}{4} + \frac{\pi^4}{80} - \frac{1}{2} \right) \\
& + \delta_{ae} \lambda_{f\beta\gamma d} \lambda_{g\alpha\beta b} \lambda_{h\alpha\gamma c} \left( \frac{25\zeta_3}{2} - \frac{23\zeta_5}{2} + \frac{7\pi^4}{120} \right) \\
& + \lambda_{c\alpha\beta a} \lambda_{dghb} \lambda_{f\alpha\beta e} \left( \frac{\zeta_3}{2} + \frac{\pi^4}{120} - \frac{5}{3} \right) \\
& + \lambda_{cg\alpha a} \lambda_{dh\beta b} \lambda_{f\alpha\beta e} \left( -\frac{7}{2}\zeta_3^2 + \frac{15\zeta_5}{2} + \frac{5\pi^6}{756} \right) \\
& + \delta_{ef} \lambda_{c\alpha\gamma b} \lambda_{d\beta\gamma a} \lambda_{h\alpha\beta g} (4\zeta_3 + 4\zeta_5) \\
& + \delta_{ef} \lambda_{\alpha\beta\gamma b} \lambda_{cd\gamma a} \lambda_{h\alpha\beta g} \left( \frac{\zeta_3}{4} - \frac{\pi^4}{120} + \frac{3}{8} \right) \\
& + \delta_{ae} \lambda_{\alpha\beta\gamma b} \lambda_{df\gamma c} \lambda_{h\alpha\beta g} \left( -\frac{\zeta_3}{8} - \frac{\pi^4}{480} \right) \\
& + \delta_{ae} \lambda_{\alpha\beta\gamma c} \lambda_{df\gamma b} \lambda_{h\alpha\beta g} \left( \frac{9\zeta_3}{4} + \frac{\pi^4}{240} - \frac{1}{2} \right) \\
& + \delta_{af} \lambda_{c\alpha\gamma b} \lambda_{e\beta\gamma d} \lambda_{h\alpha\beta g} \left( -\frac{7}{3} \right) \\
& + \delta_{ae} \lambda_{c\alpha\gamma b} \lambda_{f\beta\gamma d} \lambda_{h\alpha\beta g} (14) \\
& + \delta_{bf} \lambda_{\alpha\beta\gamma e} \lambda_{cd\gamma a} \lambda_{h\alpha\beta g} \left( -\frac{5\zeta_3}{8} + \frac{\pi^4}{480} + \frac{3}{8} \right) \\
& + \delta_{ef} \lambda_{\alpha\beta\gamma g} \lambda_{cd\gamma a} \lambda_{h\alpha\beta b} \left( -\frac{3\zeta_3}{4} + \frac{\pi^4}{240} - \frac{5}{3} \right) \\
& + \delta_{ef} \lambda_{\alpha\beta\gamma b} \lambda_{\alpha\beta\gamma g} \lambda_{cdha} \left( -\frac{55}{2304} \right) \\
& + \delta_{ae} \lambda_{\alpha\beta\gamma b} \lambda_{\alpha\beta\gamma g} \lambda_{dfhc} \left( \frac{\zeta_3}{12} - \frac{151}{2304} \right) \\
& + \delta_{ae} \lambda_{\alpha\beta\gamma g} \lambda_{df\gamma c} \lambda_{h\alpha\beta b} \left( -\frac{\zeta_3}{2} + \frac{\pi^4}{120} - \frac{7}{3} \right) \\
& + \delta_{ae} \lambda_{\alpha\beta\gamma g} \lambda_{df\gamma b} \lambda_{h\alpha\beta c} \left( -7\zeta_3 - \frac{\pi^4}{60} + 14 \right)
\end{aligned}$$

$$\begin{aligned}
& + \delta_{ae} \lambda_{\alpha\beta\gamma g} \lambda_{c\alpha\beta b} \lambda_{fh\gamma d} \left( \frac{7\zeta_3}{4} - \frac{\pi^4}{240} - \frac{5}{3} \right) \\
& + \delta_{af} \delta_{be} \lambda_{\alpha\beta\delta c} \lambda_{\alpha\beta\gamma g} \lambda_{h\gamma\delta d} \left( \frac{9\zeta_3}{4} - \frac{\pi^4}{80} - \frac{13}{12} \right) \\
& + \delta_{bf} \lambda_{\alpha\beta\gamma g} \lambda_{cd\gamma a} \lambda_{h\alpha\beta e} \left( 2\zeta_3 - \frac{\pi^4}{120} - \frac{5}{6} \right) \\
& + \delta_{bf} \lambda_{\alpha\beta\gamma e} \lambda_{\alpha\beta\gamma g} \lambda_{cdha} \left( \frac{103}{384} - \frac{\zeta_3}{6} \right) \\
& + \delta_{df} \delta_{eg} \lambda_{\alpha\beta\delta b} \lambda_{\alpha\beta\gamma h} \lambda_{c\gamma\delta a} \left( -\frac{\zeta_3}{4} + \frac{\pi^4}{240} - \frac{11}{12} \right) \\
& + \delta_{af} \delta_{eg} \lambda_{\alpha\beta\delta b} \lambda_{\alpha\beta\gamma h} \lambda_{d\gamma\delta c} \left( -\frac{3\zeta_3}{4} + \frac{\pi^4}{240} - \frac{5}{3} \right) \\
& + \delta_{bg} \delta_{df} \lambda_{\alpha\beta\delta e} \lambda_{\alpha\beta\gamma h} \lambda_{c\gamma\delta a} (14 - 8\zeta_3) \\
& + \delta_{ad} \delta_{eg} \lambda_{\alpha\beta\delta h} \lambda_{\alpha\beta\gamma b} \lambda_{f\gamma\delta c} \left( -13\zeta_3 + \frac{\pi^4}{60} + 14 \right) \\
& + \delta_{be} \delta_{df} \lambda_{\alpha\beta\delta h} \lambda_{\alpha\beta\gamma g} \lambda_{c\gamma\delta a} \left( \frac{23\zeta_3}{4} + \frac{\pi^4}{240} - \frac{9}{2} \right) \\
& + \delta_{af} \delta_{be} \lambda_{\alpha\beta\delta h} \lambda_{\alpha\beta\gamma g} \lambda_{d\gamma\delta c} \left( -\frac{5\zeta_3}{8} - \frac{\pi^4}{480} + \frac{29}{24} \right) \\
& + \delta_{df} \delta_{eg} \lambda_{\beta\gamma\delta\alpha} \lambda_{c\gamma\delta a} \lambda_{h\alpha\beta b} \left( \frac{\zeta_3}{16} - \frac{\pi^4}{320} + \frac{11}{24} \right) \\
& + \delta_{af} \delta_{eg} \lambda_{\alpha\beta\gamma b} \lambda_{\beta\gamma\delta\alpha} \lambda_{dh\delta c} \left( -\frac{55}{2304} \right) \\
& + \delta_{af} \delta_{eg} \lambda_{\beta\gamma\delta\alpha} \lambda_{d\gamma\delta c} \lambda_{h\alpha\beta b} \left( \frac{\zeta_3}{4} - \frac{\pi^4}{120} + \frac{3}{8} \right) \\
& + \delta_{af} \delta_{dg} \delta_{eh} \lambda_{\alpha\beta\epsilon b} \lambda_{\beta\gamma\delta\alpha} \lambda_{\gamma\delta\epsilon c} \left( \frac{\zeta_3}{8} + \frac{293}{768} \right) \\
& + \delta_{af} \delta_{be} \lambda_{\beta\gamma\delta\alpha} \lambda_{g\alpha\beta c} \lambda_{h\gamma\delta d} \left( \frac{7\zeta_3}{4} - \frac{\pi^4}{480} - \frac{85}{48} \right) \\
& + \delta_{bg} \delta_{df} \lambda_{\beta\gamma\delta\alpha} \lambda_{c\gamma\delta a} \lambda_{h\alpha\beta e} \left( -\frac{3\zeta_3}{4} + \frac{\pi^4}{48} - \frac{1}{2} \right) \\
& + \delta_{bg} \delta_{df} \lambda_{\alpha\beta\gamma e} \lambda_{\beta\gamma\delta\alpha} \lambda_{ch\delta a} \left( -\frac{2387}{1152} \right) \\
& + \delta_{af} \delta_{be} \lambda_{\beta\gamma\delta\alpha} \lambda_{d\gamma\delta c} \lambda_{h\alpha\beta g} \left( -\frac{\zeta_3}{8} + \frac{\pi^4}{480} - \frac{1}{16} \right) \\
& + \delta_{af} \delta_{be} \lambda_{\alpha\beta\gamma g} \lambda_{\beta\gamma\delta\alpha} \lambda_{dh\delta c} \left( \frac{755}{2304} \right) \\
& + \delta_{af} \delta_{eg} \lambda_{\alpha\beta\gamma h} \lambda_{\beta\gamma\delta\alpha} \lambda_{cd\delta b} \left( \frac{103}{384} \right) \\
& + \delta_{af} \delta_{bd} \delta_{eg} \lambda_{\alpha\beta\epsilon h} \lambda_{\beta\gamma\delta\alpha} \lambda_{\gamma\delta\epsilon c} \left( -\frac{\zeta_3}{8} - \frac{841}{768} \right)
\end{aligned} \tag{18}$$

$$\begin{aligned}
\triangle_{ab|cde|fgh}^{(6)} &= \lambda_{\alpha\beta\delta b} \lambda_{\alpha\beta\gamma a} \lambda_{ef\delta d} \lambda_{gh\gamma c} \left( \frac{1}{6} \right) \\
& + \lambda_{\alpha\beta\delta a} \lambda_{ef\delta d} \lambda_{g\alpha\gamma b} \lambda_{h\beta\gamma c} \left( \frac{32\zeta_3^2}{5} + \frac{2}{75}\pi^4\zeta_3 - 26\zeta_5 - \frac{797\zeta_7}{40} - \frac{\pi^6}{189} \right) \\
& + \lambda_{\alpha\beta\gamma a} \lambda_{ef\delta d} \lambda_{g\alpha\delta b} \lambda_{h\beta\gamma c} \left( -\frac{5}{2}\zeta_3^2 - \frac{9\zeta_3}{10} + \frac{41\zeta_5}{10} + \frac{\pi^6}{1890} + \frac{\pi^4}{40} \right) \\
& + \lambda_{\alpha\beta\gamma a} \lambda_{ef\delta d} \lambda_{g\alpha\beta b} \lambda_{h\gamma\delta c} \left( \frac{71}{15} \right) \\
& + \lambda_{\alpha\beta\gamma c} \lambda_{ef\delta d} \lambda_{g\alpha\beta a} \lambda_{h\gamma\delta b} \left( -\frac{3}{5}\zeta_3^2 - \frac{9\zeta_3}{10} + \frac{33\zeta_5}{5} - \frac{\pi^6}{1260} + \frac{\pi^4}{40} \right)
\end{aligned}$$

$$\begin{aligned}
& + \lambda_{\beta\gamma\delta c} \lambda_{ef\delta d} \lambda_{g\alpha\beta a} \lambda_{h\alpha\gamma b} \left( \frac{9\zeta_3^2}{20} - \frac{27\zeta_3}{2} - \frac{54\zeta_5}{5} + \frac{\pi^6}{630} \right) \\
& + \lambda_{\alpha\gamma\delta a} \lambda_{e\gamma\delta d} \lambda_{f\alpha\beta c} \lambda_{gh\beta b} \left( -\frac{3\zeta_3}{4} - \frac{7\zeta_5}{40} + \frac{\pi^4}{600} + \frac{1}{60} \right) \\
& + \lambda_{\alpha\beta\gamma a} \lambda_{e\gamma\delta d} \lambda_{f\alpha\beta c} \lambda_{gh\delta b} \left( -\frac{9\zeta_3}{10} - \frac{4\zeta_5}{5} - \frac{\pi^4}{600} + \frac{61}{60} \right) \\
& + \lambda_{e\gamma\delta d} \lambda_{f\alpha\beta c} \lambda_{g\alpha\gamma a} \lambda_{h\beta\delta b} \left( \frac{37\zeta_3^2}{5} - \frac{1}{150}\pi^4\zeta_3 - 13\zeta_5 - \frac{69\zeta_7}{10} - \frac{\pi^6}{378} \right) \\
& + \lambda_{e\gamma\delta d} \lambda_{f\alpha\beta c} \lambda_{g\alpha\beta a} \lambda_{h\gamma\delta b} \left( \frac{2\zeta_3}{5} + \frac{7\zeta_5}{40} + \frac{\pi^4}{240} - 1 \right) \\
& + \lambda_{e\gamma\delta d} \lambda_{f\beta\delta c} \lambda_{g\alpha\beta a} \lambda_{h\alpha\gamma b} \left( \frac{11\zeta_3^2}{10} - 27\zeta_3 - \frac{58\zeta_5}{5} + \frac{\pi^6}{1890} \right) \\
& + \delta_{eg} \lambda_{\alpha\beta\delta a} \lambda_{\alpha\gamma\epsilon b} \lambda_{f\delta\epsilon d} \lambda_{h\beta\gamma c} \left( -9\zeta_3^2 - \frac{3}{50}\pi^4\zeta_3 \right) \\
& + \delta_{eg} \lambda_{\alpha\beta\gamma a} \lambda_{\alpha\delta\epsilon b} \lambda_{f\delta\epsilon d} \lambda_{h\beta\gamma c} \left( \frac{3\zeta_3^2}{40} - \frac{9\zeta_3}{40} + \frac{21\zeta_5}{40} - \frac{\pi^6}{840} + \frac{\pi^4}{160} \right) \\
& + \delta_{eg} \lambda_{\alpha\beta\delta b} \lambda_{\alpha\beta\gamma a} \lambda_{f\delta\epsilon d} \lambda_{h\gamma\epsilon c} \left( \frac{3\zeta_3^2}{40} + \frac{33\zeta_3}{20} + \frac{7\zeta_5}{10} + \frac{\pi^6}{2520} + \frac{\pi^4}{300} \right) \\
& + \lambda_{\alpha\beta\delta b} \lambda_{eh\delta a} \lambda_{f\alpha\gamma c} \lambda_{g\beta\gamma d} \left( -\frac{162}{5}\zeta_3^2 - \frac{3}{25}\pi^4\zeta_3 + \frac{189\zeta_7}{5} \right) \\
& + \lambda_{\alpha\beta\gamma b} \lambda_{eh\delta a} \lambda_{f\alpha\beta c} \lambda_{g\gamma\delta d} \left( \frac{37\zeta_3^2}{5} - \frac{1}{150}\pi^4\zeta_3 - 13\zeta_5 + \frac{71\zeta_7}{10} - \frac{\pi^6}{378} \right) \\
& + \lambda_{e\gamma\delta a} \lambda_{f\gamma\delta b} \lambda_{g\alpha\beta c} \lambda_{h\alpha\beta d} \left( \frac{3\zeta_3}{4} + \frac{3\zeta_5}{4} + \frac{\pi^4}{400} - \frac{29}{20} \right) \\
& + \lambda_{e\gamma\delta a} \lambda_{f\alpha\gamma b} \lambda_{g\alpha\beta c} \lambda_{h\beta\delta d} \left( \frac{81\zeta_{35}}{25} + 27\zeta_3\zeta_5 - \frac{1323\zeta_7}{40} - \frac{2063\pi^8}{420000} \right) \\
& + \lambda_{e\gamma\delta a} \lambda_{f\alpha\beta b} \lambda_{g\alpha\gamma c} \lambda_{h\beta\delta d} \left( -36\zeta_3^2 - \frac{3}{25}\pi^4\zeta_3 + \frac{189\zeta_7}{4} \right) \\
& + \lambda_{e\gamma\delta a} \lambda_{f\alpha\beta b} \lambda_{g\alpha\beta c} \lambda_{h\gamma\delta d} \left( \frac{13\zeta_3}{5} + \frac{\zeta_5}{5} - \frac{\pi^4}{150} - \frac{6}{5} \right) \\
& + \lambda_{\alpha\beta\gamma b} \lambda_{c\gamma\delta a} \lambda_{eh\delta d} \lambda_{g\alpha\beta f} \left( \frac{\zeta_3}{5} - \frac{9\zeta_5}{40} + \frac{13\pi^4}{1200} - 1 \right) \\
& + \lambda_{\alpha\gamma\delta b} \lambda_{c\beta\gamma a} \lambda_{eh\delta d} \lambda_{g\alpha\beta f} \left( -\zeta_3^2 - \frac{9\zeta_3}{10} - \frac{17\zeta_5}{5} + \frac{17\pi^6}{3780} + \frac{\pi^4}{40} \right) \\
& + \lambda_{c\beta\delta a} \lambda_{e\gamma\delta d} \lambda_{g\alpha\beta f} \lambda_{h\alpha\gamma b} \left( -\frac{6}{5} \right) \\
& + \lambda_{c\alpha\beta a} \lambda_{e\gamma\delta d} \lambda_{g\alpha\beta f} \lambda_{h\gamma\delta b} \left( \frac{9\zeta_3}{40} - \frac{21\zeta_5}{40} - \frac{\pi^4}{800} + \frac{7}{80} \right) \\
& + \lambda_{\alpha\gamma\delta b} \lambda_{ch\beta a} \lambda_{e\gamma\delta d} \lambda_{g\alpha\beta f} \left( \frac{3\zeta_3}{10} - \frac{21\zeta_5}{40} + \frac{\pi^4}{400} - 1 \right) \\
& + \lambda_{c\beta\delta a} \lambda_{e\gamma\delta d} \lambda_{g\alpha\gamma f} \lambda_{h\alpha\beta b} \left( -\frac{11\zeta_3}{20} + \frac{3\zeta_5}{20} + \frac{7\pi^4}{1200} - \frac{6}{5} \right) \\
& + \lambda_{c\alpha\beta a} \lambda_{e\gamma\delta d} \lambda_{g\alpha\gamma f} \lambda_{h\beta\delta b} \left( -\frac{1}{2}\zeta_3^2 - \frac{9\zeta_3}{20} + \frac{13\zeta_5}{10} + \frac{17\pi^6}{7560} + \frac{\pi^4}{80} \right) \\
& + \lambda_{\alpha\beta\delta b} \lambda_{ch\beta a} \lambda_{e\gamma\delta d} \lambda_{g\alpha\gamma f} \left( \frac{21\zeta_3^2}{20} - \frac{9\zeta_3}{20} - \frac{9\zeta_5}{20} + \frac{\pi^6}{630} + \frac{\pi^4}{80} \right) \\
& + \lambda_{\alpha\beta\gamma b} \lambda_{c\beta\gamma a} \lambda_{eh\delta d} \lambda_{g\alpha\delta f} \left( \frac{19\zeta_3}{20} + \frac{3\zeta_5}{20} + \frac{\pi^4}{1200} - \frac{4}{5} \right) \\
& + \lambda_{c\alpha\beta a} \lambda_{e\gamma\delta d} \lambda_{g\gamma\delta f} \lambda_{h\alpha\beta b} \left( \frac{13\zeta_3}{80} - \frac{9\zeta_5}{160} - \frac{\pi^4}{960} + \frac{1}{32} \right) \\
& + \lambda_{\alpha\beta\delta b} \lambda_{\alpha\beta\gamma f} \lambda_{deha} \lambda_{g\gamma\delta c} \left( -5\zeta_3 + \frac{29\zeta_5}{10} - \frac{\pi^4}{50} + \frac{73}{10} \right)
\end{aligned}$$

$$\begin{aligned}
& + \lambda_{\alpha\beta\gamma c} \lambda_{\alpha\beta\gamma f} \lambda_{de\delta a} \lambda_{gh\delta b} \left( -\frac{\zeta_3}{240} - \frac{17\pi^4}{28800} + \frac{221}{3072} \right) \\
& + \lambda_{\alpha\beta\gamma f} \lambda_{\beta\gamma\delta c} \lambda_{de\delta a} \lambda_{gh\alpha b} \left( \frac{\zeta_3}{40} - \frac{3\zeta_5}{40} - \frac{\pi^4}{480} + \frac{1}{4} \right) \\
& + \lambda_{\alpha\beta\delta b} \lambda_{\alpha\beta\gamma f} \lambda_{c\gamma\delta a} \lambda_{eghd} \left( \frac{3\zeta_3}{5} - \frac{13}{60} \right) \\
& + \lambda_{\alpha\beta\gamma f} \lambda_{c\gamma\delta a} \lambda_{eh\delta d} \lambda_{g\alpha\beta b} \left( \frac{9\zeta_3}{2} + 3\zeta_5 - \frac{\pi^4}{200} - \frac{12}{5} \right) \\
& + \lambda_{\alpha\beta\gamma f} \lambda_{c\beta\gamma a} \lambda_{eh\delta d} \lambda_{g\alpha\delta b} \left( \frac{34\zeta_3^2}{5} - \frac{9\zeta_3}{10} - \frac{2\zeta_5}{5} - \frac{13\pi^6}{3780} + \frac{\pi^4}{40} \right) \\
& + \lambda_{\alpha\beta\gamma b} \lambda_{\alpha\beta\gamma f} \lambda_{c\gamma\delta a} \lambda_{eh\delta d} \left( -\frac{2767}{23040} \right) \\
& + \lambda_{\alpha\beta\delta b} \lambda_{\alpha\beta\gamma f} \lambda_{c\gamma\delta a} \lambda_{eh\delta d} \left( -\frac{3}{5}\zeta_3^2 - \frac{9\zeta_3}{10} + \frac{33\zeta_5}{5} - \frac{\pi^6}{1260} + \frac{\pi^4}{40} \right) \\
& + \lambda_{\alpha\beta\gamma f} \lambda_{c\beta\delta a} \lambda_{e\gamma\delta d} \lambda_{gh\alpha b} \left( -\frac{13}{10} \right) \\
& + \lambda_{\alpha\beta\gamma f} \lambda_{c\alpha\beta a} \lambda_{e\gamma\delta d} \lambda_{gh\delta b} \left( -\frac{3\zeta_3}{4} - \frac{9\zeta_5}{20} - \frac{\pi^4}{400} + \frac{61}{60} \right) \\
& + \lambda_{\alpha\beta\delta b} \lambda_{\alpha\beta\gamma f} \lambda_{c\gamma\delta a} \lambda_{e\gamma\delta d} \left( \frac{3\zeta_3}{2} - \frac{3\zeta_5}{4} - 1 \right) \\
& + \lambda_{\alpha\beta\gamma f} \lambda_{c\gamma\delta a} \lambda_{dh\delta b} \lambda_{g\alpha\beta e} \left( -\frac{43}{10}\zeta_3^2 - 27\zeta_3 + \frac{62\zeta_5}{5} + \frac{8\pi^6}{945} \right) \\
& + \lambda_{\alpha\beta\gamma f} \lambda_{c\beta\gamma a} \lambda_{dh\delta b} \lambda_{g\alpha\delta e} \left( \frac{44\zeta_3^2}{5} - \frac{4}{75}\pi^4\zeta_3 - 26\zeta_5 + \frac{1191\zeta_7}{40} - \frac{\pi^6}{189} \right) \\
& + \lambda_{\alpha\beta\gamma e} \lambda_{\alpha\beta\gamma f} \lambda_{c\gamma\delta a} \lambda_{dh\delta b} \left( \frac{151\zeta_3}{160} + \frac{29\zeta_5}{80} + \frac{\pi^4}{1200} \right) \\
& + \lambda_{\alpha\beta\delta e} \lambda_{\alpha\beta\gamma f} \lambda_{c\gamma\delta a} \lambda_{dh\delta b} \left( \frac{52\zeta_3^2}{5} + \frac{1}{75}\pi^4\zeta_3 - 13\zeta_5 - \frac{293\zeta_7}{80} - \frac{\pi^6}{378} \right) \\
& + \lambda_{\alpha\beta\delta f} \lambda_{\alpha\beta\gamma c} \lambda_{de\delta a} \lambda_{gh\gamma b} \left( -\frac{3\zeta_3}{10} + \frac{31\zeta_5}{40} + \frac{\pi^4}{300} - \frac{11}{15} \right) \\
& + \lambda_{\alpha\beta\delta f} \lambda_{c\beta\gamma a} \lambda_{eh\delta d} \lambda_{g\alpha\gamma b} \left( \frac{2\zeta_3^2}{5} - \frac{1}{75}\pi^4\zeta_3 - 26\zeta_5 - \frac{61\zeta_7}{10} - \frac{\pi^6}{189} \right) \\
& + \lambda_{\alpha\beta\delta f} \lambda_{\alpha\beta\gamma b} \lambda_{c\gamma\delta a} \lambda_{eh\delta d} \left( -\frac{5}{2}\zeta_3^2 - \frac{9\zeta_3}{10} + \frac{41\zeta_5}{10} + \frac{\pi^6}{1890} + \frac{\pi^4}{40} \right) \\
& + \lambda_{\alpha\beta\delta f} \lambda_{c\beta\gamma a} \lambda_{dh\delta b} \lambda_{g\alpha\gamma e} \left( \frac{162\zeta_3^2}{25} + 72\zeta_3\zeta_5 - \frac{1323\zeta_7}{20} - \frac{2063\pi^8}{210000} \right) \\
& + \lambda_{\alpha\gamma\delta f} \lambda_{c\alpha\beta a} \lambda_{e\gamma\delta d} \lambda_{gh\beta b} \left( -\frac{3\zeta_3}{5} + \frac{\pi^4}{100} + \frac{61}{60} \right) \\
& + \delta_{ef} \lambda_{\alpha\beta\gamma b} \lambda_{d\delta\epsilon c} \lambda_{\gamma\delta\epsilon a} \lambda_{h\alpha\beta g} \left( \frac{7\zeta_3}{40} - \frac{3\zeta_5}{8} + \frac{\pi^4}{800} + \frac{7}{80} \right) \\
& + \delta_{ef} \lambda_{\alpha\gamma\delta b} \lambda_{\beta\gamma\epsilon a} \lambda_{d\delta\epsilon c} \lambda_{h\alpha\beta g} \left( -\frac{27}{40}\zeta_3^2 - \frac{9\zeta_3}{40} - \frac{129\zeta_5}{40} + \frac{\pi^6}{1260} + \frac{\pi^4}{160} \right) \\
& + \delta_{ef} \lambda_{\alpha\beta\gamma c} \lambda_{d\delta\epsilon a} \lambda_{\gamma\delta\epsilon b} \lambda_{h\alpha\beta g} \left( \frac{\zeta_3}{2} + \frac{7\zeta_5}{40} + \frac{\pi^4}{400} + \frac{1}{3} \right) \\
& + \delta_{ef} \lambda_{\alpha\gamma\delta b} \lambda_{\beta\gamma\epsilon c} \lambda_{d\delta\epsilon a} \lambda_{h\alpha\beta g} \left( \frac{2\zeta_3^2}{5} - \frac{1}{75}\pi^4\zeta_3 - 26\zeta_5 - \frac{201\zeta_7}{10} - \frac{\pi^6}{189} \right) \\
& + \delta_{ef} \lambda_{\alpha\beta\gamma b} \lambda_{d\delta\epsilon a} \lambda_{\gamma\delta\epsilon c} \lambda_{h\alpha\beta g} \left( \frac{3\zeta_3}{10} + \frac{99\zeta_5}{40} + \frac{\pi^4}{400} - 1 \right) \\
& + \delta_{ae} \lambda_{\alpha\beta\gamma b} \lambda_{f\delta\epsilon d} \lambda_{\gamma\delta\epsilon c} \lambda_{h\alpha\beta g} \left( \frac{\zeta_3}{20} - \frac{17\zeta_5}{10} + \frac{7\pi^4}{600} + \frac{3}{40} \right) \\
& + \delta_{bf} \lambda_{\alpha\beta\gamma e} \lambda_{d\delta\epsilon a} \lambda_{\gamma\delta\epsilon c} \lambda_{h\alpha\beta g} \left( \frac{27\zeta_3}{20} + \frac{15\zeta_5}{8} - \frac{7\pi^4}{1200} - \frac{221}{120} \right)
\end{aligned}$$



$$\begin{aligned}
& + \delta_{bf} \lambda_{\alpha\gamma\delta e} \lambda_{\beta\gamma\epsilon c} \lambda_{d\delta\epsilon a} \lambda_{h\alpha\beta g} \left( \frac{81\zeta_3^2}{20} + 5\zeta_3 - \frac{23\zeta_5}{10} - \frac{\pi^6}{315} + \frac{\pi^4}{40} \right) \\
& + \lambda_{\alpha\beta\delta a} \lambda_{de\delta b} \lambda_{f\beta\gamma c} \lambda_{h\alpha\gamma g} \left( -\frac{43\zeta_3}{10} - \frac{7\zeta_5}{20} + \frac{\pi^4}{100} + \frac{73}{10} \right) \\
& + \delta_{af} \lambda_{\alpha\beta\delta b} \lambda_{\beta\gamma\epsilon c} \lambda_{e\delta\epsilon d} \lambda_{h\alpha\gamma g} \left( \frac{227}{30} \right) \\
& + \delta_{ae} \lambda_{\alpha\beta\delta b} \lambda_{\beta\gamma\epsilon c} \lambda_{f\delta\epsilon d} \lambda_{h\alpha\gamma g} \left( -\frac{53}{10}\zeta_3^2 - \frac{96\zeta_3}{5} + \frac{62\zeta_5}{5} - \frac{8\pi^6}{945} - \frac{\pi^4}{100} \right) \\
& + \lambda_{\alpha\beta\delta f} \lambda_{c\beta\gamma b} \lambda_{de\delta a} \lambda_{h\alpha\gamma g} \left( \frac{73}{10} \right) \\
& + \delta_{ef} \lambda_{\alpha\beta\gamma b} \lambda_{\beta\gamma\epsilon a} \lambda_{d\delta\epsilon c} \lambda_{h\alpha\delta g} \left( \frac{\zeta_3}{4} + \frac{7\zeta_5}{80} + \frac{\pi^4}{800} + \frac{1}{6} \right) \\
& + \delta_{ef} \lambda_{\alpha\beta\gamma c} \lambda_{\beta\gamma\epsilon b} \lambda_{d\delta\epsilon a} \lambda_{h\alpha\delta g} \left( -\frac{27}{10}\zeta_3^2 - \frac{9\zeta_3}{10} + \frac{51\zeta_5}{10} + \frac{\pi^6}{315} + \frac{\pi^4}{40} \right) \\
& + \delta_{ef} \lambda_{\alpha\beta\gamma b} \lambda_{\beta\gamma\epsilon c} \lambda_{d\delta\epsilon a} \lambda_{h\alpha\delta g} \left( \frac{23\zeta_3^2}{10} - \frac{9\zeta_3}{10} + \frac{41\zeta_5}{10} + \frac{\pi^6}{1890} + \frac{\pi^4}{40} \right) \\
& + \delta_{af} \lambda_{\alpha\beta\gamma b} \lambda_{\beta\gamma\epsilon c} \lambda_{e\delta\epsilon d} \lambda_{h\alpha\delta g} \left( \frac{17\zeta_3}{20} + \frac{3\zeta_5}{20} + \frac{\pi^4}{400} - \frac{2}{5} \right) \\
& + \delta_{ae} \lambda_{\alpha\beta\gamma b} \lambda_{\beta\gamma\epsilon c} \lambda_{f\delta\epsilon d} \lambda_{h\alpha\delta g} \left( \frac{47\zeta_3}{10} + \frac{7\zeta_5}{5} - \frac{13\pi^4}{600} + \frac{11}{5} \right) \\
& + \delta_{bf} \lambda_{\alpha\beta\gamma e} \lambda_{\beta\gamma\epsilon c} \lambda_{d\delta\epsilon a} \lambda_{h\alpha\delta g} \left( -\frac{12\zeta_3}{5} - \frac{17\zeta_5}{10} - \frac{\pi^4}{300} + \frac{227}{30} \right) \\
& + \lambda_{\alpha\beta\gamma f} \lambda_{c\beta\gamma b} \lambda_{de\delta a} \lambda_{h\alpha\delta g} \left( \frac{7\zeta_3}{5} + \frac{3\zeta_5}{10} + \frac{\pi^4}{300} - 1 \right) \\
& + \delta_{af} \lambda_{\alpha\beta\gamma c} \lambda_{\alpha\delta\epsilon b} \lambda_{e\delta\epsilon d} \lambda_{h\beta\gamma g} \left( \frac{3\zeta_3}{20} - \frac{\pi^4}{400} - \frac{11}{40} \right) \\
& + \delta_{ae} \lambda_{\alpha\beta\gamma c} \lambda_{\alpha\delta\epsilon b} \lambda_{f\delta\epsilon d} \lambda_{h\beta\gamma g} \left( \frac{17\zeta_3}{20} + \frac{89\zeta_5}{40} + \frac{\pi^4}{400} - \frac{5}{8} \right) \\
& + \delta_{af} \lambda_{\alpha\beta\delta b} \lambda_{\alpha\beta\gamma c} \lambda_{e\delta\epsilon d} \lambda_{h\gamma\epsilon g} \left( -\frac{\zeta_3}{10} - \frac{31\zeta_5}{20} - \frac{\pi^4}{300} + \frac{17}{20} \right) \\
& + \delta_{ae} \lambda_{\alpha\beta\delta b} \lambda_{\alpha\beta\gamma c} \lambda_{f\delta\epsilon d} \lambda_{h\gamma\epsilon g} \left( \frac{23\zeta_3}{5} + \frac{17\zeta_5}{10} - \frac{\pi^4}{75} + \frac{11}{5} \right) \\
& + \delta_{ef} \lambda_{\alpha\beta\gamma b} \lambda_{\alpha\beta\gamma c} \lambda_{d\delta\epsilon a} \lambda_{h\delta\epsilon g} \left( \frac{\zeta_3}{12} - \frac{\pi^4}{2880} - \frac{319}{7680} \right) \\
& + \delta_{af} \lambda_{\alpha\beta\gamma b} \lambda_{\alpha\beta\gamma c} \lambda_{e\delta\epsilon d} \lambda_{h\delta\epsilon g} \left( -\frac{\zeta_3}{40} + \frac{17\pi^4}{28800} - \frac{661}{15360} \right) \\
& + \lambda_{\alpha\beta\delta a} \lambda_{\alpha\beta\gamma g} \lambda_{de\delta b} \lambda_{fh\gamma c} \left( \frac{\zeta_3}{5} - \frac{9\zeta_5}{40} + \frac{13\pi^4}{1200} - 1 \right) \\
& + \lambda_{\alpha\beta\gamma a} \lambda_{\alpha\beta\gamma g} \lambda_{de\delta b} \lambda_{fh\delta c} \left( -\frac{7\zeta_3}{120} + \frac{\pi^4}{3600} - \frac{81}{5120} \right) \\
& + \lambda_{\alpha\beta\gamma g} \lambda_{de\delta b} \lambda_{f\beta\gamma c} \lambda_{h\alpha\delta a} \left( -\frac{29\zeta_3}{10} - \frac{15\zeta_5}{4} + \frac{73}{10} \right) \\
& + \lambda_{\alpha\beta\gamma g} \lambda_{de\delta b} \lambda_{f\gamma\delta c} \lambda_{h\alpha\beta a} \left( \frac{16\zeta_3}{5} + \frac{17\zeta_5}{10} - \frac{\pi^4}{100} - \frac{13}{10} \right) \\
& + \delta_{ef} \lambda_{\alpha\beta\gamma g} \lambda_{\alpha\delta\epsilon b} \lambda_{d\delta\epsilon a} \lambda_{h\beta\gamma c} \left( -\frac{\zeta_3}{5} - \frac{17\zeta_5}{10} - \frac{\pi^4}{150} + \frac{71}{15} \right) \\
& + \delta_{ef} \lambda_{\alpha\beta\delta b} \lambda_{\alpha\beta\gamma g} \lambda_{d\delta\epsilon a} \lambda_{h\gamma\epsilon c} \left( \frac{2\zeta_3^2}{5} - \frac{1}{75}\pi^4\zeta_3 - 26\zeta_5 + \frac{359\zeta_7}{10} - \frac{\pi^6}{189} \right) \\
& + \delta_{ef} \lambda_{\alpha\beta\gamma b} \lambda_{\alpha\beta\gamma g} \lambda_{d\delta\epsilon a} \lambda_{h\delta\epsilon c} \left( -\frac{\zeta_3}{2} + \frac{\pi^4}{720} - \frac{2767}{23040} \right) \\
& + \delta_{ef} \lambda_{\alpha\beta\gamma c} \lambda_{\alpha\beta\gamma g} \lambda_{d\delta\epsilon a} \lambda_{h\delta\epsilon b} \left( -\frac{14167}{46080} \right)
\end{aligned}$$

$$\begin{aligned}
& + \lambda_{\alpha\beta\gamma g} \lambda_{\beta\gamma\delta c} \lambda_{defb} \lambda_{h\alpha\delta a} \left( -\frac{6\zeta_3}{5} - \frac{9\zeta_5}{2} - \frac{\pi^4}{100} + \frac{73}{10} \right) \\
& + \delta_{ef} \lambda_{\alpha\beta\gamma g} \lambda_{\alpha\delta\epsilon b} \lambda_{\beta\gamma\delta c} \lambda_{dh\epsilon a} \left( -\frac{27}{4}\zeta_3^2 - \frac{27\zeta_3}{2} + \frac{81\zeta_5}{5} + \frac{\pi^6}{630} \right) \\
& + \delta_{ef} \lambda_{\alpha\beta\gamma g} \lambda_{\beta\gamma\epsilon c} \lambda_{d\delta\epsilon a} \lambda_{h\alpha\delta b} \left( \frac{31\zeta_3^2}{5} + \frac{1}{30}\pi^4\zeta_3 - 13\zeta_5 + \frac{23\zeta_7}{20} - \frac{\pi^6}{378} \right) \\
& + \delta_{ef} \lambda_{\alpha\beta\gamma g} \lambda_{d\delta\epsilon a} \lambda_{\gamma\delta\epsilon c} \lambda_{h\alpha\beta b} \left( \frac{101\zeta_3}{20} - \frac{63\zeta_5}{20} - \frac{13\pi^4}{1200} - \frac{6}{5} \right) \\
& + \lambda_{\alpha\beta\gamma g} \lambda_{cf\beta b} \lambda_{e\gamma\delta d} \lambda_{h\alpha\delta a} \left( \frac{44\zeta_3^2}{5} - \frac{4}{75}\pi^4\zeta_3 - 26\zeta_5 + \frac{71\zeta_7}{40} - \frac{\pi^6}{189} \right) \\
& + \lambda_{\alpha\beta\gamma g} \lambda_{cf\delta b} \lambda_{e\gamma\delta d} \lambda_{h\alpha\beta a} \left( \frac{13\zeta_3}{5} + \frac{7\zeta_5}{10} - \frac{\pi^4}{150} - \frac{12}{5} \right) \\
& + \delta_{af} \lambda_{\alpha\beta\gamma c} \lambda_{\alpha\beta\gamma g} \lambda_{e\delta\epsilon d} \lambda_{h\delta\epsilon b} \left( -\frac{\zeta_3}{120} - \frac{17\pi^4}{14400} + \frac{221}{1536} \right) \\
& + \delta_{af} \lambda_{\alpha\beta\gamma g} \lambda_{\beta\gamma\epsilon c} \lambda_{e\delta\epsilon d} \lambda_{h\alpha\delta b} \left( -\frac{53\zeta_3}{10} - \frac{3\zeta_5}{10} + \frac{\pi^4}{600} + \frac{11}{5} \right) \\
& + \delta_{ae} \lambda_{\alpha\beta\gamma b} \lambda_{\alpha\beta\gamma g} \lambda_{f\delta\epsilon d} \lambda_{h\delta\epsilon c} \left( \frac{3\zeta_3}{20} - \frac{\pi^4}{2400} + \frac{1529}{23040} \right) \\
& + \delta_{ae} \lambda_{\alpha\beta\gamma c} \lambda_{\alpha\beta\gamma g} \lambda_{f\delta\epsilon d} \lambda_{h\delta\epsilon b} \left( -\frac{13\zeta_3}{20} + \frac{\pi^4}{1200} + \frac{1127}{7680} \right) \\
& + \delta_{ae} \lambda_{\alpha\beta\gamma g} \lambda_{\beta\gamma\epsilon c} \lambda_{f\delta\epsilon d} \lambda_{h\alpha\delta b} \left( -\frac{81}{10}\zeta_3^2 - \frac{96\zeta_3}{5} + \frac{162\zeta_5}{5} - \frac{\pi^6}{315} - \frac{\pi^4}{100} \right) \\
& + \delta_{ae} \lambda_{\alpha\beta\gamma g} \lambda_{f\delta\epsilon d} \lambda_{\gamma\delta\epsilon c} \lambda_{h\alpha\beta b} \left( -\frac{39\zeta_3}{10} - 2\zeta_5 + \frac{\pi^4}{200} + \frac{23}{5} \right) \\
& + \lambda_{\alpha\beta\delta g} \lambda_{\alpha\beta\gamma a} \lambda_{de\delta b} \lambda_{fh\gamma c} \left( -\frac{9\zeta_3}{20} + \frac{7\zeta_5}{20} - \frac{\pi^4}{1200} + \frac{61}{60} \right) \\
& + \lambda_{\alpha\beta\delta g} \lambda_{de\delta b} \lambda_{f\beta\gamma c} \lambda_{h\alpha\gamma a} \left( -\frac{48}{5}\zeta_3^2 + \frac{63\zeta_3}{5} + \frac{66\zeta_5}{5} - \frac{\pi^6}{210} - \frac{\pi^4}{300} \right) \\
& + \delta_{ef} \lambda_{\alpha\beta\delta g} \lambda_{\alpha\gamma\epsilon b} \lambda_{d\delta\epsilon a} \lambda_{h\beta\gamma c} \left( \frac{162\zeta_{35}}{25} + 18\zeta_3\zeta_5 - \frac{1323\zeta_7}{20} - \frac{2063\pi^8}{210000} \right) \\
& + \delta_{ef} \lambda_{\alpha\beta\delta g} \lambda_{\alpha\beta\gamma b} \lambda_{d\delta\epsilon a} \lambda_{h\gamma\epsilon c} \left( \frac{32\zeta_3^2}{5} + \frac{2}{75}\pi^4\zeta_3 - 26\zeta_5 + \frac{1443\zeta_7}{40} - \frac{\pi^6}{189} \right) \\
& + \delta_{ef} \lambda_{\alpha\beta\delta g} \lambda_{\alpha\beta\gamma c} \lambda_{d\delta\epsilon a} \lambda_{h\gamma\epsilon b} \left( \frac{46\zeta_3^2}{5} + \frac{4}{75}\pi^4\zeta_3 - 13\zeta_5 - \frac{377\zeta_7}{80} - \frac{\pi^6}{378} \right) \\
& + \delta_{ef} \lambda_{\alpha\beta\delta g} \lambda_{\beta\gamma\epsilon c} \lambda_{d\delta\epsilon a} \lambda_{h\alpha\gamma b} \left( \frac{81\zeta_{35}}{25} + 27\zeta_3\zeta_5 - \frac{1323\zeta_7}{40} - \frac{2063\pi^8}{420000} \right) \\
& + \delta_{af} \lambda_{\alpha\beta\delta g} \lambda_{\alpha\beta\gamma c} \lambda_{e\delta\epsilon d} \lambda_{h\gamma\epsilon b} \left( 3\zeta_3 + \frac{31\zeta_5}{10} - \frac{\pi^4}{150} - \frac{46}{15} \right) \\
& + \delta_{af} \lambda_{\alpha\beta\delta g} \lambda_{\beta\gamma\epsilon c} \lambda_{e\delta\epsilon d} \lambda_{h\alpha\gamma b} (-42) \\
& + \delta_{ae} \lambda_{\alpha\beta\delta g} \lambda_{\alpha\beta\gamma b} \lambda_{fh\epsilon d} \lambda_{\gamma\delta\epsilon c} \left( \frac{21\zeta_3}{10} - \frac{39\zeta_5}{10} - \frac{7\pi^4}{200} + \frac{11}{5} \right) \\
& + \delta_{ae} \lambda_{\alpha\beta\delta g} \lambda_{\alpha\beta\gamma b} \lambda_{f\delta\epsilon d} \lambda_{h\gamma\epsilon c} \left( \frac{187\zeta_3^2}{10} - \frac{96\zeta_3}{5} + \frac{62\zeta_5}{5} - \frac{8\pi^6}{945} - \frac{\pi^4}{100} \right) \\
& + \delta_{ae} \lambda_{\alpha\beta\delta g} \lambda_{\alpha\beta\gamma c} \lambda_{f\delta\epsilon d} \lambda_{h\gamma\epsilon b} \left( -\frac{179}{10}\zeta_3^2 - \frac{96\zeta_3}{5} + \frac{212\zeta_5}{5} - \frac{\pi^6}{1890} - \frac{\pi^4}{100} \right) \\
& + \delta_{ae} \lambda_{\alpha\beta\delta g} \lambda_{\beta\gamma\epsilon c} \lambda_{f\delta\epsilon d} \lambda_{h\alpha\gamma b} \left( \frac{16\zeta_3^2}{5} + \frac{1}{75}\pi^4\zeta_3 - 64\zeta_5 + \frac{761\zeta_7}{10} - \frac{8\pi^6}{189} \right) \\
& + \delta_{ef} \lambda_{\alpha\beta\epsilon g} \lambda_{\alpha\gamma\delta b} \lambda_{\beta\gamma\delta c} \lambda_{dh\epsilon a} \left( \frac{137\zeta_3^2}{10} - 27\zeta_3 + \frac{92\zeta_5}{5} - \frac{\pi^6}{135} \right) \\
& + \lambda_{\alpha\gamma\delta g} \lambda_{cf\beta b} \lambda_{e\gamma\delta d} \lambda_{h\alpha\beta a} \left( -\frac{5}{2}\zeta_3^2 - \frac{9\zeta_3}{10} - \frac{79\zeta_5}{10} + \frac{\pi^6}{1890} + \frac{\pi^4}{40} \right)
\end{aligned}$$

$$\begin{aligned}
& + \delta_{ae} \lambda_{\alpha\beta\epsilon b} \lambda_{\alpha\gamma\delta g} \lambda_{\beta\gamma\delta c} \lambda_{fh\epsilon d} \left( -\frac{18\zeta_3}{5} + 3\zeta_5 - \frac{\pi^4}{50} + \frac{11}{5} \right) \\
& + \delta_{ae} \lambda_{\alpha\beta\delta b} \lambda_{\alpha\gamma\epsilon g} \lambda_{f\delta\epsilon d} \lambda_{h\beta\gamma c} \left( \frac{56\zeta_3^2}{5} + \frac{7}{150} \pi^4 \zeta_3 - 32\zeta_5 + \frac{153\zeta_7}{10} - \frac{4\pi^6}{189} \right) \\
& + \delta_{ef} \lambda_{\alpha\beta\gamma b} \lambda_{\alpha\delta\epsilon g} \lambda_{d\delta\epsilon a} \lambda_{h\beta\gamma c} \left( -\frac{26}{5} \zeta_3^2 - \frac{9\zeta_3}{10} + \frac{58\zeta_5}{5} - \frac{13\pi^6}{3780} + \frac{\pi^4}{40} \right) \\
& + \delta_{ef} \lambda_{\alpha\beta\gamma c} \lambda_{\alpha\delta\epsilon g} \lambda_{d\delta\epsilon a} \lambda_{h\beta\gamma b} \left( -\frac{31}{5} \zeta_3^2 - \frac{9\zeta_3}{20} + \frac{44\zeta_5}{5} - \frac{13\pi^6}{7560} + \frac{\pi^4}{80} \right) \\
& + \delta_{af} \lambda_{\alpha\beta\gamma c} \lambda_{\alpha\delta\epsilon g} \lambda_{e\delta\epsilon d} \lambda_{h\beta\gamma b} \left( -\frac{3\zeta_3}{5} + \frac{\pi^4}{100} + \frac{61}{60} \right) \\
& + \delta_{ae} \lambda_{\alpha\beta\gamma b} \lambda_{\alpha\delta\epsilon g} \lambda_{\beta\gamma\delta c} \lambda_{fh\epsilon d} \left( \frac{9\zeta_3}{2} + 3\zeta_5 - \frac{\pi^4}{200} - \frac{12}{5} \right) \\
& + \delta_{ae} \lambda_{\alpha\beta\gamma b} \lambda_{\alpha\delta\epsilon g} \lambda_{f\delta\epsilon d} \lambda_{h\beta\gamma c} \left( \frac{13\zeta_3}{5} + \frac{13\zeta_5}{10} - \frac{2\pi^4}{75} + \frac{11}{5} \right) \\
& + \delta_{ae} \lambda_{\alpha\beta\gamma c} \lambda_{\alpha\delta\epsilon g} \lambda_{f\delta\epsilon d} \lambda_{h\beta\gamma b} \left( \frac{117\zeta_3}{10} - 11\zeta_5 - \frac{\pi^4}{40} + \frac{11}{5} \right) \\
& + \delta_{af} \delta_{eg} \lambda_{\alpha\beta\gamma c} \lambda_{\alpha\beta\gamma h} \lambda_{\delta\epsilon\zeta b} \lambda_{\delta\epsilon\zeta d} \left( \frac{1}{96} \right) \\
& + \delta_{af} \delta_{eg} \lambda_{\alpha\beta\gamma h} \lambda_{\alpha\delta\epsilon b} \lambda_{\beta\gamma\zeta c} \lambda_{\delta\epsilon\zeta d} \left( \frac{57\zeta_3}{5} - \frac{167\zeta_5}{20} - \frac{19\pi^4}{600} - \frac{46}{15} \right) \\
& + \delta_{af} \delta_{eg} \lambda_{\alpha\beta\delta b} \lambda_{\alpha\beta\gamma h} \lambda_{\delta\epsilon\zeta d} \lambda_{\gamma\epsilon\zeta c} \left( -\frac{33\zeta_3}{10} + \frac{7\zeta_5}{5} + \frac{\pi^4}{600} + \frac{13}{3} \right) \\
& + \delta_{cf} \delta_{dg} \lambda_{\alpha\beta\delta e} \lambda_{\alpha\beta\gamma h} \lambda_{\delta\epsilon\zeta b} \lambda_{\gamma\epsilon\zeta a} \left( -\frac{11}{60} \right) \\
& + \delta_{cf} \delta_{dg} \lambda_{\alpha\beta\gamma h} \lambda_{\alpha\delta\epsilon e} \lambda_{\beta\gamma\zeta a} \lambda_{\delta\epsilon\zeta b} \left( \frac{\zeta_3}{20} + \frac{9\zeta_5}{80} - \frac{\pi^4}{800} - \frac{1}{20} \right) \\
& + \delta_{cf} \delta_{dg} \lambda_{\alpha\beta\gamma a} \lambda_{\alpha\beta\gamma h} \lambda_{\delta\epsilon\zeta b} \lambda_{\delta\epsilon\zeta e} \left( \frac{\zeta_3}{144} - \frac{7}{3072} \right) \\
& + \delta_{af} \delta_{eg} \lambda_{\alpha\beta\delta h} \lambda_{\alpha\beta\gamma c} \lambda_{\delta\epsilon\zeta d} \lambda_{\gamma\epsilon\zeta b} \left( \frac{36\zeta_3}{5} - \frac{7\zeta_5}{2} - \frac{3\pi^4}{100} - \frac{46}{15} \right) \\
& + \delta_{af} \delta_{eg} \lambda_{\alpha\beta\delta h} \lambda_{\alpha\gamma\epsilon b} \lambda_{\beta\gamma\zeta c} \lambda_{\delta\epsilon\zeta d} \left( \frac{159\zeta_3^2}{10} - 33\zeta_3 + \frac{138\zeta_5}{5} + \frac{2\pi^6}{315} - \frac{2\pi^4}{15} \right) \\
& + \delta_{cf} \delta_{dg} \lambda_{\alpha\beta\delta h} \lambda_{\alpha\gamma\epsilon e} \lambda_{\beta\gamma\zeta a} \lambda_{\delta\epsilon\zeta b} \left( -\frac{9}{40} \zeta_3^2 + \frac{33\zeta_3}{20} + \frac{3\zeta_5}{2} - \frac{\pi^6}{1260} + \frac{\pi^4}{200} \right) \\
& + \delta_{cf} \delta_{dg} \lambda_{\alpha\beta\delta h} \lambda_{\alpha\beta\gamma a} \lambda_{\delta\epsilon\zeta b} \lambda_{\gamma\epsilon\zeta e} \left( \frac{\zeta_3}{20} - \frac{11\zeta_5}{40} - \frac{1}{20} \right) \\
& + \delta_{ef} \lambda_{\alpha\beta\delta h} \lambda_{\alpha\beta\gamma g} \lambda_{c\gamma\epsilon b} \lambda_{d\delta\epsilon a} \left( \frac{15\zeta_3^2}{4} - \frac{27\zeta_3}{2} + \frac{6\zeta_5}{5} + \frac{\pi^6}{180} \right) \\
& + \lambda_{\alpha\beta\delta h} \lambda_{\alpha\beta\gamma g} \lambda_{c\gamma\delta a} \lambda_{de\epsilon b} \left( \frac{3\zeta_3}{2} + 3\zeta_5 + \frac{\pi^4}{100} - \frac{14}{3} \right) \\
& + \lambda_{\alpha\beta\delta h} \lambda_{\alpha\beta\gamma g} \lambda_{cf\gamma a} \lambda_{de\delta b} \left( \frac{7\zeta_3}{5} - \frac{17\zeta_5}{5} - \frac{\pi^4}{100} + \frac{73}{10} \right) \\
& + \delta_{ef} \lambda_{\alpha\beta\delta h} \lambda_{\alpha\beta\gamma g} \lambda_{cd\epsilon a} \lambda_{\gamma\delta\epsilon b} \left( \frac{\zeta_3}{5} + \frac{53\zeta_5}{20} + \frac{\pi^4}{60} - \frac{14}{3} \right) \\
& + \delta_{ae} \lambda_{\alpha\beta\delta h} \lambda_{\alpha\beta\gamma g} \lambda_{df\epsilon b} \lambda_{\gamma\delta\epsilon c} \left( -\frac{72\zeta_3}{5} - 3\zeta_5 - \frac{\pi^4}{50} + \frac{184}{15} \right) \\
& + \delta_{af} \lambda_{\alpha\beta\delta h} \lambda_{\alpha\beta\gamma g} \lambda_{c\gamma\epsilon b} \lambda_{e\delta\epsilon d} \left( -\frac{51\zeta_3}{10} - \frac{17\zeta_5}{10} + \frac{3\pi^4}{200} + \frac{23}{5} \right) \\
& + \delta_{ae} \lambda_{\alpha\beta\delta h} \lambda_{\alpha\beta\gamma g} \lambda_{c\gamma\epsilon b} \lambda_{f\delta\epsilon d} \left( \frac{74\zeta_3}{5} + \frac{17\zeta_5}{5} + \frac{\pi^4}{25} - 42 \right) \\
& + \delta_{af} \delta_{be} \lambda_{\alpha\beta\delta h} \lambda_{\alpha\beta\gamma g} \lambda_{\delta\epsilon\zeta d} \lambda_{\gamma\epsilon\zeta c} \left( -\frac{\zeta_3}{40} + \frac{3\zeta_5}{40} + \frac{\pi^4}{480} - \frac{3}{4} \right)
\end{aligned}$$

$$\begin{aligned}
& + \delta_{bf} \lambda_{\alpha\beta\delta h} \lambda_{\alpha\beta\gamma g} \lambda_{cd\epsilon a} \lambda_{\gamma\delta\epsilon e} \left( -\frac{3\zeta_3}{2} - \frac{3\zeta_5}{2} + \frac{17}{15} \right) \\
& + \delta_{ef} \lambda_{\alpha\beta\delta g} \lambda_{\alpha\gamma\epsilon h} \lambda_{c\beta\gamma b} \lambda_{d\delta\epsilon a} \left( -\frac{162}{5} \zeta_3^2 - \frac{3}{25} \pi^4 \zeta_3 + \frac{189\zeta_7}{5} \right) \\
& + \delta_{af} \lambda_{\alpha\beta\delta g} \lambda_{\alpha\gamma\epsilon h} \lambda_{c\beta\gamma b} \lambda_{e\delta\epsilon d} \left( \frac{69\zeta_3^2}{20} - \frac{48\zeta_3}{5} + \frac{6\zeta_5}{5} - \frac{\pi^6}{180} - \frac{\pi^4}{200} \right) \\
& + \delta_{ae} \lambda_{\alpha\beta\delta g} \lambda_{\alpha\gamma\epsilon h} \lambda_{c\beta\gamma b} \lambda_{f\delta\epsilon d} \left( -\frac{81}{10} \zeta_3^2 - 33\zeta_3 + \frac{138\zeta_5}{5} + \frac{2\pi^6}{315} - \frac{2\pi^4}{15} \right) \\
& + \delta_{af} \delta_{be} \lambda_{\alpha\beta\delta g} \lambda_{\alpha\gamma\epsilon h} \lambda_{\beta\gamma\zeta c} \lambda_{\delta\epsilon\zeta d} \left( -\frac{57}{10} \zeta_3^2 + \frac{5\zeta_3}{2} + \frac{16\zeta_5}{5} + \frac{\pi^6}{840} - \frac{\pi^4}{100} \right) \\
& + \delta_{ef} \lambda_{\alpha\beta\gamma g} \lambda_{\alpha\delta\epsilon h} \lambda_{c\beta\gamma b} \lambda_{d\delta\epsilon a} \left( -\frac{93}{20} \zeta_3^2 - \frac{9\zeta_3}{20} + \frac{141\zeta_5}{20} - \frac{\pi^6}{420} + \frac{\pi^4}{80} \right) \\
& + \delta_{ef} \lambda_{\alpha\beta\gamma g} \lambda_{\alpha\delta\epsilon h} \lambda_{\beta\gamma\delta b} \lambda_{cd\epsilon a} \left( -\frac{33\zeta_3}{10} - \frac{19\zeta_5}{20} - \frac{\pi^4}{50} + \frac{73}{10} \right) \\
& + \delta_{ae} \lambda_{\alpha\beta\gamma g} \lambda_{\alpha\delta\epsilon h} \lambda_{\beta\gamma\delta c} \lambda_{df\epsilon b} \left( \frac{182\zeta_3}{5} - \frac{64\zeta_5}{5} + \frac{\pi^4}{50} - 42 \right) \\
& + \delta_{af} \lambda_{\alpha\beta\gamma g} \lambda_{\alpha\delta\epsilon h} \lambda_{c\beta\gamma b} \lambda_{e\delta\epsilon d} \left( \frac{19\zeta_3}{20} + \frac{77\zeta_5}{40} - \frac{\pi^4}{400} - \frac{5}{8} \right) \\
& + \delta_{ae} \lambda_{\alpha\beta\gamma g} \lambda_{\alpha\delta\epsilon h} \lambda_{c\beta\gamma b} \lambda_{f\delta\epsilon d} \left( -\frac{29\zeta_3}{10} - \frac{15\zeta_5}{4} + \frac{73}{10} \right) \\
& + \delta_{af} \delta_{be} \lambda_{\alpha\beta\gamma g} \lambda_{\alpha\delta\epsilon h} \lambda_{\beta\gamma\zeta c} \lambda_{\delta\epsilon\zeta d} \left( -\frac{14\zeta_3}{5} + \frac{17\zeta_5}{8} + \frac{\pi^4}{600} + \frac{17}{10} \right) \\
& + \delta_{bf} \lambda_{\alpha\beta\gamma g} \lambda_{\alpha\delta\epsilon h} \lambda_{\beta\gamma\delta e} \lambda_{cd\epsilon a} \left( \frac{21\zeta_3}{10} - \frac{21\zeta_5}{10} + \frac{3\pi^4}{200} - \frac{7}{10} \right) \\
& + \delta_{eg} \lambda_{\alpha\beta\gamma a} \lambda_{\alpha\delta\epsilon b} \lambda_{\beta\gamma\delta h} \lambda_{df\epsilon c} \left( \frac{19\zeta_3}{10} + \frac{7\zeta_5}{20} - \frac{\pi^4}{200} - \frac{17}{20} \right) \\
& + \delta_{ae} \lambda_{\alpha\beta\epsilon b} \lambda_{\alpha\gamma\delta g} \lambda_{\beta\gamma\delta h} \lambda_{df\epsilon c} \left( \frac{12\zeta_3}{5} + \frac{3\zeta_5}{2} + \frac{\pi^4}{200} - \frac{79}{30} \right) \\
& + \delta_{ae} \lambda_{\alpha\beta\delta g} \lambda_{\alpha\beta\gamma b} \lambda_{df\epsilon c} \lambda_{\gamma\delta\epsilon h} \left( -\frac{27\zeta_3}{5} + \frac{32\zeta_5}{5} - \frac{7\pi^4}{300} + \frac{227}{30} \right) \\
& + \delta_{af} \delta_{be} \lambda_{\alpha\beta\delta g} \lambda_{\alpha\beta\gamma c} \lambda_{\delta\epsilon\zeta d} \lambda_{\gamma\epsilon\zeta h} \left( -\frac{19\zeta_3}{5} + \frac{97\zeta_5}{40} + \frac{\pi^4}{300} + \frac{17}{10} \right) \\
& + \delta_{af} \delta_{be} \lambda_{\alpha\beta\gamma c} \lambda_{\alpha\beta\gamma g} \lambda_{\delta\epsilon\zeta d} \lambda_{\delta\epsilon\zeta h} \left( \frac{5}{9216} \right) \\
& + \delta_{eg} \lambda_{\alpha\beta\epsilon a} \lambda_{\beta\gamma\delta\alpha} \lambda_{df\epsilon c} \lambda_{h\gamma\delta b} \left( -\frac{21\zeta_3}{20} - \frac{7\zeta_5}{10} + \frac{\pi^4}{150} - \frac{67}{120} \right) \\
& + \lambda_{\beta\gamma\delta\alpha} \lambda_{de\delta b} \lambda_{f\beta\gamma c} \lambda_{gh\alpha a} \left( \frac{9\zeta_3}{20} - \frac{7\zeta_5}{20} + \frac{\pi^4}{300} - \frac{11}{15} \right) \\
& + \delta_{ef} \lambda_{\alpha\beta\epsilon b} \lambda_{\beta\gamma\delta\alpha} \lambda_{dh\epsilon a} \lambda_{g\gamma\delta c} \left( \frac{3\zeta_3^2}{20} - \frac{9\zeta_3}{20} + \frac{21\zeta_5}{20} - \frac{\pi^6}{420} + \frac{\pi^4}{80} \right) \\
& + \delta_{ef} \lambda_{\alpha\beta\gamma b} \lambda_{\beta\gamma\delta\alpha} \lambda_{dh\epsilon a} \lambda_{g\delta\epsilon c} \left( -\frac{13\zeta_3}{16} - \frac{7\zeta_5}{24} + \frac{\pi^4}{240} \right) \\
& + \delta_{ef} \lambda_{\beta\gamma\delta\alpha} \lambda_{d\delta\epsilon a} \lambda_{g\alpha\epsilon b} \lambda_{h\beta\gamma c} \left( \frac{31\zeta_3^2}{5} + \frac{1}{30} \pi^4 \zeta_3 - 13\zeta_5 - \frac{117\zeta_7}{20} - \frac{\pi^6}{378} \right) \\
& + \delta_{ef} \lambda_{\beta\gamma\delta\alpha} \lambda_{\beta\gamma\delta c} \lambda_{dh\epsilon a} \lambda_{g\alpha\epsilon b} \left( \frac{151\zeta_3}{40} + \frac{37\zeta_5}{60} + \frac{\pi^4}{300} \right) \\
& + \delta_{ef} \lambda_{\beta\gamma\delta\alpha} \lambda_{dh\epsilon a} \lambda_{g\alpha\beta b} \lambda_{\gamma\delta\epsilon c} \left( -\frac{19}{10} \zeta_3^2 - \frac{9\zeta_3}{10} + \frac{71\zeta_5}{10} - \frac{\pi^6}{135} + \frac{\pi^4}{40} \right) \\
& + \lambda_{\beta\gamma\delta\alpha} \lambda_{c\gamma\delta a} \lambda_{eghd} \lambda_{f\alpha\beta b} \left( \frac{3}{10} - \frac{21\zeta_5}{40} \right) \\
& + \lambda_{\beta\gamma\delta\alpha} \lambda_{c\beta\gamma a} \lambda_{eh\delta d} \lambda_{fg\alpha b} \left( -\frac{3\zeta_3}{10} + \frac{\zeta_5}{5} - \frac{\pi^4}{600} + \frac{61}{60} \right)
\end{aligned}$$

$$\begin{aligned}
& + \lambda_{\beta\gamma\delta\alpha}\lambda_{cg\gamma a}\lambda_{eh\delta d}\lambda_{f\alpha\beta b}\left(-\frac{37}{10}\zeta_3^2 - \frac{9\zeta_3}{10} + \frac{101\zeta_5}{10} + \frac{\pi^6}{1890} + \frac{\pi^4}{40}\right) \\
& + \lambda_{\alpha\beta\gamma b}\lambda_{\beta\gamma\delta\alpha}\lambda_{cfga}\lambda_{eh\delta d}\left(-\frac{319}{7680}\right) \\
& + \lambda_{\beta\gamma\delta\alpha}\lambda_{ch\beta a}\lambda_{e\gamma\delta d}\lambda_{fg\alpha b}\left(\frac{9\zeta_3}{20} + \frac{7\zeta_5}{20} + \frac{\pi^4}{240} + \frac{61}{60}\right) \\
& + \lambda_{\beta\gamma\delta\alpha}\lambda_{cgha}\lambda_{e\gamma\delta d}\lambda_{f\alpha\beta b}\left(\frac{17\zeta_3}{40} - \frac{9\zeta_5}{40} - \frac{\pi^4}{800} + \frac{7}{40}\right) \\
& + \delta_{ae}\lambda_{\alpha\beta\epsilon b}\lambda_{\beta\gamma\delta\alpha}\lambda_{fh\epsilon d}\lambda_{g\gamma\delta c}\left(\frac{19\zeta_3}{20} - \frac{43\zeta_5}{40} - \frac{\pi^4}{400} - \frac{5}{8}\right) \\
& + \delta_{ae}\lambda_{\alpha\beta\gamma b}\lambda_{\beta\gamma\delta\alpha}\lambda_{fh\epsilon d}\lambda_{g\delta\epsilon c}\left(-\frac{2767}{23040}\right) \\
& + \delta_{ae}\lambda_{\beta\gamma\delta\alpha}\lambda_{\beta\gamma\delta c}\lambda_{fh\epsilon d}\lambda_{g\alpha\epsilon b}\left(\frac{1127}{7680}\right) \\
& + \delta_{ae}\lambda_{\beta\gamma\delta\alpha}\lambda_{fh\epsilon d}\lambda_{g\alpha\beta b}\lambda_{\gamma\delta\epsilon c}\left(\frac{21\zeta_3}{20} - \frac{3\zeta_5}{8} - \frac{3\pi^4}{400} - \frac{5}{8}\right) \\
& + \delta_{ae}\lambda_{\beta\gamma\delta\alpha}\lambda_{f\delta\epsilon d}\lambda_{g\alpha\epsilon b}\lambda_{h\beta\gamma c}\left(-\frac{179}{10}\zeta_3^2 - \frac{96\zeta_3}{5} + \frac{212\zeta_5}{5} - \frac{\pi^6}{1890} - \frac{\pi^4}{100}\right) \\
& + \delta_{ae}\lambda_{\beta\gamma\delta\alpha}\lambda_{f\delta\epsilon d}\lambda_{g\alpha\beta b}\lambda_{h\gamma\epsilon c}\left(\frac{309\zeta_3^2}{20} - \frac{48\zeta_3}{5} + \frac{6\zeta_5}{5} - \frac{\pi^6}{180} - \frac{\pi^4}{200}\right) \\
& + \lambda_{\beta\gamma\delta\alpha}\lambda_{c\gamma\delta a}\lambda_{dghb}\lambda_{f\alpha\beta e}\left(-\frac{27\zeta_3}{20} - \frac{\zeta_5}{4} + \frac{\pi^4}{1200} + \frac{61}{60}\right) \\
& + \lambda_{\beta\gamma\delta\alpha}\lambda_{cg\gamma a}\lambda_{dh\delta b}\lambda_{f\alpha\beta e}\left(\frac{67\zeta_3^2}{10} + \frac{1}{60}\pi^4\zeta_3 - \frac{13\zeta_5}{2} - \frac{26\zeta_7}{5} - \frac{\pi^6}{756}\right) \\
& + \lambda_{\alpha\beta\gamma e}\lambda_{\beta\gamma\delta\alpha}\lambda_{cf\delta a}\lambda_{dghb}\left(-\frac{10057}{11520}\right) \\
& + \delta_{ef}\lambda_{\beta\gamma\delta\alpha}\lambda_{c\gamma\epsilon b}\lambda_{d\delta\epsilon a}\lambda_{h\alpha\beta g}\left(-\frac{27}{20}\zeta_3^2 - \frac{9\zeta_3}{20} - \frac{129\zeta_5}{20} + \frac{\pi^6}{630} + \frac{\pi^4}{80}\right) \\
& + \delta_{ef}\lambda_{\beta\gamma\delta\alpha}\lambda_{cd\epsilon a}\lambda_{\gamma\delta\epsilon b}\lambda_{h\alpha\beta g}\left(\frac{7\zeta_3}{20} - \frac{3\zeta_5}{4} + \frac{\pi^4}{400} + \frac{7}{40}\right) \\
& + \delta_{ae}\lambda_{\beta\gamma\delta\alpha}\lambda_{df\epsilon b}\lambda_{\gamma\delta\epsilon c}\lambda_{h\alpha\beta g}\left(-\frac{31\zeta_3}{20} + \frac{9\zeta_5}{40} + \frac{\pi^4}{80} - \frac{5}{8}\right) \\
& + \delta_{af}\lambda_{\beta\gamma\delta\alpha}\lambda_{c\gamma\epsilon b}\lambda_{e\delta\epsilon d}\lambda_{h\alpha\beta g}\left(\frac{33\zeta_3}{20} + \frac{7\zeta_5}{40} - \frac{\pi^4}{240} - \frac{221}{120}\right) \\
& + \delta_{ae}\lambda_{\beta\gamma\delta\alpha}\lambda_{c\gamma\epsilon b}\lambda_{f\delta\epsilon d}\lambda_{h\alpha\beta g}\left(-\frac{27\zeta_3}{5} - \frac{7\zeta_5}{20} - \frac{7\pi^4}{600} - \frac{46}{15}\right) \\
& + \delta_{bf}\lambda_{\beta\gamma\delta\alpha}\lambda_{cd\epsilon a}\lambda_{\gamma\delta\epsilon e}\lambda_{h\alpha\beta g}\left(\frac{\zeta_3}{20} + \frac{9\zeta_5}{80} - \frac{\pi^4}{200} + \frac{23}{80}\right) \\
& + \delta_{ef}\lambda_{\beta\gamma\delta\alpha}\lambda_{c\beta\gamma b}\lambda_{d\delta\epsilon a}\lambda_{h\alpha\epsilon g}\left(\frac{23\zeta_3^2}{10} - \frac{9\zeta_3}{10} + \frac{41\zeta_5}{10} + \frac{\pi^6}{1890} + \frac{\pi^4}{40}\right) \\
& + \delta_{ef}\lambda_{\beta\gamma\delta\alpha}\lambda_{\beta\gamma\delta b}\lambda_{cd\epsilon a}\lambda_{h\alpha\epsilon g}\left(\frac{\zeta_3}{12} - \frac{\pi^4}{2880} - \frac{319}{7680}\right) \\
& + \delta_{ae}\lambda_{\beta\gamma\delta\alpha}\lambda_{\beta\gamma\delta c}\lambda_{df\epsilon b}\lambda_{h\alpha\epsilon g}\left(\frac{11\zeta_3}{60} - \frac{\pi^4}{1800} + \frac{1127}{7680}\right) \\
& + \delta_{af}\lambda_{\beta\gamma\delta\alpha}\lambda_{c\beta\gamma b}\lambda_{e\delta\epsilon d}\lambda_{h\alpha\epsilon g}\left(-\frac{19\zeta_3}{20} + \frac{7\zeta_5}{8} - \frac{\pi^4}{150} + \frac{17}{20}\right) \\
& + \delta_{ae}\lambda_{\beta\gamma\delta\alpha}\lambda_{c\beta\gamma b}\lambda_{f\delta\epsilon d}\lambda_{h\alpha\epsilon g}\left(-\frac{43\zeta_3}{10} - \frac{7\zeta_5}{20} + \frac{\pi^4}{100} + \frac{73}{10}\right) \\
& + \delta_{bf}\lambda_{\beta\gamma\delta\alpha}\lambda_{\beta\gamma\delta e}\lambda_{cd\epsilon a}\lambda_{h\alpha\epsilon g}\left(-\frac{3\zeta_3}{40} - \frac{\pi^4}{3600} + \frac{249}{5120}\right) \\
& + \delta_{ae}\lambda_{\alpha\beta\epsilon b}\lambda_{\beta\gamma\delta\alpha}\lambda_{df\epsilon c}\lambda_{h\gamma\delta g}\left(\frac{\zeta_3}{5} - \frac{9\zeta_5}{80} + \frac{\pi^4}{1200} + \frac{1}{16}\right)
\end{aligned}$$

$$\begin{aligned}
& + \delta_{ae} \lambda_{\alpha\beta\gamma b} \lambda_{\beta\gamma\delta\alpha} \lambda_{df\epsilon c} \lambda_{h\delta\epsilon g} \left( -\frac{7\zeta_3}{120} + \frac{\pi^4}{3600} - \frac{81}{5120} \right) \\
& + \lambda_{\alpha\beta\gamma g} \lambda_{\beta\gamma\delta\alpha} \lambda_{cfha} \lambda_{de\delta b} \left( -\frac{11\zeta_3}{60} - \frac{\pi^4}{1800} + \frac{221}{1536} \right) \\
& + \delta_{ef} \lambda_{\alpha\beta\gamma g} \lambda_{\beta\gamma\delta\alpha} \lambda_{cd\epsilon a} \lambda_{h\delta\epsilon b} \left( \frac{\zeta_3}{2} - \frac{\pi^4}{1440} - \frac{10057}{11520} \right) \\
& + \delta_{ae} \lambda_{\alpha\beta\gamma g} \lambda_{\beta\gamma\delta\alpha} \lambda_{df\epsilon c} \lambda_{h\delta\epsilon b} \left( -\frac{7369}{7680} \right) \\
& + \delta_{ae} \lambda_{\alpha\beta\gamma g} \lambda_{\beta\gamma\delta\alpha} \lambda_{df\epsilon b} \lambda_{h\delta\epsilon c} \left( \frac{64327}{11520} \right) \\
& + \delta_{ae} \lambda_{\alpha\beta\gamma g} \lambda_{\beta\gamma\delta\alpha} \lambda_{cd\epsilon b} \lambda_{fh\epsilon d} \left( \frac{29\zeta_3}{60} + \frac{\pi^4}{1800} - \frac{2447}{7680} \right) \\
& + \delta_{bf} \lambda_{\alpha\beta\gamma g} \lambda_{\beta\gamma\delta\alpha} \lambda_{cd\epsilon a} \lambda_{h\delta\epsilon e} \left( \frac{4267}{23040} \right) \\
& + \delta_{ef} \lambda_{\alpha\beta\epsilon g} \lambda_{\beta\gamma\delta\alpha} \lambda_{cd\epsilon a} \lambda_{h\gamma\delta b} \left( \frac{3\zeta_3}{5} - \frac{31\zeta_5}{10} - \frac{\pi^4}{300} + \frac{61}{60} \right) \\
& + \delta_{ef} \lambda_{\alpha\beta\epsilon g} \lambda_{\beta\gamma\delta\alpha} \lambda_{cdha} \lambda_{\gamma\delta\epsilon b} \left( -\frac{\zeta_3}{20} + \frac{\pi^4}{2400} + \frac{79}{256} \right) \\
& + \delta_{ae} \lambda_{\alpha\beta\epsilon g} \lambda_{\beta\gamma\delta\alpha} \lambda_{df\epsilon c} \lambda_{h\gamma\delta b} \left( \frac{3\zeta_3}{4} - \frac{57\zeta_5}{40} - \frac{\pi^4}{200} + \frac{17}{20} \right) \\
& + \delta_{ae} \lambda_{\alpha\beta\epsilon g} \lambda_{\beta\gamma\delta\alpha} \lambda_{df\epsilon b} \lambda_{h\gamma\delta c} \left( \frac{3\zeta_3}{5} + \frac{57\zeta_5}{20} - \frac{\pi^4}{40} - \frac{46}{15} \right) \\
& + \delta_{ae} \lambda_{\alpha\beta\epsilon g} \lambda_{\beta\gamma\delta\alpha} \lambda_{c\gamma\delta b} \lambda_{fh\epsilon d} \left( \frac{\zeta_3}{5} - \frac{9\zeta_5}{40} + \frac{13\pi^4}{1200} - 1 \right) \\
& + \delta_{af} \delta_{be} \lambda_{\alpha\beta\epsilon g} \lambda_{\beta\gamma\delta\alpha} \lambda_{\gamma\delta\epsilon c} \lambda_{h\epsilon\zeta d} \left( \frac{2\zeta_3}{5} - \frac{19\zeta_5}{4} + \frac{\pi^4}{300} + \frac{17}{5} \right) \\
& + \delta_{bf} \lambda_{\alpha\beta\epsilon g} \lambda_{\beta\gamma\delta\alpha} \lambda_{cd\epsilon a} \lambda_{h\gamma\delta e} \left( -\frac{3\zeta_3}{2} + \frac{99\zeta_5}{40} + \frac{\pi^4}{50} - \frac{301}{120} \right) \\
& + \delta_{bf} \lambda_{\alpha\beta\epsilon g} \lambda_{\beta\gamma\delta\alpha} \lambda_{cdha} \lambda_{\gamma\delta\epsilon e} \left( \frac{9\zeta_3}{20} - \frac{\pi^4}{400} - \frac{929}{640} \right) \\
& + \delta_{af} \delta_{be} \lambda_{\alpha\epsilon\zeta g} \lambda_{\beta\gamma\delta\alpha} \lambda_{\beta\gamma\delta c} \lambda_{h\epsilon\zeta d} \left( \frac{3\zeta_3}{4} - \frac{\pi^4}{720} - \frac{59}{96} \right) \\
& + \delta_{ae} \lambda_{\alpha\beta\epsilon b} \lambda_{\beta\gamma\delta\alpha} \lambda_{dfhc} \lambda_{\gamma\delta\epsilon g} \left( -\frac{9\zeta_3}{40} + \frac{\pi^4}{800} + \frac{1393}{3840} \right) \\
& + \delta_{df} \delta_{eg} \lambda_{\alpha\beta\gamma h} \lambda_{\beta\gamma\delta\alpha} \lambda_{c\epsilon\zeta a} \lambda_{\delta\epsilon\zeta b} \left( -\frac{13\zeta_3}{120} - \frac{\pi^4}{3600} + \frac{541}{5120} \right) \\
& + \delta_{af} \delta_{eg} \lambda_{\alpha\beta\gamma h} \lambda_{\beta\gamma\delta\alpha} \lambda_{\delta\epsilon\zeta b} \lambda_{d\epsilon\zeta c} \left( -\frac{\zeta_3}{40} - \frac{\pi^4}{1600} + \frac{221}{1536} \right) \\
& + \delta_{bg} \delta_{df} \lambda_{\alpha\beta\gamma h} \lambda_{\beta\gamma\delta\alpha} \lambda_{c\epsilon\zeta a} \lambda_{\delta\epsilon\zeta e} \left( -\frac{\zeta_3}{3} + \frac{\pi^4}{720} + \frac{1127}{7680} \right) \\
& + \delta_{df} \delta_{eg} \lambda_{\alpha\beta\epsilon h} \lambda_{\beta\gamma\delta\alpha} \lambda_{c\epsilon\zeta a} \lambda_{\gamma\delta\zeta b} \left( \frac{\zeta_3}{10} + \frac{9\zeta_5}{40} - \frac{\pi^4}{400} - \frac{1}{10} \right) \\
& + \delta_{af} \delta_{eg} \lambda_{\alpha\beta\epsilon h} \lambda_{\beta\gamma\delta\alpha} \lambda_{d\epsilon\zeta c} \lambda_{\gamma\delta\zeta b} \left( \frac{3\zeta_3}{5} - \frac{31\zeta_5}{10} - \frac{\pi^4}{300} + \frac{61}{60} \right) \\
& + \delta_{bg} \delta_{df} \lambda_{\alpha\beta\epsilon h} \lambda_{\beta\gamma\delta\alpha} \lambda_{c\epsilon\zeta a} \lambda_{\gamma\delta\zeta e} \left( -\frac{24\zeta_3}{5} + \frac{41\zeta_5}{4} - \frac{17\pi^4}{600} - \frac{46}{15} \right) \\
& + \delta_{df} \delta_{eg} \lambda_{\alpha\epsilon\zeta h} \lambda_{\beta\gamma\delta\alpha} \lambda_{\beta\gamma\delta b} \lambda_{c\epsilon\zeta a} \left( \frac{1429}{15360} \right) \\
& + \delta_{af} \delta_{eg} \lambda_{\alpha\epsilon\zeta h} \lambda_{\beta\gamma\delta\alpha} \lambda_{\beta\gamma\delta b} \lambda_{d\epsilon\zeta c} \left( \frac{\zeta_3}{12} - \frac{\pi^4}{2880} - \frac{319}{7680} \right) \\
& + \delta_{bg} \delta_{df} \lambda_{\alpha\epsilon\zeta h} \lambda_{\beta\gamma\delta\alpha} \lambda_{\beta\gamma\delta e} \lambda_{c\epsilon\zeta a} \left( -\frac{2\zeta_3}{3} + \frac{\pi^4}{720} - \frac{2447}{7680} \right)
\end{aligned}$$

$$\begin{aligned}
& + \delta_{ad} \delta_{eg} \lambda_{\alpha \varepsilon \zeta b} \lambda_{\beta \gamma \delta \alpha} \lambda_{\beta \gamma \delta h} \lambda_{f \varepsilon \zeta c} \left( -\frac{41\zeta_3}{60} + \frac{7\pi^4}{3600} - \frac{2447}{7680} \right) \\
& + \delta_{ad} \delta_{eg} \lambda_{\alpha \beta \varepsilon b} \lambda_{\beta \gamma \delta \alpha} \lambda_{f \varepsilon \zeta c} \lambda_{\gamma \delta \zeta h} \left( \frac{42\zeta_3}{5} - \frac{59\zeta_5}{20} - \frac{11\pi^4}{200} - \frac{46}{15} \right) \\
& + \delta_{be} \delta_{df} \lambda_{\alpha \beta \varepsilon g} \lambda_{\beta \gamma \delta \alpha} \lambda_{c \varepsilon \zeta a} \lambda_{\gamma \delta \zeta h} \left( -\frac{183\zeta_3}{20} - \frac{19\zeta_5}{5} + \frac{\pi^4}{300} + \frac{1609}{120} \right) \\
& + \delta_{af} \delta_{be} \lambda_{\alpha \beta \varepsilon g} \lambda_{\beta \gamma \delta \alpha} \lambda_{d \varepsilon \zeta c} \lambda_{\gamma \delta \zeta h} \left( \frac{53\zeta_3}{40} + \frac{19\zeta_5}{10} + \frac{\pi^4}{600} - \frac{241}{80} \right) \\
& + \delta_{ad} \delta_{eg} \lambda_{\alpha \beta \gamma b} \lambda_{\beta \gamma \delta \alpha} \lambda_{d \varepsilon \zeta h} \lambda_{f \varepsilon \zeta c} \left( -\frac{\zeta_3}{2} + \frac{\pi^4}{720} - \frac{2767}{23040} \right) \\
& + \delta_{be} \delta_{df} \lambda_{\alpha \beta \gamma g} \lambda_{\beta \gamma \delta \alpha} \lambda_{c \varepsilon \zeta a} \lambda_{d \varepsilon \zeta h} \left( \frac{\zeta_3}{2} - \frac{\pi^4}{1440} - \frac{10057}{11520} \right) \\
& + \delta_{af} \delta_{be} \lambda_{\alpha \beta \gamma g} \lambda_{\beta \gamma \delta \alpha} \lambda_{d \varepsilon \zeta h} \lambda_{d \varepsilon \zeta c} \left( -\frac{5\zeta_3}{24} + \frac{\pi^4}{2880} + \frac{553}{2560} \right) \\
& + \delta_{eg} \lambda_{\alpha \beta \delta a} \lambda_{\beta \gamma \varepsilon \alpha} \lambda_{d f \varepsilon c} \lambda_{h \gamma \delta b} \left( \frac{19\zeta_3}{10} + \frac{7\zeta_5}{20} - \frac{\pi^4}{200} - \frac{17}{20} \right) \\
& + \delta_{ef} \lambda_{\alpha \beta \delta b} \lambda_{\beta \gamma \varepsilon \alpha} \lambda_{d h \varepsilon a} \lambda_{g \gamma \delta c} \left( \frac{279\zeta_3^2}{20} - \frac{27\zeta_3}{2} + \frac{21\zeta_5}{5} - \frac{\pi^6}{420} \right) \\
& + \delta_{ef} \lambda_{\beta \gamma \delta c} \lambda_{\beta \gamma \varepsilon \alpha} \lambda_{d h \varepsilon a} \lambda_{g \alpha \delta b} \left( -\frac{157}{10} \zeta_3^2 - 27\zeta_3 + \frac{212\zeta_5}{5} + \frac{\pi^6}{1890} \right) \\
& + \delta_{ae} \lambda_{\alpha \beta \delta b} \lambda_{\beta \gamma \varepsilon \alpha} \lambda_{f h \varepsilon d} \lambda_{g \gamma \delta c} \left( 2\zeta_3 - \frac{18\zeta_5}{5} - \frac{2\pi^4}{75} + \frac{11}{5} \right) \\
& + \delta_{ae} \lambda_{\beta \gamma \delta c} \lambda_{\beta \gamma \varepsilon \alpha} \lambda_{f h \varepsilon d} \lambda_{g \alpha \delta b} \left( \frac{11\zeta_3}{2} - \frac{73\zeta_5}{10} - \frac{11\pi^4}{600} + \frac{11}{5} \right) \\
& + \delta_{ef} \lambda_{\beta \gamma \delta b} \lambda_{\beta \gamma \varepsilon \alpha} \lambda_{c d \varepsilon a} \lambda_{h \alpha \delta g} \left( \frac{3\zeta_3}{10} + \frac{99\zeta_5}{40} + \frac{\pi^4}{400} - 1 \right) \\
& + \delta_{ae} \lambda_{\beta \gamma \delta c} \lambda_{\beta \gamma \varepsilon \alpha} \lambda_{d f \varepsilon b} \lambda_{h \alpha \delta g} \left( \frac{17\zeta_3}{10} - \frac{7\zeta_5}{10} - \frac{\pi^4}{600} + \frac{11}{5} \right) \\
& + \delta_{bf} \lambda_{\beta \gamma \delta e} \lambda_{\beta \gamma \varepsilon \alpha} \lambda_{c d \varepsilon a} \lambda_{h \alpha \delta g} \left( \frac{19\zeta_3}{20} - \frac{7\zeta_5}{20} - \frac{\pi^4}{1200} - \frac{19}{20} \right) \\
& + \delta_{ae} \lambda_{\alpha \beta \delta b} \lambda_{\beta \gamma \varepsilon \alpha} \lambda_{d f \varepsilon c} \lambda_{h \gamma \delta g} \left( -\frac{\zeta_3}{4} + \frac{7\zeta_5}{20} - \frac{\pi^4}{400} - \frac{2}{5} \right) \\
& + \delta_{ef} \lambda_{\alpha \beta \delta g} \lambda_{\beta \gamma \varepsilon \alpha} \lambda_{c d \varepsilon a} \lambda_{h \gamma \delta b} \left( \frac{\zeta_3}{2} - \frac{127\zeta_5}{20} - \frac{\pi^4}{100} + \frac{73}{10} \right) \\
& + \delta_{ae} \lambda_{\alpha \beta \delta g} \lambda_{\beta \gamma \varepsilon \alpha} \lambda_{d f \varepsilon c} \lambda_{h \gamma \delta b} \left( \frac{3\zeta_3}{5} - \frac{83\zeta_5}{10} - \frac{\pi^4}{150} + \frac{227}{30} \right) \\
& + \delta_{ae} \lambda_{\alpha \beta \delta g} \lambda_{\beta \gamma \varepsilon \alpha} \lambda_{d f \varepsilon b} \lambda_{h \gamma \delta c} \left( \frac{52\zeta_3}{5} + \frac{83\zeta_5}{5} + \frac{\pi^4}{50} - 42 \right) \\
& + \delta_{ae} \lambda_{\alpha \beta \delta g} \lambda_{\beta \gamma \varepsilon \alpha} \lambda_{c \gamma \delta b} \lambda_{f h \varepsilon d} \left( -\frac{69\zeta_3}{10} + \frac{7\zeta_5}{10} + \frac{11\pi^4}{600} + \frac{13}{3} \right) \\
& + \delta_{bf} \lambda_{\alpha \beta \delta g} \lambda_{\beta \gamma \varepsilon \alpha} \lambda_{c d \varepsilon a} \lambda_{h \gamma \delta e} \left( -\frac{39\zeta_3}{10} + \frac{69\zeta_5}{10} + \frac{3\pi^4}{200} - \frac{7}{10} \right) \\
& + \delta_{af} \delta_{be} \lambda_{\alpha \delta \zeta g} \lambda_{\beta \gamma \delta c} \lambda_{\beta \gamma \varepsilon \alpha} \lambda_{h \varepsilon \zeta d} \left( -\frac{18\zeta_3}{5} - \frac{37\zeta_5}{5} + \frac{11\pi^4}{150} - \frac{28}{15} \right) \\
& + \delta_{df} \delta_{eg} \lambda_{\alpha \beta \delta h} \lambda_{\beta \gamma \varepsilon \alpha} \lambda_{c \varepsilon \zeta a} \lambda_{\gamma \delta \zeta b} \left( \frac{11\zeta_3}{10} - \frac{7\zeta_5}{10} - \frac{7\pi^4}{600} + \frac{24}{5} \right) \\
& + \delta_{af} \delta_{eg} \lambda_{\alpha \beta \delta h} \lambda_{\beta \gamma \varepsilon \alpha} \lambda_{d \varepsilon \zeta c} \lambda_{\gamma \delta \zeta b} \left( \frac{\zeta_3}{2} - \frac{127\zeta_5}{20} - \frac{\pi^4}{100} + \frac{73}{10} \right) \\
& + \delta_{bg} \delta_{df} \lambda_{\alpha \beta \delta h} \lambda_{\beta \gamma \varepsilon \alpha} \lambda_{c \varepsilon \zeta a} \lambda_{\gamma \delta \zeta e} \left( 38\zeta_3 - \frac{17\zeta_5}{5} - 42 \right) \\
& + \delta_{df} \delta_{eg} \lambda_{\alpha \delta \zeta h} \lambda_{\beta \gamma \delta b} \lambda_{\beta \gamma \varepsilon \alpha} \lambda_{c \varepsilon \zeta a} \left( -\frac{27\zeta_3}{10} - 3\zeta_5 - \frac{\pi^4}{200} + \frac{24}{5} \right)
\end{aligned}$$

$$\begin{aligned}
& + \delta_{af} \delta_{eg} \lambda_{\alpha\delta\zeta h} \lambda_{\beta\gamma\delta b} \lambda_{\beta\gamma\epsilon\alpha} \lambda_{d\epsilon\zeta c} \left( -\frac{33\zeta_3}{10} - \frac{19\zeta_5}{20} - \frac{\pi^4}{50} + \frac{73}{10} \right) \\
& + \delta_{bg} \delta_{df} \lambda_{\alpha\delta\zeta h} \lambda_{\beta\gamma\delta e} \lambda_{\beta\gamma\epsilon\alpha} \lambda_{c\epsilon\zeta a} (12\zeta_3 + 22\zeta_5 - 42) \\
& + \delta_{ad} \delta_{eg} \lambda_{\alpha\delta\zeta b} \lambda_{\beta\gamma\delta h} \lambda_{\beta\gamma\epsilon\alpha} \lambda_{f\epsilon\zeta c} \left( \frac{238\zeta_3}{5} - \frac{116\zeta_5}{5} - \frac{\pi^4}{50} - 42 \right) \\
& + \delta_{ad} \delta_{eg} \lambda_{\alpha\beta\delta b} \lambda_{\beta\gamma\epsilon\alpha} \lambda_{f\epsilon\zeta c} \lambda_{\gamma\delta\zeta h} \left( \frac{164\zeta_3}{5} + \frac{107\zeta_5}{5} - \frac{3\pi^4}{50} - 42 \right) \\
& + \delta_{be} \delta_{df} \lambda_{\alpha\beta\delta g} \lambda_{\beta\gamma\epsilon\alpha} \lambda_{c\epsilon\zeta a} \lambda_{\gamma\delta\zeta h} \left( -\frac{113\zeta_3}{5} - \frac{46\zeta_5}{5} + \frac{\pi^4}{25} + \frac{237}{10} \right) \\
& + \delta_{af} \delta_{be} \lambda_{\alpha\beta\delta g} \lambda_{\beta\gamma\epsilon\alpha} \lambda_{d\epsilon\zeta c} \lambda_{\gamma\delta\zeta h} \left( \frac{24\zeta_3}{5} + \frac{23\zeta_5}{5} + \frac{\pi^4}{300} - \frac{239}{30} \right) \\
& + \delta_{ef} \lambda_{\beta\gamma\delta\alpha} \lambda_{\beta\gamma\epsilon\alpha} \lambda_{c\gamma\delta b} \lambda_{dh\epsilon a} \left( \frac{151\zeta_3}{160} - \frac{21\zeta_5}{80} + \frac{\pi^4}{1200} \right) \\
& + \delta_{ef} \lambda_{\beta\gamma\delta\alpha} \lambda_{\beta\gamma\epsilon\alpha} \lambda_{cd\epsilon a} \lambda_{gh\delta b} \left( -\frac{\zeta_3}{80} - \frac{\pi^4}{3200} + \frac{221}{3072} \right) \\
& + \delta_{df} \delta_{eg} \lambda_{\beta\gamma\delta\alpha} \lambda_{\beta\gamma\epsilon\alpha} \lambda_{c\epsilon\zeta a} \lambda_{h\delta\zeta b} \left( -\frac{5023}{15360} \right) \\
& + \delta_{af} \delta_{eg} \lambda_{\beta\gamma\delta\alpha} \lambda_{\beta\gamma\epsilon\alpha} \lambda_{d\epsilon\zeta c} \lambda_{h\delta\zeta b} \left( \frac{\zeta_3}{2} - \frac{\pi^4}{1440} - \frac{10057}{11520} \right) \\
& + \delta_{af} \delta_{dg} \delta_{eh} \lambda_{\beta\gamma\delta\alpha} \lambda_{\beta\gamma\epsilon\alpha} \lambda_{\delta\zeta\eta b} \lambda_{\epsilon\zeta\eta c} \left( \frac{1069}{5120} \right) \\
& + \delta_{ae} \lambda_{\beta\gamma\delta\alpha} \lambda_{\beta\gamma\epsilon\alpha} \lambda_{c\gamma\delta b} \lambda_{fh\epsilon d} \left( -\frac{2447}{7680} \right) \\
& + \delta_{af} \delta_{be} \lambda_{\beta\gamma\delta\alpha} \lambda_{\beta\gamma\epsilon\alpha} \lambda_{g\delta\zeta c} \lambda_{h\epsilon\zeta d} \left( \frac{13\zeta_3}{24} - \frac{\pi^4}{1440} + \frac{599}{2560} \right) \\
& + \delta_{bf} \lambda_{\beta\gamma\delta\alpha} \lambda_{\beta\gamma\epsilon\alpha} \lambda_{cd\epsilon a} \lambda_{gh\delta e} \left( \frac{249}{5120} \right) \\
& + \delta_{bg} \delta_{df} \lambda_{\beta\gamma\delta\alpha} \lambda_{\beta\gamma\epsilon\alpha} \lambda_{c\epsilon\zeta a} \lambda_{h\delta\zeta e} \left( -2\zeta_3 + \frac{\pi^4}{360} + \frac{64327}{11520} \right) \\
& + \delta_{af} \delta_{be} \lambda_{\beta\gamma\delta\alpha} \lambda_{\beta\gamma\epsilon\alpha} \lambda_{d\epsilon\zeta c} \lambda_{h\delta\zeta g} \left( -\frac{5\zeta_3}{48} + \frac{\pi^4}{5760} + \frac{553}{5120} \right) \\
& + \delta_{af} \delta_{bd} \delta_{eg} \lambda_{\beta\gamma\delta\alpha} \lambda_{\beta\gamma\epsilon\alpha} \lambda_{\delta\zeta\eta h} \lambda_{\epsilon\zeta\eta c} \left( -\frac{2789}{5120} \right) \\
& + \delta_{ef} \lambda_{\beta\delta\epsilon\alpha} \lambda_{d\delta\epsilon a} \lambda_{g\alpha\gamma b} \lambda_{h\beta\gamma c} \left( \frac{2\zeta_3^2}{5} - \frac{1}{75}\pi^4\zeta_3 - 26\zeta_5 + \frac{499\zeta_7}{10} - \frac{\pi^6}{189} \right) \\
& + \delta_{af} \lambda_{\beta\delta\epsilon\alpha} \lambda_{c\beta\gamma b} \lambda_{e\delta\epsilon d} \lambda_{h\alpha\gamma g} \left( \frac{19\zeta_3}{20} + \frac{7\zeta_5}{40} + \frac{\pi^4}{600} + \frac{17}{20} \right) \\
& + \delta_{ae} \lambda_{\beta\delta\epsilon\alpha} \lambda_{c\beta\gamma b} \lambda_{f\delta\epsilon d} \lambda_{h\alpha\gamma g} \left( \frac{36\zeta_3}{5} - \frac{7\zeta_5}{4} - \frac{\pi^4}{120} - \frac{46}{15} \right) \\
& + \delta_{df} \delta_{eg} \lambda_{\beta\delta\zeta\alpha} \lambda_{\beta\gamma\epsilon\alpha} \lambda_{c\epsilon\zeta a} \lambda_{h\gamma\delta b} \left( \frac{3\zeta_3}{5} + \frac{9\zeta_5}{4} + \frac{\pi^4}{200} - \frac{57}{20} \right) \\
& + \delta_{af} \delta_{eg} \lambda_{\beta\delta\zeta\alpha} \lambda_{\beta\gamma\epsilon\alpha} \lambda_{d\epsilon\zeta c} \lambda_{h\gamma\delta b} \left( \frac{\zeta_3}{5} + \frac{53\zeta_5}{20} + \frac{\pi^4}{60} - \frac{14}{3} \right) \\
& + \delta_{af} \delta_{dg} \delta_{eh} \lambda_{\beta\delta\zeta\alpha} \lambda_{\beta\gamma\epsilon\alpha} \lambda_{\gamma\delta\eta b} \lambda_{\epsilon\zeta\eta c} \left( -\frac{63\zeta_3}{80} - \frac{\pi^4}{800} - \frac{19}{1280} \right) \\
& + \delta_{af} \delta_{be} \lambda_{\beta\delta\zeta\alpha} \lambda_{\beta\gamma\epsilon\alpha} \lambda_{g\gamma\delta c} \lambda_{h\epsilon\zeta d} \left( -4\zeta_3 - \frac{37\zeta_5}{20} + \frac{193}{30} \right) \\
& + \delta_{bg} \delta_{df} \lambda_{\beta\delta\zeta\alpha} \lambda_{\beta\gamma\epsilon\alpha} \lambda_{c\epsilon\zeta a} \lambda_{h\gamma\delta e} \left( -\frac{46\zeta_3}{5} - \frac{8\zeta_5}{5} - \frac{7\pi^4}{150} + \frac{184}{15} \right) \\
& + \delta_{af} \delta_{be} \lambda_{\beta\delta\zeta\alpha} \lambda_{\beta\gamma\epsilon\alpha} \lambda_{d\epsilon\zeta c} \lambda_{h\gamma\delta g} \left( \frac{\zeta_3}{40} - \frac{53\zeta_5}{80} - \frac{\pi^4}{400} + \frac{163}{240} \right)
\end{aligned}$$



$$\begin{aligned}
& + \delta_{af} \delta_{bd} \delta_{eg} \lambda_{\beta\delta\zeta\alpha} \lambda_{\beta\gamma\epsilon\alpha} \lambda_{\gamma\delta\eta h} \lambda_{\epsilon\zeta\eta c} \left( \frac{147\zeta_3}{80} + \frac{\pi^4}{800} + \frac{931}{1280} \right) \\
& + \delta_{af} \delta_{be} \lambda_{\alpha\gamma\delta g} \lambda_{\beta\gamma\delta c} \lambda_{\beta\epsilon\zeta\alpha} \lambda_{h\epsilon\zeta d} \left( -\frac{17\zeta_3}{2} + \frac{9\zeta_5}{5} + \frac{3\pi^4}{200} + 7 \right) \\
& + \delta_{df} \delta_{eg} \lambda_{\alpha\gamma\delta h} \lambda_{\beta\gamma\delta b} \lambda_{\beta\epsilon\zeta\alpha} \lambda_{c\epsilon\zeta a} \left( \frac{7\zeta_3}{5} - \frac{\zeta_5}{5} + \frac{\pi^4}{150} - 2 \right) \\
& + \delta_{af} \delta_{eg} \lambda_{\alpha\gamma\delta h} \lambda_{\beta\gamma\delta b} \lambda_{\beta\epsilon\zeta\alpha} \lambda_{d\epsilon\zeta c} \left( \frac{3\zeta_3}{10} + \frac{99\zeta_5}{40} + \frac{\pi^4}{400} - 1 \right) \\
& + \delta_{bg} \delta_{df} \lambda_{\alpha\gamma\delta h} \lambda_{\beta\gamma\delta e} \lambda_{\beta\epsilon\zeta\alpha} \lambda_{c\epsilon\zeta a} \left( \frac{47\zeta_3}{10} - \frac{28\zeta_5}{5} - \frac{13\pi^4}{600} + \frac{11}{5} \right) \\
& + \delta_{ad} \delta_{eg} \lambda_{\alpha\gamma\delta b} \lambda_{\beta\gamma\delta h} \lambda_{\beta\epsilon\zeta\alpha} \lambda_{f\epsilon\zeta c} \left( \frac{13\zeta_3}{10} + \frac{4\zeta_5}{5} - \frac{23\pi^4}{600} + \frac{11}{5} \right) \\
& + \delta_{be} \delta_{df} \lambda_{\alpha\gamma\delta g} \lambda_{\beta\gamma\delta h} \lambda_{\beta\epsilon\zeta\alpha} \lambda_{c\epsilon\zeta a} \left( \frac{\zeta_3}{5} + \frac{53\zeta_5}{20} + \frac{\pi^4}{60} - \frac{14}{3} \right) \\
& + \delta_{af} \delta_{be} \lambda_{\alpha\gamma\delta g} \lambda_{\beta\gamma\delta h} \lambda_{\beta\epsilon\zeta\alpha} \lambda_{d\epsilon\zeta c} \left( \frac{\zeta_3}{20} - \frac{53\zeta_5}{40} - \frac{\pi^4}{200} + \frac{163}{120} \right) \\
& + \delta_{df} \delta_{eg} \lambda_{\beta\gamma\delta\alpha} \lambda_{\beta\epsilon\zeta\alpha} \lambda_{c\epsilon\zeta a} \lambda_{h\gamma\delta b} \left( -\frac{9\zeta_3}{80} - \frac{27\zeta_5}{160} + \frac{3\pi^4}{1600} + \frac{3}{32} \right) \\
& + \delta_{af} \delta_{eg} \lambda_{\beta\gamma\delta\alpha} \lambda_{\beta\epsilon\zeta\alpha} \lambda_{dh\zeta c} \lambda_{\gamma\delta\epsilon b} \left( -\frac{\zeta_3}{20} + \frac{\pi^4}{2400} + \frac{79}{256} \right) \\
& + \delta_{af} \delta_{eg} \lambda_{\beta\gamma\delta\alpha} \lambda_{\beta\epsilon\zeta\alpha} \lambda_{d\epsilon\zeta c} \lambda_{h\gamma\delta b} \left( \frac{7\zeta_3}{20} - \frac{3\zeta_5}{4} + \frac{\pi^4}{400} + \frac{7}{40} \right) \\
& + \delta_{af} \delta_{dg} \delta_{eh} \lambda_{\beta\gamma\delta\alpha} \lambda_{\beta\epsilon\zeta\alpha} \lambda_{\gamma\delta\eta b} \lambda_{\epsilon\zeta\eta c} \left( -\frac{81\zeta_3}{320} + \frac{\pi^4}{3200} - \frac{93}{2560} \right) \\
& + \delta_{af} \delta_{be} \lambda_{\beta\gamma\delta\alpha} \lambda_{\beta\epsilon\zeta\alpha} \lambda_{g\gamma\delta c} \lambda_{h\epsilon\zeta d} \left( -\frac{23\zeta_3}{40} - \frac{33\zeta_5}{80} + \frac{11\pi^4}{1200} + \frac{19}{80} \right) \\
& + \delta_{bg} \delta_{df} \lambda_{\beta\gamma\delta\alpha} \lambda_{\beta\epsilon\zeta\alpha} \lambda_{c\epsilon\zeta a} \lambda_{h\gamma\delta e} \left( -\frac{5\zeta_3}{4} + \frac{93\zeta_5}{40} - \frac{\pi^4}{400} - \frac{5}{8} \right) \\
& + \delta_{bg} \delta_{df} \lambda_{\beta\gamma\delta\alpha} \lambda_{\beta\epsilon\zeta\alpha} \lambda_{ch\zeta a} \lambda_{\gamma\delta\epsilon e} \left( \frac{4\zeta_3}{5} + \frac{\pi^4}{1200} + \frac{4823}{640} \right) \\
& + \delta_{af} \delta_{be} \lambda_{\beta\gamma\delta\alpha} \lambda_{\beta\epsilon\zeta\alpha} \lambda_{d\epsilon\zeta c} \lambda_{h\gamma\delta g} \left( -\frac{\zeta_3}{16} + \frac{3\zeta_5}{16} - \frac{\pi^4}{960} - \frac{1}{32} \right) \\
& + \delta_{af} \delta_{be} \lambda_{\beta\gamma\delta\alpha} \lambda_{\beta\epsilon\zeta\alpha} \lambda_{dh\zeta c} \lambda_{\gamma\delta\epsilon g} \left( -\frac{3\zeta_3}{20} - \frac{\pi^4}{2400} - \frac{5509}{3840} \right) \\
& + \delta_{af} \delta_{eg} \lambda_{\beta\gamma\delta\alpha} \lambda_{\beta\epsilon\zeta\alpha} \lambda_{cd\zeta b} \lambda_{\gamma\delta\epsilon h} \left( -\frac{7\zeta_3}{20} - \frac{\pi^4}{1200} - \frac{929}{640} \right) \\
& + \delta_{af} \delta_{bd} \delta_{eg} \lambda_{\beta\gamma\delta\alpha} \lambda_{\beta\epsilon\zeta\alpha} \lambda_{\gamma\delta\eta h} \lambda_{\epsilon\zeta\eta c} \left( \frac{33\zeta_3}{64} - \frac{\pi^4}{3200} + \frac{69}{2560} \right) \\
& + \delta_{af} \delta_{dg} \delta_{eh} \lambda_{\beta\gamma\delta b} \lambda_{\beta\gamma\epsilon\alpha} \lambda_{\delta\zeta\eta\alpha} \lambda_{\epsilon\zeta\eta c} \left( -\frac{\zeta_3}{40} + \frac{\pi^4}{400} - \frac{1103}{640} \right) \\
& + \delta_{af} \delta_{bd} \delta_{eg} \lambda_{\beta\gamma\delta h} \lambda_{\beta\gamma\epsilon\alpha} \lambda_{\delta\zeta\eta\alpha} \lambda_{\epsilon\zeta\eta c} \left( -\frac{7\zeta_3}{8} - \frac{\pi^4}{400} + \frac{575}{128} \right) \\
& + \delta_{af} \delta_{dg} \delta_{eh} \lambda_{\beta\gamma\delta\alpha} \lambda_{\beta\gamma\delta b} \lambda_{\epsilon\zeta\eta\alpha} \lambda_{\epsilon\zeta\eta c} \left( \frac{\zeta_3}{72} - \frac{7}{1536} \right) \\
& + \delta_{af} \delta_{bd} \delta_{eg} \lambda_{\beta\gamma\delta\alpha} \lambda_{\beta\gamma\delta h} \lambda_{\epsilon\zeta\eta\alpha} \lambda_{\epsilon\zeta\eta c} \left( \frac{5}{4608} - \frac{\zeta_3}{72} \right)
\end{aligned} \tag{19}$$

$$\begin{aligned}
\Box_{abc|def|ghi|jkl}^{(3)} &= \delta_{aj} \delta_{bk} \delta_{ch} \delta_{dg} \delta_{el} \delta_{fi} \left( -\frac{1}{8} \right) \\
&+ \delta_{aj} \delta_{bh} \delta_{ce} \delta_{dg} \delta_{fl} \delta_{ik} \left( \frac{\zeta_3}{2} \right)
\end{aligned} \tag{20}$$

$$\begin{aligned}
\Box_{abc|def|ghi|jkl}^{(4)} &= \delta_{ch}\delta_{dg}\delta_{fl}\delta_{ik}\lambda_{beja}\left(\frac{\pi^4}{60} - 3\zeta_3\right) \\
&+ \delta_{bj}\delta_{ch}\delta_{dg}\delta_{fl}\lambda_{eika}(-5\zeta_5) \\
&+ \delta_{ak}\delta_{bl}\delta_{cg}\delta_{dj}\lambda_{fhie}\left(\frac{\zeta_3}{4} - \frac{1}{8}\right) \\
&+ \delta_{ak}\delta_{bg}\delta_{ch}\delta_{dj}\lambda_{file}\left(\frac{2}{3}\right)
\end{aligned} \tag{21}$$

$$\begin{aligned}
\Box_{abc|def|ghi|jkl}^{(5)} &= \delta_{ce}\delta_{il}\lambda_{dhkb}\lambda_{fgja}\left(\frac{9\zeta_3^2}{2}\right) \\
&+ \delta_{ch}\delta_{dg}\delta_{il}\lambda_{ej\alpha a}\lambda_{fk\alpha b}(6\zeta_3^2) \\
&+ \delta_{cg}\delta_{il}\lambda_{bdka}\lambda_{fhje}\left(\frac{\zeta_3}{2} - \frac{3\zeta_5}{2} - \frac{\pi^4}{40}\right) \\
&+ \delta_{bj}\delta_{cg}\lambda_{dila}\lambda_{fhke}\left(-\frac{5}{2}\zeta_3^2 + \frac{25\zeta_5}{2} - \frac{5\pi^6}{756}\right) \\
&+ \delta_{bj}\delta_{cg}\delta_{il}\lambda_{dk\alpha a}\lambda_{fh\alpha e}\left(\frac{31\zeta_3}{4} + \frac{7\zeta_5}{4} - \frac{7\pi^4}{240}\right) \\
&+ \delta_{cg}\delta_{il}\lambda_{bdha}\lambda_{fjke}\left(-\frac{5\zeta_3}{8} + \frac{\pi^4}{480} + \frac{3}{8}\right) \\
&+ \delta_{ck}\delta_{dg}\lambda_{bhia}\lambda_{fjle}\left(-\frac{\zeta_3}{16} + \frac{\pi^4}{960} - \frac{1}{32}\right) \\
&+ \delta_{cg}\delta_{hk}\delta_{il}\lambda_{bd\alpha a}\lambda_{fj\alpha e}\left(-\frac{5\zeta_3}{8} + \frac{\pi^4}{480} + \frac{3}{8}\right) \\
&+ \delta_{ch}\delta_{dg}\delta_{il}\lambda_{bk\alpha a}\lambda_{fj\alpha e}\left(\frac{\zeta_3}{4} - \frac{3\zeta_5}{4} - \frac{\pi^4}{80}\right) \\
&+ \delta_{bg}\delta_{ch}\delta_{il}\lambda_{dk\alpha a}\lambda_{fj\alpha e}\left(-\frac{7}{3}\right) \\
&+ \delta_{ck}\delta_{dg}\lambda_{bfia}\lambda_{hjle}\left(\frac{\zeta_3}{8} + \frac{7\zeta_5}{8} - \frac{\pi^4}{160}\right) \\
&+ \delta_{bj}\delta_{ck}\delta_{dg}\lambda_{fi\alpha a}\lambda_{hl\alpha e}\left(-\frac{13\zeta_3}{8} - \frac{7\zeta_5}{8} + \frac{\pi^4}{480}\right) \\
&+ \delta_{bk}\delta_{cg}\delta_{dj}\lambda_{fi\alpha a}\lambda_{hl\alpha e}\left(\frac{441\zeta_7}{8}\right) \\
&+ \delta_{bk}\delta_{cg}\delta_{dj}\delta_{il}\lambda_{f\alpha\beta a}\lambda_{h\alpha\beta e}\left(\frac{31\zeta_3}{4} - \frac{23\zeta_5}{4} - \frac{7\pi^4}{240}\right) \\
&+ \delta_{ch}\delta_{dg}\delta_{fl}\lambda_{bk\alpha a}\lambda_{ij\alpha e}\left(\zeta_3^2 + 25\zeta_5 - \frac{5\pi^6}{378}\right) \\
&+ \delta_{bj}\delta_{ch}\delta_{dg}\delta_{fl}\lambda_{i\alpha\beta e}\lambda_{k\alpha\beta a}\left(-\frac{11}{4}\zeta_3^2 + \frac{25\zeta_5}{4} - \frac{5\pi^6}{1512}\right) \\
&+ \delta_{ch}\delta_{dg}\delta_{fl}\lambda_{bi\alpha a}\lambda_{jk\alpha e}\left(\frac{1}{3}\right) \\
&+ \delta_{ch}\delta_{dg}\delta_{fl}\delta_{ik}\lambda_{b\alpha\beta a}\lambda_{j\alpha\beta e}\left(\frac{\zeta_3}{4} + \frac{7\zeta_5}{4} - \frac{\pi^4}{80}\right) \\
&+ \delta_{cj}\delta_{dg}\delta_{fi}\lambda_{bh\alpha a}\lambda_{kl\alpha e}\left(-\frac{\zeta_3}{16} - \frac{\pi^4}{960}\right) \\
&+ \delta_{bj}\delta_{ck}\delta_{dg}\delta_{fi}\lambda_{h\alpha\beta a}\lambda_{l\alpha\beta e}\left(\frac{1}{12}\right) \\
&+ \delta_{ce}\delta_{il}\lambda_{bdka}\lambda_{ghjf}\left(\frac{1}{3}\right) \\
&+ \delta_{ak}\delta_{bl}\delta_{cg}\delta_{dj}\lambda_{h\alpha\beta e}\lambda_{i\alpha\beta f}\left(-\frac{5\zeta_3}{16} - \frac{\pi^4}{960} + \frac{29}{48}\right) \\
&+ \delta_{ak}\delta_{bg}\delta_{ch}\delta_{dj}\lambda_{i\alpha\beta f}\lambda_{l\alpha\beta e}\left(-\frac{\zeta_3}{2} + \frac{\pi^4}{120} - \frac{7}{3}\right)
\end{aligned}$$

$$\begin{aligned}
& + \delta_{ak} \delta_{bl} \delta_{cg} \delta_{dj} \lambda_{f\alpha\beta e} \lambda_{i\alpha\beta h} \left( -\frac{\zeta_3}{8} + \frac{\pi^4}{480} - \frac{1}{16} \right) \\
& + \delta_{ak} \delta_{bg} \delta_{ce} \delta_{dj} \delta_{il} \lambda_{\alpha\beta\gamma f} \lambda_{\alpha\beta\gamma h} \left( \frac{\pi^4}{720} - \frac{9\zeta_3}{16} \right) \\
& + \delta_{ch} \delta_{dg} \delta_{fl} \lambda_{be\alpha a} \lambda_{jk\alpha i} \left( \frac{\zeta_3}{4} - 2\zeta_5 - \frac{\pi^4}{80} \right) \\
& + \delta_{bj} \delta_{ch} \delta_{dg} \delta_{fl} \lambda_{e\alpha\beta a} \lambda_{k\alpha\beta i} \left( -\frac{17}{8}\zeta_3^2 + \frac{25\zeta_5}{8} - \frac{5\pi^6}{3024} \right) \\
& + \delta_{ak} \delta_{bg} \delta_{ch} \delta_{dj} \lambda_{f\alpha\beta e} \lambda_{l\alpha\beta i} \left( -\frac{\zeta_3}{8} - \frac{\pi^4}{480} \right) \\
& + \delta_{aj} \delta_{bk} \delta_{ch} \delta_{dg} \delta_{fl} \lambda_{\alpha\beta\gamma e} \lambda_{\alpha\beta\gamma i} \left( \frac{755}{4608} \right) \\
& + \delta_{ak} \delta_{bg} \delta_{ch} \delta_{dj} \delta_{fl} \lambda_{\alpha\beta\gamma e} \lambda_{\alpha\beta\gamma i} \left( \frac{\zeta_3}{24} - \frac{151}{4608} \right) \tag{22} \\
\Box_{abc|def|ghi|jkl}^{(6)} = & \lambda_{dilc} \lambda_{egja} \lambda_{fhkb} \left( \frac{96\zeta_{35}}{5} + 36\zeta_3\zeta_5 - \frac{116\pi^8}{23625} \right) \\
& + \lambda_{cilib} \lambda_{djka} \lambda_{fghe} \left( \frac{11\zeta_3}{80} + \frac{7\zeta_5}{80} - \frac{\pi^4}{960} - \frac{11}{80} \right) \\
& + \delta_{il} \lambda_{chab} \lambda_{dk\alpha a} \lambda_{fgje} \left( -\frac{11}{20}\zeta_3^2 - \frac{3\zeta_3}{10} + \frac{17\zeta_5}{10} - \frac{\pi^6}{3780} + \frac{\pi^4}{25} \right) \\
& + \lambda_{cilib} \lambda_{dhka} \lambda_{fgje} \left( \frac{5\zeta_3^2}{4} - \frac{1}{120}\pi^4\zeta_3 - \frac{7\zeta_5}{4} + \frac{9\zeta_7}{4} + \frac{5\pi^6}{1512} \right) \\
& + \delta_{il} \lambda_{ck\alpha b} \lambda_{dhja} \lambda_{fg\alpha e} \left( \frac{5\zeta_3^2}{2} - \frac{1}{60}\pi^4\zeta_3 - \frac{7\zeta_5}{2} + \zeta_7 + \frac{5\pi^6}{756} \right) \\
& + \delta_{cg} \lambda_{dl\alpha b} \lambda_{fhje} \lambda_{ik\alpha a} \left( -\frac{81\zeta_{35}}{25} - \frac{3087\zeta_7}{40} + \frac{2063\pi^8}{420000} \right) \\
& + \delta_{cg} \lambda_{di\alpha b} \lambda_{fjke} \lambda_{hl\alpha a} \left( \frac{57\zeta_3^2}{40} - \frac{31\zeta_3}{40} + \frac{7\zeta_5}{40} - \frac{\pi^6}{2520} - \frac{\pi^4}{800} \right) \\
& + \delta_{cg} \lambda_{dilb} \lambda_{fj\alpha e} \lambda_{hk\alpha a} \left( \frac{3}{25}\pi^4\zeta_3 - 18\zeta_3^2 \right) \\
& + \delta_{cg} \delta_{il} \lambda_{dk\beta b} \lambda_{fj\alpha e} \lambda_{h\alpha\beta a} \left( -\frac{81\zeta_{35}}{25} + 18\zeta_3\zeta_5 - \frac{3087\zeta_7}{40} + \frac{2063\pi^8}{420000} \right) \\
& + \delta_{cg} \delta_{il} \lambda_{dk\beta b} \lambda_{f\alpha\beta e} \lambda_{hj\alpha a} \left( 5\zeta_3^2 - \frac{1}{60}\pi^4\zeta_3 - 31\zeta_5 - \frac{19\zeta_7}{2} + \frac{5\pi^6}{378} \right) \\
& + \lambda_{cilib} \lambda_{dfka} \lambda_{ghje} \left( \frac{13\zeta_3^2}{20} + \frac{\zeta_3}{20} + \frac{9\zeta_5}{20} - \frac{\pi^6}{1890} + \frac{\pi^4}{1200} \right) \\
& + \delta_{il} \lambda_{chkb} \lambda_{df\alpha a} \lambda_{gj\alpha e} \left( -\frac{39}{40}\zeta_3^2 - \frac{3\zeta_3}{20} - \frac{63\zeta_5}{20} + \frac{\pi^6}{840} + \frac{\pi^4}{50} \right) \\
& + \delta_{il} \lambda_{chab} \lambda_{dfka} \lambda_{gj\alpha e} \left( 2\zeta_3^2 - \frac{1}{75}\pi^4\zeta_3 - 7\zeta_5 - \frac{323\zeta_7}{80} + \frac{5\pi^6}{378} \right) \\
& + \delta_{cg} \lambda_{dilb} \lambda_{fk\alpha a} \lambda_{hj\alpha e} \left( -\frac{216\zeta_{35}}{5} - 126\zeta_3\zeta_5 + \frac{29\pi^8}{2625} \right) \\
& + \delta_{cg} \delta_{il} \lambda_{dfkb} \lambda_{h\alpha\beta a} \lambda_{j\alpha\beta e} \left( 8\zeta_3^2 - \frac{4}{75}\pi^4\zeta_3 - 7\zeta_5 - \frac{239\zeta_7}{80} + \frac{5\pi^6}{378} \right) \\
& + \delta_{cg} \delta_{il} \lambda_{df\beta b} \lambda_{hk\alpha a} \lambda_{j\alpha\beta e} \left( -2\zeta_3^2 + \frac{1}{150}\pi^4\zeta_3 - 62\zeta_5 - \frac{359\zeta_7}{20} + \frac{5\pi^6}{189} \right) \\
& + \delta_{ch} \delta_{dg} \delta_{il} \lambda_{\alpha\beta\gamma a} \lambda_{fk\gamma b} \lambda_{j\alpha\beta e} \left( -\frac{198}{5}\zeta_3^2 + \frac{3}{25}\pi^4\zeta_3 + \frac{567\zeta_7}{10} \right) \\
& + \delta_{ch} \delta_{dg} \delta_{il} \lambda_{f\beta\gamma b} \lambda_{j\alpha\beta e} \lambda_{k\alpha\gamma a} (-40\zeta_3\zeta_5) \\
& + \delta_{ce} \delta_{il} \lambda_{dh\beta b} \lambda_{gj\alpha f} \lambda_{k\alpha\beta a} \left( -8\zeta_3^3 - \frac{1063\zeta_9}{9} \right)
\end{aligned}$$

$$\begin{aligned}
& + \delta_{ce} \delta_{il} \lambda_{d\alpha\beta b} \lambda_{gj\alpha f} \lambda_{hk\beta a} (-60\zeta_3\zeta_5) \\
& + \delta_{ce} \delta_{il} \lambda_{dhkb} \lambda_{g\alpha\beta f} \lambda_{j\alpha\beta a} \left( -18\zeta_3^2 + \frac{3}{50}\pi^4\zeta_3 + \frac{189\zeta_7}{8} \right) \\
& + \delta_{cg} \lambda_{bd\alpha a} \lambda_{hilf} \lambda_{jk\alpha e} \left( \frac{5\zeta_3^2}{4} + \frac{3\zeta_3}{20} - \frac{3\zeta_5}{20} - \frac{\pi^6}{3780} + \frac{\pi^4}{400} \right) \\
& + \delta_{cg} \delta_{il} \lambda_{bd\beta a} \lambda_{hk\alpha f} \lambda_{j\alpha\beta e} \left( -\frac{81\zeta_{35}}{25} - 27\zeta_3\zeta_5 - \frac{3087\zeta_7}{40} + \frac{2063\pi^8}{420000} \right) \\
& + \delta_{bj} \delta_{cg} \delta_{il} \lambda_{\alpha\beta\gamma e} \lambda_{d\beta\gamma a} \lambda_{hk\alpha f} \left( \frac{243\zeta_3^2}{20} - \frac{102\zeta_3}{5} - \frac{21\zeta_5}{5} + \frac{\pi^6}{1260} + \frac{43\pi^4}{600} \right) \\
& + \delta_{cg} \lambda_{bdia} \lambda_{hl\alpha f} \lambda_{jk\alpha e} \left( -\frac{13}{10} \right) \\
& + \delta_{bj} \delta_{cg} \lambda_{di\beta a} \lambda_{hl\alpha f} \lambda_{k\alpha\beta e} \left( -16\zeta_3^3 - \frac{2126\zeta_9}{9} \right) \\
& + \delta_{bk} \delta_{cg} \delta_{dj} \lambda_{\alpha\beta\gamma e} \lambda_{hl\alpha f} \lambda_{i\beta\gamma a} \left( -\frac{81\zeta_{35}}{25} + 27\zeta_3\zeta_5 - \frac{3087\zeta_7}{40} + \frac{2063\pi^8}{420000} \right) \\
& + \delta_{cg} \delta_{il} \lambda_{bd\beta a} \lambda_{h\alpha\beta f} \lambda_{jk\alpha e} \left( -\frac{1}{2}\zeta_3^2 + \frac{1}{300}\pi^4\zeta_3 - \frac{7\zeta_5}{2} + \frac{61\zeta_7}{40} + \frac{5\pi^6}{756} \right) \\
& + \delta_{cg} \delta_{il} \lambda_{bdka} \lambda_{h\alpha\beta f} \lambda_{j\alpha\beta e} \left( \frac{43\zeta_3^2}{20} - \frac{3\zeta_3}{10} + \frac{47\zeta_5}{10} - \frac{4\pi^6}{945} + \frac{\pi^4}{25} \right) \\
& + \delta_{bj} \delta_{cg} \lambda_{dila} \lambda_{h\alpha\beta f} \lambda_{k\alpha\beta e} \left( 5\zeta_3^2 - \frac{1}{60}\pi^4\zeta_3 - 31\zeta_5 + \frac{9\zeta_7}{2} + \frac{5\pi^6}{378} \right) \\
& + \delta_{bj} \delta_{cg} \delta_{il} \lambda_{d\beta\gamma a} \lambda_{h\alpha\gamma f} \lambda_{k\alpha\beta e} \left( \frac{63\zeta_7}{2} - 24\zeta_3^2 \right) \\
& + \delta_{bk} \delta_{cg} \delta_{dj} \lambda_{h\alpha\gamma f} \lambda_{i\beta\gamma a} \lambda_{l\alpha\beta e} (-168\zeta_9) \\
& + \delta_{bk} \delta_{cg} \delta_{dj} \delta_{il} \lambda_{\alpha\beta\gamma e} \lambda_{\beta\gamma\delta a} \lambda_{h\alpha\delta f} \left( \frac{57\zeta_3^2}{10} - \frac{204\zeta_3}{5} + \frac{138\zeta_5}{5} - \frac{2\pi^6}{315} + \frac{43\pi^4}{300} \right) \\
& + \delta_{ck} \delta_{dg} \lambda_{b\alpha\beta a} \lambda_{h\alpha\beta e} \lambda_{ijlf} \left( -\frac{3}{40}\zeta_3^2 + \frac{3\zeta_3}{40} - \frac{63\zeta_5}{40} + \frac{\pi^6}{840} + \frac{\pi^4}{800} \right) \\
& + \delta_{cg} \lambda_{bd\alpha a} \lambda_{hj\alpha e} \lambda_{iklf} \left( 2\zeta_3^2 - \frac{1}{75}\pi^4\zeta_3 - 7\zeta_5 + \frac{797\zeta_7}{80} + \frac{5\pi^6}{378} \right) \\
& + \delta_{ch} \delta_{dg} \lambda_{b\alpha\beta a} \lambda_{iklf} \lambda_{j\alpha\beta e} \left( \frac{5\zeta_3^2}{4} + \frac{3\zeta_3}{20} - \frac{3\zeta_5}{20} - \frac{\pi^6}{3780} + \frac{\pi^4}{400} \right) \\
& + \delta_{bg} \delta_{ch} \lambda_{d\alpha\beta a} \lambda_{iklf} \lambda_{j\alpha\beta e} \left( \frac{2\zeta_3}{5} - \frac{3\zeta_5}{10} - \frac{2}{5} \right) \\
& + \delta_{cg} \lambda_{bdla} \lambda_{hj\alpha e} \lambda_{ik\alpha f} \left( -\frac{9}{5}\zeta_3^2 + \frac{3}{50}\pi^4\zeta_3 - \frac{189\zeta_7}{10} \right) \\
& + \delta_{bg} \delta_{ch} \lambda_{dl\beta a} \lambda_{ik\alpha f} \lambda_{j\alpha\beta e} \left( \frac{7\zeta_3^2}{10} - \frac{7}{600}\pi^4\zeta_3 + \frac{11\zeta_5}{2} + \frac{127\zeta_7}{40} - \frac{\pi^6}{756} \right) \\
& + \delta_{ck} \delta_{dg} \lambda_{b\alpha\beta a} \lambda_{hj\alpha e} \lambda_{il\beta f} \left( \frac{3}{50}\pi^4\zeta_3 - 9\zeta_3^2 \right) \\
& + \delta_{bj} \delta_{cg} \lambda_{d\alpha\beta a} \lambda_{hk\alpha e} \lambda_{il\beta f} \left( -\frac{216\zeta_{35}}{5} - 126\zeta_3\zeta_5 + \frac{29\pi^8}{2625} \right) \\
& + \delta_{ch} \delta_{dg} \lambda_{b\alpha\beta a} \lambda_{il\beta f} \lambda_{jk\alpha e} \left( 2\zeta_3^2 - \frac{1}{75}\pi^4\zeta_3 - 7\zeta_5 + \frac{797\zeta_7}{80} + \frac{5\pi^6}{378} \right) \\
& + \delta_{bg} \delta_{ch} \lambda_{d\alpha\beta a} \lambda_{il\beta f} \lambda_{jk\alpha e} \left( \frac{11\zeta_3^2}{20} + \frac{33\zeta_3}{10} + \frac{21\zeta_5}{10} + \frac{\pi^6}{3780} - \frac{\pi^4}{100} \right) \\
& + \delta_{bj} \delta_{ck} \delta_{dg} \lambda_{\alpha\beta\gamma a} \lambda_{h\alpha\beta e} \lambda_{il\gamma f} \left( \frac{39\zeta_3^2}{40} + \frac{33\zeta_3}{20} + \frac{21\zeta_5}{20} - \frac{\pi^6}{840} - \frac{\pi^4}{200} \right) \\
& + \delta_{bk} \delta_{cg} \delta_{dj} \lambda_{\alpha\beta\gamma a} \lambda_{h\alpha\beta e} \lambda_{il\gamma f} \left( -\frac{81\zeta_{35}}{25} + 54\zeta_3\zeta_5 - \frac{3087\zeta_7}{40} + \frac{2063\pi^8}{420000} \right) \\
& + \delta_{bk} \delta_{cg} \delta_{dj} \lambda_{h\alpha\beta e} \lambda_{i\alpha\gamma f} \lambda_{l\beta\gamma a} (-60\zeta_3\zeta_5)
\end{aligned}$$

$$\begin{aligned}
& + \delta_{ch} \delta_{dg} \delta_{il} \lambda_{\alpha\beta\gamma e} \lambda_{b\beta\gamma a} \lambda_{jk\alpha f} \left( \frac{5\zeta_3^2}{4} + \frac{3\zeta_3}{20} - \frac{3\zeta_5}{20} - \frac{\pi^6}{3780} + \frac{\pi^4}{400} \right) \\
& + \delta_{cg} \delta_{hk} \delta_{il} \lambda_{\alpha\beta\gamma e} \lambda_{bd\gamma a} \lambda_{j\alpha\beta f} \left( \frac{27\zeta_3}{20} + \frac{15\zeta_5}{8} - \frac{7\pi^4}{1200} - \frac{221}{120} \right) \\
& + \delta_{ch} \delta_{dg} \delta_{il} \lambda_{\alpha\beta\gamma e} \lambda_{bk\gamma a} \lambda_{j\alpha\beta f} \left( \frac{43\zeta_3^2}{20} - \frac{3\zeta_3}{10} + \frac{47\zeta_5}{10} - \frac{4\pi^6}{945} + \frac{\pi^4}{25} \right) \\
& + \delta_{bg} \delta_{ch} \delta_{il} \lambda_{\alpha\beta\gamma e} \lambda_{dk\gamma a} \lambda_{j\alpha\beta f} \left( -\frac{12\zeta_3}{5} - \frac{17\zeta_5}{10} - \frac{\pi^4}{300} + \frac{227}{30} \right) \\
& + \delta_{ch} \delta_{dg} \lambda_{bi\beta a} \lambda_{j\alpha\beta e} \lambda_{kl\alpha f} \left( -\frac{13}{10} \right) \\
& + \delta_{bh} \delta_{ci} \delta_{dg} \lambda_{\alpha\beta\gamma a} \lambda_{j\alpha\beta e} \lambda_{kl\gamma f} \left( -\frac{\zeta_3}{10} - \frac{31\zeta_5}{20} - \frac{\pi^4}{300} + \frac{17}{20} \right) \\
& + \delta_{cg} \delta_{il} \lambda_{bdha} \lambda_{j\alpha\beta e} \lambda_{k\alpha\beta f} \left( -\frac{3\zeta_3}{2} - \frac{3\zeta_5}{2} + \frac{17}{15} \right) \\
& + \delta_{ch} \delta_{dg} \delta_{il} \lambda_{b\beta\gamma a} \lambda_{j\alpha\beta e} \lambda_{k\alpha\gamma f} \left( -\frac{9}{5}\zeta_3^2 + \frac{3}{50}\pi^4\zeta_3 - \frac{189\zeta_7}{10} \right) \\
& + \delta_{bg} \delta_{ch} \delta_{il} \lambda_{d\beta\gamma a} \lambda_{j\alpha\beta e} \lambda_{k\alpha\gamma f} \left( \frac{81\zeta_3^2}{20} + 5\zeta_3 - \frac{23\zeta_5}{10} - \frac{\pi^6}{315} + \frac{\pi^4}{40} \right) \\
& + \delta_{ck} \delta_{dg} \lambda_{bhia} \lambda_{j\alpha\beta e} \lambda_{l\alpha\beta f} \left( \frac{\zeta_3}{40} - \frac{53\zeta_5}{80} - \frac{\pi^4}{400} + \frac{163}{240} \right) \\
& + \delta_{bk} \delta_{cg} \delta_{dj} \delta_{il} \lambda_{\alpha\beta\delta f} \lambda_{\alpha\beta\gamma e} \lambda_{h\gamma\delta a} \left( -\frac{141}{20}\zeta_3^2 + \frac{9\zeta_3}{5} - \frac{14\zeta_5}{5} + \frac{\pi^6}{1260} + \frac{13\pi^4}{600} \right) \\
& + \delta_{ce} \lambda_{bd\alpha a} \lambda_{hilf} \lambda_{jk\alpha g} \left( \frac{1}{60} \right) \\
& + \delta_{ce} \delta_{il} \lambda_{dhkb} \lambda_{f\alpha\beta a} \lambda_{j\alpha\beta g} \left( \frac{3}{100}\pi^4\zeta_3 - \frac{9\zeta_3^2}{2} \right) \\
& + \delta_{ce} \delta_{il} \lambda_{bd\beta a} \lambda_{hk\alpha f} \lambda_{j\alpha\beta g} \left( -\frac{3}{20}\zeta_3^2 + \frac{21\zeta_3}{5} + \frac{21\zeta_5}{10} - \frac{\pi^6}{1260} - \frac{19\pi^4}{600} \right) \\
& + \delta_{ce} \delta_{il} \lambda_{bdka} \lambda_{h\alpha\beta f} \lambda_{j\alpha\beta g} \left( \frac{16\zeta_3}{5} + \frac{17\zeta_5}{10} - \frac{\pi^4}{100} - \frac{13}{10} \right) \\
& + \delta_{ce} \delta_{hk} \delta_{il} \lambda_{\alpha\beta\gamma f} \lambda_{\alpha\beta\gamma g} \lambda_{bdja} \left( -\frac{7\zeta_3}{120} + \frac{\pi^4}{3600} - \frac{81}{5120} \right) \\
& + \delta_{cg} \lambda_{bd\alpha a} \lambda_{fkle} \lambda_{ij\alpha h} \left( \frac{3\zeta_3}{40} - \frac{\pi^4}{800} - \frac{11}{80} \right) \\
& + \delta_{ck} \delta_{dg} \lambda_{b\alpha\beta a} \lambda_{fl\beta e} \lambda_{ij\alpha h} \left( \frac{27\zeta_3^2}{40} + \frac{3\zeta_3}{40} + \frac{27\zeta_5}{40} - \frac{\pi^6}{1260} + \frac{\pi^4}{800} \right) \\
& + \delta_{cg} \lambda_{bdfa} \lambda_{ij\alpha h} \lambda_{kl\alpha e} \left( \frac{\zeta_3}{20} + \frac{9\zeta_5}{80} - \frac{\pi^4}{200} + \frac{23}{80} \right) \\
& + \delta_{ck} \delta_{dg} \lambda_{b\alpha\beta a} \lambda_{fjle} \lambda_{i\alpha\beta h} \left( -\frac{\zeta_3}{16} + \frac{3\zeta_5}{16} - \frac{\pi^4}{960} - \frac{1}{32} \right) \\
& + \delta_{cg} \lambda_{bd\alpha a} \lambda_{file} \lambda_{jk\alpha h} \left( \frac{\zeta_3^2}{2} + \frac{3\zeta_3}{20} + \frac{21\zeta_5}{10} - \frac{17\pi^6}{7560} + \frac{\pi^4}{400} \right) \\
& + \delta_{cg} \lambda_{bdla} \lambda_{fia e} \lambda_{jk\alpha h} \left( -\frac{21}{40}\zeta_3^2 + \frac{3\zeta_3}{40} + \frac{27\zeta_5}{40} - \frac{\pi^6}{1260} + \frac{\pi^4}{800} \right) \\
& + \delta_{cg} \lambda_{bdia} \lambda_{fl\alpha e} \lambda_{jk\alpha h} \left( \frac{\zeta_3}{20} - \frac{3\zeta_5}{20} - \frac{\pi^4}{240} + \frac{1}{2} \right) \\
& + \delta_{cg} \delta_{il} \lambda_{bd\beta a} \lambda_{f\alpha\beta e} \lambda_{jk\alpha h} \left( \frac{\zeta_3}{20} - \frac{3\zeta_5}{20} - \frac{\pi^4}{240} + \frac{1}{2} \right) \\
& + \delta_{cg} \lambda_{bdfa} \lambda_{il\alpha e} \lambda_{jk\alpha h} \left( \frac{33\zeta_3}{20} + \frac{7\zeta_5}{40} - \frac{\pi^4}{240} - \frac{221}{120} \right) \\
& + \delta_{ck} \delta_{dg} \lambda_{bf\beta a} \lambda_{i\alpha\beta e} \lambda_{jl\alpha h} \left( -\frac{1}{2}\zeta_3^2 + \frac{1}{300}\pi^4\zeta_3 - \frac{7\zeta_5}{2} - \frac{359\zeta_7}{40} + \frac{5\pi^6}{756} \right)
\end{aligned}$$

$$\begin{aligned}
& + \delta_{cg} \delta_{il} \lambda_{bd\beta a} \lambda_{fk\alpha e} \lambda_{j\alpha\beta h} \left( -\zeta_3^2 + \frac{1}{150} \pi^4 \zeta_3 - 7\zeta_5 + \frac{61\zeta_7}{20} + \frac{5\pi^6}{378} \right) \\
& + \delta_{ck} \delta_{dg} \lambda_{bi\beta a} \lambda_{fl\alpha e} \lambda_{j\alpha\beta h} \left( -\frac{1}{2} \zeta_3^2 + \frac{1}{300} \pi^4 \zeta_3 - \frac{7\zeta_5}{2} + \frac{201\zeta_7}{40} + \frac{5\pi^6}{756} \right) \\
& + \delta_{cg} \delta_{il} \lambda_{bdka} \lambda_{f\alpha\beta e} \lambda_{j\alpha\beta h} \left( \frac{5\zeta_3^2}{4} + \frac{3\zeta_3}{20} - \frac{3\zeta_5}{20} - \frac{\pi^6}{3780} + \frac{\pi^4}{400} \right) \\
& + \delta_{ck} \delta_{dg} \lambda_{bf\beta a} \lambda_{il\alpha e} \lambda_{j\alpha\beta h} \left( -\frac{81\zeta_{35}}{25} - 9\zeta_3\zeta_5 - \frac{3087\zeta_7}{40} + \frac{2063\pi^8}{420000} \right) \\
& + \delta_{cg} \delta_{il} \lambda_{bdfa} \lambda_{j\alpha\beta h} \lambda_{k\alpha\beta e} \left( \frac{27\zeta_3}{20} + \frac{15\zeta_5}{8} - \frac{7\pi^4}{1200} - \frac{221}{120} \right) \\
& + \delta_{ck} \delta_{dg} \lambda_{bfia} \lambda_{j\alpha\beta h} \lambda_{l\alpha\beta e} \left( \frac{27\zeta_3^2}{8} - \frac{3\zeta_3}{20} - \frac{33\zeta_5}{20} - \frac{\pi^6}{1260} + \frac{\pi^4}{50} \right) \\
& + \delta_{bj} \delta_{cg} \lambda_{d\alpha\beta a} \lambda_{file} \lambda_{k\alpha\beta h} \left( \frac{11\zeta_3^2}{2} - \frac{11}{300} \pi^4 \zeta_3 - \frac{7\zeta_5}{2} - \frac{5\zeta_7}{2} + \frac{5\pi^6}{756} \right) \\
& + \delta_{bj} \delta_{cg} \lambda_{dl\beta a} \lambda_{fi\alpha e} \lambda_{k\alpha\beta h} \left( -\frac{81\zeta_{35}}{25} + 9\zeta_3\zeta_5 - \frac{3087\zeta_7}{40} + \frac{2063\pi^8}{420000} \right) \\
& + \delta_{bj} \delta_{cg} \lambda_{dila} \lambda_{f\alpha\beta e} \lambda_{k\alpha\beta h} \left( \frac{5\zeta_3^2}{2} - \frac{1}{60} \pi^4 \zeta_3 - \frac{7\zeta_5}{2} - \frac{19\zeta_7}{2} + \frac{5\pi^6}{756} \right) \\
& + \delta_{bj} \delta_{cg} \delta_{il} \lambda_{d\beta\gamma a} \lambda_{f\alpha\gamma e} \lambda_{k\alpha\beta h} \left( \frac{3\zeta_3^2}{20} - \frac{102\zeta_3}{5} - \frac{21\zeta_5}{5} + \frac{\pi^6}{1260} + \frac{43\pi^4}{600} \right) \\
& + \delta_{bj} \delta_{cg} \lambda_{df\beta a} \lambda_{il\alpha e} \lambda_{k\alpha\beta h} \left( -\frac{108}{5} \zeta_3^2 + \frac{3}{25} \pi^4 \zeta_3 + \frac{189\zeta_7}{20} \right) \\
& + \delta_{bj} \delta_{cg} \lambda_{dfia} \lambda_{i\alpha\beta e} \lambda_{k\alpha\beta h} \left( -\frac{77}{20} \zeta_3^2 - \frac{3\zeta_3}{10} + \frac{47\zeta_5}{10} - \frac{4\pi^6}{945} + \frac{\pi^4}{25} \right) \\
& + \delta_{cj} \delta_{dg} \delta_{fi} \lambda_{b\beta\gamma a} \lambda_{k\alpha\beta h} \lambda_{l\alpha\gamma e} \left( \frac{9\zeta_3^2}{40} + \frac{33\zeta_3}{20} + \frac{21\zeta_5}{20} + \frac{\pi^6}{1260} - \frac{\pi^4}{200} \right) \\
& + \delta_{bj} \delta_{cg} \delta_{il} \lambda_{\alpha\beta\gamma e} \lambda_{df\gamma a} \lambda_{k\alpha\beta h} \left( -\frac{39}{40} \zeta_3^2 - \frac{3\zeta_3}{20} - \frac{63\zeta_5}{20} + \frac{\pi^6}{840} + \frac{\pi^4}{50} \right) \\
& + \delta_{bj} \delta_{ck} \delta_{dg} \lambda_{f\beta\gamma a} \lambda_{i\alpha\gamma e} \lambda_{l\alpha\beta h} \left( \frac{\zeta_3^2}{5} - \frac{1}{300} \pi^4 \zeta_3 + 11\zeta_5 + \frac{359\zeta_7}{40} - \frac{\pi^6}{378} \right) \\
& + \delta_{bk} \delta_{cg} \delta_{dj} \lambda_{f\beta\gamma a} \lambda_{i\alpha\gamma e} \lambda_{l\alpha\beta h} \left( -8\zeta_3^3 - \frac{1063\zeta_9}{9} \right) \\
& + \delta_{bj} \delta_{cg} \delta_{il} \lambda_{\alpha\beta\gamma h} \lambda_{dk\gamma a} \lambda_{f\alpha\beta e} \left( -\frac{57}{20} \zeta_3^2 - \frac{23\zeta_3}{20} - \frac{49\zeta_5}{20} + \frac{\pi^6}{1260} + \frac{7\pi^4}{400} \right) \\
& + \delta_{bj} \delta_{ck} \delta_{dg} \lambda_{\alpha\beta\gamma h} \lambda_{f\beta\gamma a} \lambda_{il\alpha e} \left( \frac{17\zeta_3^2}{20} + \frac{33\zeta_3}{10} + \frac{21\zeta_5}{10} - \frac{\pi^6}{270} - \frac{\pi^4}{100} \right) \\
& + \delta_{bk} \delta_{cg} \delta_{dj} \lambda_{\alpha\beta\gamma h} \lambda_{f\beta\gamma a} \lambda_{il\alpha e} \left( -\frac{81\zeta_{35}}{25} + 45\zeta_3\zeta_5 - \frac{3087\zeta_7}{40} + \frac{2063\pi^8}{420000} \right) \\
& + \delta_{bk} \delta_{cg} \delta_{dj} \lambda_{\alpha\beta\gamma h} \lambda_{fl\gamma a} \lambda_{i\alpha\beta e} \left( -2\zeta_3^2 + \frac{1}{150} \pi^4 \zeta_3 - 62\zeta_5 + \frac{761\zeta_7}{20} + \frac{5\pi^6}{189} \right) \\
& + \delta_{cj} \delta_{dg} \delta_{fi} \lambda_{\alpha\beta\gamma h} \lambda_{b\beta\gamma a} \lambda_{kl\alpha e} \left( \frac{\zeta_3}{5} - \frac{9\zeta_5}{80} + \frac{\pi^4}{1200} + \frac{1}{16} \right) \\
& + \delta_{bj} \delta_{ck} \delta_{dg} \delta_{fi} \lambda_{\alpha\beta\gamma h} \lambda_{\beta\gamma\delta a} \lambda_{l\alpha\delta e} \left( -\frac{7\zeta_3}{40} - \frac{3\zeta_5}{40} - \frac{\pi^4}{2400} - \frac{1}{5} \right) \\
& + \delta_{bj} \delta_{cg} \delta_{il} \lambda_{\alpha\beta\gamma e} \lambda_{\alpha\beta\gamma h} \lambda_{dfka} \left( \frac{9\zeta_3}{160} + \frac{21\zeta_5}{80} - \frac{7\pi^4}{2400} \right) \\
& + \delta_{bk} \delta_{cg} \delta_{dj} \lambda_{\alpha\beta\gamma e} \lambda_{\alpha\beta\gamma h} \lambda_{fila} \left( \frac{\zeta_3^2}{12} + \frac{25\zeta_5}{6} - \frac{5\pi^6}{4536} \right) \\
& + \delta_{ak} \delta_{bl} \delta_{cg} \delta_{dj} \lambda_{\alpha\beta\delta e} \lambda_{\alpha\beta\gamma h} \lambda_{i\gamma\delta f} \left( \frac{12\zeta_3}{5} + \frac{23\zeta_5}{10} + \frac{\pi^4}{600} - \frac{239}{60} \right) \\
& + \delta_{bg} \delta_{ch} \lambda_{d\alpha\beta a} \lambda_{fl\beta e} \lambda_{jk\alpha i} \left( \frac{17\zeta_3}{20} + \frac{3\zeta_5}{20} + \frac{\pi^4}{400} - \frac{2}{5} \right)
\end{aligned}$$

$$\begin{aligned}
& + \delta_{bg} \delta_{ch} \lambda_{dl\beta a} \lambda_{f\alpha\beta e} \lambda_{jk\alpha i} \left( -\frac{2}{5} \right) \\
& + \delta_{ch} \delta_{dg} \lambda_{bf\beta a} \lambda_{jk\alpha i} \lambda_{l\alpha\beta e} \left( -\frac{11}{20} \zeta_3^2 - \frac{3\zeta_3}{10} + \frac{17\zeta_5}{10} - \frac{\pi^6}{3780} + \frac{\pi^4}{25} \right) \\
& + \delta_{bg} \delta_{ch} \lambda_{df\beta a} \lambda_{jk\alpha i} \lambda_{l\alpha\beta e} \left( \frac{\zeta_3}{40} - \frac{3\zeta_5}{40} - \frac{\pi^4}{480} + \frac{1}{4} \right) \\
& + \delta_{ch} \delta_{dg} \delta_{fl} \lambda_{\alpha\beta\gamma e} \lambda_{b\beta\gamma a} \lambda_{jk\alpha i} \left( \frac{27\zeta_3^2}{20} + \frac{3\zeta_3}{20} + \frac{27\zeta_5}{20} - \frac{\pi^6}{630} + \frac{\pi^4}{400} \right) \\
& + \delta_{bg} \delta_{ch} \lambda_{d\alpha\beta a} \lambda_{fkle} \lambda_{j\alpha\beta i} \left( -\frac{13\zeta_3}{80} - \frac{7\zeta_5}{160} + \frac{\pi^4}{4800} + \frac{3}{32} \right) \\
& + \delta_{bg} \delta_{ch} \lambda_{dkla} \lambda_{f\alpha\beta e} \lambda_{j\alpha\beta i} \left( -\frac{3\zeta_3}{20} - \frac{21\zeta_5}{80} + \frac{1}{16} \right) \\
& + \delta_{ch} \delta_{dg} \lambda_{bf\beta a} \lambda_{j\alpha\beta i} \lambda_{kl\alpha e} \left( -\frac{9}{20} \zeta_3^2 - \frac{3\zeta_3}{10} + \frac{57\zeta_5}{10} - \frac{\pi^6}{630} + \frac{\pi^4}{25} \right) \\
& + \delta_{ch} \delta_{dg} \delta_{fl} \lambda_{b\beta\gamma a} \lambda_{j\alpha\beta i} \lambda_{k\alpha\gamma e} \left( -\frac{81\zeta_{35}}{25} - 9\zeta_3\zeta_5 - \frac{3087\zeta_7}{40} + \frac{2063\pi^8}{420000} \right) \\
& + \delta_{ch} \delta_{dg} \delta_{fl} \lambda_{\alpha\beta\gamma e} \lambda_{bk\gamma a} \lambda_{j\alpha\beta i} \left( 8\zeta_3^2 - \frac{4}{75} \pi^4 \zeta_3 - 7\zeta_5 + \frac{377\zeta_7}{80} + \frac{5\pi^6}{378} \right) \\
& + \delta_{bj} \delta_{ch} \delta_{dg} \delta_{fl} \lambda_{\alpha\gamma\delta e} \lambda_{\beta\gamma\delta a} \lambda_{k\alpha\beta i} \left( \frac{17\zeta_3^2}{2} - \frac{17}{600} \pi^4 \zeta_3 - \frac{31\zeta_5}{2} - \frac{17\zeta_7}{8} + \frac{5\pi^6}{756} \right) \\
& + \delta_{ak} \delta_{bg} \delta_{ch} \delta_{dj} \lambda_{\alpha\gamma\delta e} \lambda_{\beta\gamma\delta f} \lambda_{l\alpha\beta i} \left( \frac{12\zeta_3}{5} + \frac{3\zeta_5}{2} + \frac{\pi^4}{200} - \frac{79}{30} \right) \\
& + \delta_{ch} \delta_{dg} \delta_{fl} \lambda_{\alpha\beta\gamma i} \lambda_{b\beta\gamma a} \lambda_{jk\alpha e} \left( -\frac{3\zeta_3}{4} - \frac{7\zeta_5}{40} + \frac{\pi^4}{600} + \frac{1}{60} \right) \\
& + \delta_{ch} \delta_{dg} \delta_{fl} \lambda_{\alpha\beta\gamma i} \lambda_{bk\gamma a} \lambda_{j\alpha\beta e} \left( 5\zeta_3^2 - \frac{1}{30} \pi^4 \zeta_3 - 7\zeta_5 + \frac{117\zeta_7}{20} + \frac{5\pi^6}{378} \right) \\
& + \delta_{ch} \delta_{dg} \delta_{fl} \lambda_{\alpha\beta\gamma e} \lambda_{\alpha\beta\gamma i} \lambda_{bjka} \left( -\frac{5\zeta_3}{48} + \frac{\pi^4}{5760} + \frac{553}{5120} \right) \\
& + \delta_{ak} \delta_{bg} \delta_{ch} \delta_{dj} \lambda_{\alpha\beta\delta e} \lambda_{\alpha\beta\gamma i} \lambda_{l\gamma\delta f} \left( -\frac{27\zeta_3}{5} + \frac{32\zeta_5}{5} - \frac{7\pi^4}{300} + \frac{227}{30} \right) \\
& + \delta_{ak} \delta_{bl} \delta_{cg} \delta_{dj} \lambda_{\alpha\beta\delta i} \lambda_{\alpha\beta\gamma h} \lambda_{f\gamma\delta e} \left( \frac{\zeta_3}{20} - \frac{53\zeta_5}{40} - \frac{\pi^4}{200} + \frac{163}{120} \right) \\
& + \delta_{cg} \delta_{il} \lambda_{bd\beta a} \lambda_{fh\alpha e} \lambda_{k\alpha\beta j} \left( \frac{\zeta_3^2}{2} + \frac{3\zeta_3}{20} + \frac{21\zeta_5}{10} - \frac{17\pi^6}{7560} + \frac{\pi^4}{400} \right) \\
& + \delta_{cg} \delta_{il} \lambda_{bdha} \lambda_{f\alpha\beta e} \lambda_{k\alpha\beta j} \left( \frac{\zeta_3}{20} + \frac{9\zeta_5}{80} - \frac{\pi^4}{200} + \frac{23}{80} \right) \\
& + \delta_{ch} \delta_{dg} \delta_{il} \lambda_{b\beta\gamma a} \lambda_{f\alpha\gamma e} \lambda_{k\alpha\beta j} \left( -\frac{7}{40} \zeta_3^2 + \frac{\zeta_3}{40} + \frac{9\zeta_5}{40} - \frac{\pi^6}{3780} + \frac{\pi^4}{2400} \right) \\
& + \delta_{bg} \delta_{ch} \delta_{il} \lambda_{d\beta\gamma a} \lambda_{f\alpha\gamma e} \lambda_{k\alpha\beta j} \left( \frac{33\zeta_3}{20} + \frac{7\zeta_5}{40} - \frac{\pi^4}{240} - \frac{221}{120} \right) \\
& + \delta_{cg} \delta_{il} \lambda_{bdfa} \lambda_{h\alpha\beta e} \lambda_{k\alpha\beta j} \left( \frac{3\zeta_3}{20} - \frac{\pi^4}{400} - \frac{11}{40} \right) \\
& + \delta_{ch} \delta_{dg} \lambda_{bf\beta a} \lambda_{il\alpha e} \lambda_{k\alpha\beta j} \left( -\frac{11}{20} \zeta_3^2 - \frac{3\zeta_3}{10} + \frac{17\zeta_5}{10} - \frac{\pi^6}{3780} + \frac{\pi^4}{25} \right) \\
& + \delta_{ch} \delta_{dg} \delta_{fl} \lambda_{b\beta\gamma a} \lambda_{i\alpha\gamma e} \lambda_{k\alpha\beta j} \left( -\frac{1}{2} \zeta_3^2 + \frac{1}{300} \pi^4 \zeta_3 - \frac{7\zeta_5}{2} + \frac{201\zeta_7}{40} + \frac{5\pi^6}{756} \right) \\
& + \delta_{bh} \delta_{ci} \delta_{dg} \lambda_{f\beta\gamma a} \lambda_{k\alpha\beta j} \lambda_{l\alpha\gamma e} \left( \frac{227}{30} \right) \\
& + \delta_{bg} \delta_{ch} \delta_{il} \lambda_{\alpha\beta\gamma e} \lambda_{df\gamma a} \lambda_{k\alpha\beta j} \left( \frac{\zeta_3}{20} + \frac{9\zeta_5}{80} - \frac{\pi^4}{200} + \frac{23}{80} \right) \\
& + \delta_{ce} \delta_{il} \lambda_{bd\beta a} \lambda_{gh\alpha f} \lambda_{k\alpha\beta j} \left( -\frac{3\zeta_3}{4} - \frac{7\zeta_5}{40} + \frac{\pi^4}{600} + \frac{1}{60} \right)
\end{aligned}$$

$$\begin{aligned}
& + \delta_{ce} \delta_{il} \lambda_{bdha} \lambda_{g\alpha\beta f} \lambda_{k\alpha\beta j} \left( -\frac{3\zeta_3}{4} - \frac{7\zeta_5}{40} + \frac{\pi^4}{600} + \frac{1}{60} \right) \\
& + \delta_{bg} \delta_{ch} \delta_{il} \lambda_{\alpha\beta\gamma j} \lambda_{d\beta\gamma a} \lambda_{fk\alpha e} \left( -\frac{19\zeta_3}{20} + \frac{7\zeta_5}{8} - \frac{\pi^4}{150} + \frac{17}{20} \right) \\
& + \delta_{cg} \delta_{hk} \delta_{il} \lambda_{\alpha\beta\gamma j} \lambda_{bd\gamma a} \lambda_{f\alpha\beta e} \left( \frac{3\zeta_3}{20} - \frac{\pi^4}{400} - \frac{11}{40} \right) \\
& + \delta_{bg} \delta_{ch} \delta_{il} \lambda_{\alpha\beta\gamma j} \lambda_{dk\gamma a} \lambda_{f\alpha\beta e} \left( \frac{19\zeta_3}{20} + \frac{7\zeta_5}{40} + \frac{\pi^4}{600} + \frac{17}{20} \right) \\
& + \delta_{ch} \delta_{dg} \delta_{fl} \lambda_{\alpha\beta\gamma j} \lambda_{b\beta\gamma a} \lambda_{ik\alpha e} \left( -\zeta_3^2 + \frac{1}{150} \pi^4 \zeta_3 - 7\zeta_5 - \frac{359\zeta_7}{20} + \frac{5\pi^6}{378} \right) \\
& + \delta_{ch} \delta_{dg} \delta_{fl} \lambda_{\alpha\beta\gamma j} \lambda_{bk\gamma a} \lambda_{i\alpha\beta e} \left( 5\zeta_3^2 - \frac{1}{30} \pi^4 \zeta_3 - 7\zeta_5 - \frac{23\zeta_7}{20} + \frac{5\pi^6}{378} \right) \\
& + \delta_{bh} \delta_{ci} \delta_{dg} \lambda_{\alpha\beta\gamma j} \lambda_{f\beta\gamma a} \lambda_{kl\alpha e} \left( \frac{17\zeta_3}{20} + \frac{3\zeta_5}{20} + \frac{\pi^4}{400} - \frac{2}{5} \right) \\
& + \delta_{ch} \delta_{dg} \delta_{fl} \lambda_{\alpha\beta\gamma j} \lambda_{bi\gamma a} \lambda_{k\alpha\beta e} \left( \frac{16\zeta_3}{5} + \frac{17\zeta_5}{10} - \frac{\pi^4}{100} - \frac{13}{10} \right) \\
& + \delta_{bg} \delta_{ch} \delta_{il} \lambda_{\alpha\beta\gamma j} \lambda_{df\gamma a} \lambda_{k\alpha\beta e} \left( \frac{19\zeta_3}{20} - \frac{7\zeta_5}{20} - \frac{\pi^4}{1200} - \frac{19}{20} \right) \\
& + \delta_{cg} \delta_{hk} \delta_{il} \lambda_{\alpha\beta\gamma e} \lambda_{\alpha\beta\gamma j} \lambda_{bdfa} \left( -\frac{\zeta_3}{40} + \frac{17\pi^4}{28800} - \frac{661}{15360} \right) \\
& + \delta_{ch} \delta_{dg} \delta_{il} \lambda_{\alpha\beta\gamma e} \lambda_{\alpha\beta\gamma j} \lambda_{bfka} \left( \frac{9\zeta_3}{160} - \frac{29\zeta_5}{80} - \frac{7\pi^4}{2400} \right) \\
& + \delta_{ch} \delta_{dg} \delta_{fl} \lambda_{\alpha\beta\gamma e} \lambda_{\alpha\beta\gamma j} \lambda_{bika} \left( \frac{4267}{23040} \right) \\
& + \delta_{bg} \delta_{ch} \delta_{il} \lambda_{\alpha\beta\gamma e} \lambda_{\alpha\beta\gamma j} \lambda_{dfka} \left( -\frac{3\zeta_3}{40} - \frac{\pi^4}{3600} + \frac{249}{5120} \right) \\
& + \delta_{ch} \delta_{dg} \delta_{fl} \delta_{ik} \lambda_{\alpha\beta\delta e} \lambda_{\alpha\beta\gamma j} \lambda_{b\gamma\delta a} \left( \frac{27\zeta_3^2}{8} - \frac{3\zeta_3}{20} - \frac{33\zeta_5}{20} - \frac{\pi^6}{1260} + \frac{\pi^4}{50} \right) \\
& + \delta_{ce} \delta_{hk} \delta_{il} \lambda_{\alpha\beta\gamma j} \lambda_{bd\gamma a} \lambda_{g\alpha\beta f} \left( -\frac{29}{60} \right) \\
& + \delta_{ch} \delta_{dg} \delta_{fl} \lambda_{\alpha\beta\gamma j} \lambda_{be\gamma a} \lambda_{k\alpha\beta i} \left( -\frac{15}{4} \zeta_3^2 - \frac{3\zeta_3}{10} + \frac{87\zeta_5}{10} - \frac{\pi^6}{180} + \frac{\pi^4}{25} \right) \\
& + \delta_{ch} \delta_{dg} \delta_{fl} \lambda_{\alpha\beta\gamma i} \lambda_{\alpha\beta\gamma j} \lambda_{beka} \left( \frac{9\zeta_3}{80} - \frac{37\zeta_5}{120} - \frac{7\pi^4}{1200} \right) \\
& + \delta_{bj} \delta_{cg} \delta_{il} \lambda_{\alpha\beta\gamma k} \lambda_{d\beta\gamma a} \lambda_{fh\alpha e} \left( -\frac{23\zeta_3}{10} + \frac{28\zeta_5}{5} - \frac{\pi^6}{420} + \frac{7\pi^4}{200} \right) \\
& + \delta_{bj} \delta_{ch} \delta_{dg} \delta_{fl} \lambda_{\alpha\beta\gamma k} \lambda_{\beta\gamma\delta a} \lambda_{i\alpha\delta e} \left( 11\zeta_3^2 - \frac{11}{300} \pi^4 \zeta_3 - 31\zeta_5 + \frac{243\zeta_7}{40} + \frac{5\pi^6}{378} \right) \\
& + \delta_{cj} \delta_{dg} \delta_{fi} \lambda_{\alpha\beta\gamma k} \lambda_{bh\gamma a} \lambda_{l\alpha\beta e} \left( -\frac{\zeta_3}{4} + \frac{7\zeta_5}{20} - \frac{\pi^4}{400} - \frac{2}{5} \right) \\
& + \delta_{ak} \delta_{bg} \delta_{ch} \delta_{dj} \lambda_{\alpha\beta\delta e} \lambda_{\alpha\beta\gamma l} \lambda_{i\gamma\delta f} \left( \frac{3\zeta_3}{5} - \frac{83\zeta_5}{10} - \frac{\pi^4}{150} + \frac{227}{30} \right) \\
& + \delta_{ak} \delta_{bg} \delta_{ch} \delta_{dj} \lambda_{\alpha\beta\delta i} \lambda_{\alpha\beta\gamma l} \lambda_{f\gamma\delta e} \left( -\frac{\zeta_3}{4} + \frac{7\zeta_5}{20} - \frac{\pi^4}{400} - \frac{2}{5} \right) \\
& + \delta_{bk} \delta_{cg} \delta_{dj} \delta_{il} \lambda_{\beta\gamma\delta\alpha} \lambda_{f\gamma\delta a} \lambda_{h\alpha\beta e} \left( -\frac{123}{20} \zeta_3^2 - \frac{23\zeta_3}{20} + \frac{161\zeta_5}{20} - \frac{\pi^6}{315} + \frac{7\pi^4}{400} \right) \\
& + \delta_{bj} \delta_{ch} \delta_{dg} \delta_{fl} \lambda_{\beta\gamma\delta\alpha} \lambda_{\beta\gamma\delta\alpha} \lambda_{ik\alpha e} \left( -\frac{5}{12} \zeta_3^2 + \frac{25\zeta_5}{6} - \frac{5\pi^6}{4536} \right) \\
& + \delta_{bj} \delta_{ch} \delta_{dg} \delta_{fl} \lambda_{\beta\gamma\delta\alpha} \lambda_{i\alpha\beta e} \lambda_{k\gamma\delta a} \left( \frac{11\zeta_3^2}{4} - \frac{11}{600} \pi^4 \zeta_3 - \frac{7\zeta_5}{4} - \frac{317\zeta_7}{80} + \frac{5\pi^6}{1512} \right) \\
& + \delta_{ch} \delta_{dg} \delta_{fl} \delta_{ik} \lambda_{\beta\gamma\delta\alpha} \lambda_{b\gamma\delta a} \lambda_{j\alpha\beta e} \left( -\frac{3}{40} \zeta_3^2 + \frac{3\zeta_3}{40} - \frac{63\zeta_5}{40} + \frac{\pi^6}{840} + \frac{\pi^4}{800} \right)
\end{aligned}$$



$$\begin{aligned}
& + \delta_{bj} \delta_{ck} \delta_{dg} \delta_{fi} \lambda_{\beta\gamma\delta\alpha} \lambda_{h\gamma\delta\alpha} \lambda_{l\alpha\beta e} \left( -\frac{3\zeta_3}{80} - \frac{21\zeta_5}{160} + \frac{\pi^4}{1600} + \frac{9}{160} \right) \\
& + \delta_{ch} \delta_{dg} \delta_{fl} \delta_{ik} \lambda_{\alpha\beta\gamma e} \lambda_{\beta\gamma\delta\alpha} \lambda_{bj\delta a} \left( \frac{9\zeta_3}{80} - \frac{37\zeta_5}{120} - \frac{7\pi^4}{1200} \right) \\
& + \delta_{bk} \delta_{cg} \delta_{dj} \delta_{il} \lambda_{\alpha\beta\gamma e} \lambda_{\beta\gamma\delta\alpha} \lambda_{fh\delta a} \left( \frac{45\zeta_3}{16} + \frac{7\zeta_5}{24} - \frac{\pi^4}{120} \right) \\
& + \delta_{ak} \delta_{bg} \delta_{ch} \delta_{dj} \lambda_{\alpha\beta\gamma e} \lambda_{\beta\gamma\delta\alpha} \lambda_{il\delta f} \left( -\frac{7369}{7680} \right) \\
& + \delta_{ak} \delta_{bl} \delta_{cg} \delta_{dj} \lambda_{\beta\gamma\delta\alpha} \lambda_{h\alpha\beta e} \lambda_{i\gamma\delta f} \left( \frac{53\zeta_3}{80} + \frac{19\zeta_5}{20} + \frac{\pi^4}{1200} - \frac{241}{160} \right) \\
& + \delta_{ak} \delta_{bg} \delta_{ch} \delta_{dj} \lambda_{\beta\gamma\delta\alpha} \lambda_{i\gamma\delta f} \lambda_{l\alpha\beta e} \left( \frac{3\zeta_3}{4} - \frac{57\zeta_5}{40} - \frac{\pi^4}{200} + \frac{17}{20} \right) \\
& + \delta_{ak} \delta_{bl} \delta_{cg} \delta_{dj} \lambda_{\beta\gamma\delta\alpha} \lambda_{f\gamma\delta e} \lambda_{i\alpha\beta h} \left( -\frac{\zeta_3}{16} + \frac{3\zeta_5}{16} - \frac{\pi^4}{960} - \frac{1}{32} \right) \\
& + \delta_{ak} \delta_{bl} \delta_{cg} \delta_{dj} \lambda_{\alpha\beta\gamma h} \lambda_{\beta\gamma\delta\alpha} \lambda_{fi\delta e} \left( -\frac{5\zeta_3}{24} + \frac{\pi^4}{2880} + \frac{553}{2560} \right) \\
& + \delta_{ak} \delta_{bg} \delta_{ce} \delta_{dj} \delta_{il} \lambda_{\alpha\beta\epsilon h} \lambda_{\beta\gamma\delta\alpha} \lambda_{\gamma\delta\epsilon f} \left( \frac{141\zeta_3}{80} + \frac{7\zeta_5}{20} - \frac{\pi^4}{150} \right) \\
& + \delta_{bj} \delta_{ch} \delta_{dg} \delta_{fl} \lambda_{\beta\gamma\delta\alpha} \lambda_{e\gamma\delta a} \lambda_{k\alpha\beta i} \left( \frac{17\zeta_3^2}{8} - \frac{17\pi^4\zeta_3}{1200} - \frac{7\zeta_5}{8} - \frac{45\zeta_7}{16} + \frac{5\pi^6}{3024} \right) \\
& + \delta_{ak} \delta_{bg} \delta_{ch} \delta_{dj} \lambda_{\beta\gamma\delta\alpha} \lambda_{f\gamma\delta e} \lambda_{l\alpha\beta i} \left( \frac{\zeta_3}{5} - \frac{9\zeta_5}{80} + \frac{\pi^4}{1200} + \frac{1}{16} \right) \\
& + \delta_{ak} \delta_{bg} \delta_{ch} \delta_{dj} \lambda_{\alpha\beta\gamma i} \lambda_{\beta\gamma\delta\alpha} \lambda_{fl\delta e} \left( -\frac{7\zeta_3}{120} + \frac{\pi^4}{3600} - \frac{81}{5120} \right) \\
& + \delta_{aj} \delta_{bk} \delta_{ch} \delta_{dg} \delta_{fl} \lambda_{\alpha\beta\epsilon i} \lambda_{\beta\gamma\delta\alpha} \lambda_{\gamma\delta\epsilon e} \left( -\frac{3\zeta_3}{40} - \frac{\pi^4}{4800} - \frac{5509}{7680} \right) \\
& + \delta_{ak} \delta_{bg} \delta_{ch} \delta_{dj} \delta_{fl} \lambda_{\alpha\beta\epsilon i} \lambda_{\beta\gamma\delta\alpha} \lambda_{\gamma\delta\epsilon e} \left( -\frac{9\zeta_3}{80} + \frac{\pi^4}{1600} + \frac{1393}{7680} \right) \\
& + \delta_{ak} \delta_{bg} \delta_{ch} \delta_{dj} \lambda_{\alpha\beta\gamma l} \lambda_{\beta\gamma\delta\alpha} \lambda_{fi\delta e} \left( \frac{249}{5120} \right)
\end{aligned} \tag{23}$$
